# Supplementary material for: Probability-weighted ensembles of U.S. county-level climate projections for climate risk analysis
Source: arXiv:1510.00313 ancillary file (2015-10-05)
Supplement: Supplementary file 1 [file TP_Projections_appendix.pdf]

## APPENDIX A

## Supplementary Methods

*a. Concentration pathways*

We incorporate radiative forcing projections from all four representative concentration pathways (RCPs): RCP 2.6, RCP 4.5, RCP 6.0, and RCP 8.5 (Van Vuuren et al. 2011). Each RCP represents a greenhouse gas concentration pathway and does not necessarily reflect socio-economic and/or policy scenarios. However, a set of socio-economic projections, unaccompanied by climate policy, (the Shared Socioeconomic Pathways, or “SSP”) has recently been constructed, and the radiative forcings of these no-policy projections can be compared to those in the RCPs (O’Neill et al. 2013, 2014, 2015; Riahi 2013). The lowest emissions, ‘sustainable growth’ SSP (SSP 1) has radiative forcing comparable to RCP 6.0, while the highest SSP is comparable to or slightly higher than RCP 8.5, which can be interpreted as a high emissions, business-as-usual scenario. RCP 4.5 is consistent with moderate greenhouse gas emission reductions, and RCP 2.6 is a strong mitigation scenario. Notably, RCP 6.0 has the second lowest CO<sub>2</sub>-equivalent emissions total prior to 2050 (see Meinshausen et al. 2011, Fig. 3g). As a consequence, mean global temperature projections from RCP 6.0 do not exceed those of RCP 4.5 until the third quarter of the 21st century.

For each RCP, we used 600 MAGICC6 model runs. The 5th/17th/83rd/90th percentiles of equilibrium climate sensitivity for these 600 runs are 1.5°C/1.6°C/4.9°C/5.9°C per CO<sub>2</sub> doubling. From the MAGICC6 projections, the four RCPs yield *likely* (67% probability) global mean temperature increases in 2080–2099 above 1981–2010 levels of 0.5–1.4°C, 1.1–2.5°C, 1.5–3.0°C, and 2.6–4.9°C, respectively (Table A1).

Over the contiguous United States, the median change in 10-yr running annual average temperature for all RCPs is roughly equivalent between the equal-weighted CMIP5 ensemble and the SMME and MPCR methods (relative to 1981–2010). Despite greater CO<sub>2</sub>-equivalent emissions at the end of the century, RCP 6.0 is cooler than both RCP 4.5 and the strong mitigation scenario, RCP2.6, for much of the first half of the century due to lower CO<sub>2</sub>-equivalent emissions (Fig. A13).

*b. Daily climate projections*

## 1) GLOBAL CLIMATE MODEL OUTPUT

Although state-of-the-art GCMs can achieve resolutions of  $\sim 50 \text{ km} \times 50 \text{ km}$  (e.g., Delworth et al. 2012), GCM results from CMIP5 are calculated with horizontal resolutions too coarse (i.e., around 1 to 2 degrees)(see Flato et al. 2013, table 9.1) to attempt to characterize vulnerabilities and impacts at the county level. Additionally,

GCM projections contain systematic model biases that must be corrected before being employed to address climate impacts (Ho et al. 2011). In this study, projections of average temperature, minimum daily temperature, maximum daily temperature, and precipitation (all monthly averaged) were obtained from a BCSO archive derived from select CMIP5 models (Brekke et al. 2013). A detailed inventory of the models used in this study with each RCP is shown in Table A2. For the contiguous United States (CONUS), projections are disaggregated to  $1/8 \times 1/8$  degree ( $\sim 14 \text{ km}$ ) horizontal resolution, while  $1/2 \times 1/2$  degree ( $\sim 56 \text{ km}$ ) model output with global coverage over land only is used to provide projections for Alaska and Hawaii.

As with all climate downscaling techniques, providing climate variables at higher spatial and temporal resolution does not necessarily make projections any more reliable than raw results from the underlying GCM. More detail is not always indicative of superior information. Statistical downscaling techniques assume current relationships between local and large scale climate variables will remain in future climates, which may or may not be strictly true. Investigators should ideally employ multiple statistical downscaling methodologies to gauge uncertainties associated with the their method. Various approaches are given in the literature (e.g., Stoner et al. 2013; Mahmood and Babel 2013; McGinnis et al. 2015).

Starting with the BCSO model projections, we apply the delta method (Ramirez-Villegas and Jarvis 2010) and then map and add the anomalies to observed temperature and precipitation normals (1981–2010) at stations from the Global Historical Climatology Network (GHCN) (Arguez et al. 2012) (<http://go.usa.gov/KmqH>). Geographic county centroids are then mapped to the nearest GHCN station (*see County-Weather Station Mapping*). The GHCN data set is a database of meteorological variables measured daily worldwide and is the most comprehensive set of climate data within the U.S. The use of station-level normals accounts for local meteorological phenomena, such as the urban heat island effect and land-sea interaction, that are not well reproduced by the gridded BCSO model output. Only GHCN stations that met the top two most strict National Climatic Data Center’s data completion requirements for the 30-year monthly climate normals definitions were used. Those are stations with either (1) complete records and/or (2) no more than five years missing and no more than three consecutive years missing among sufficiently complete years.

## 2) COUNTY-WEATHER STATION MAPPING

Since measured variables differ by station and because record lengths and data completion may also vary, different GHCN station mappings exist for temperature and precipitation. Each geographic county centroid is mapped to

the nearest GHCN station meeting either data completion requirement; no additional attention was given to the geographic placement of each station. Note that for large counties or for counties with complex terrain, baseline climate can spatially vary dramatically and a single representative weather station may not well characterize the average climate of the county. In some cases, multiple counties are mapped to the same weather station. Details regarding the mapping of geographic county centroids to GHCN weather stations are given in the supporting files.

### 3) DAILY PROJECTIONS

Both GCM output and surrogate output are treated at the monthly average level. As is standard with the BCSD downscaling technique (Wood et al. 2004), to generate daily temperature and precipitation, we assume that the relationship between the monthly means and the daily values come from a stationary distribution (e.g., Wood et al. 2002). We randomly assign each future year to a historical year between 1981–2010. Monthly averages are mapped to daily values from the GHCN stations using the additive relationship (for temperature) or multiplicative relationship (for precipitation) from that historical year. Where daily observations are missing from the 30-year historical record, we fill in the missing days and months using relationships between daily and monthly values from gridded datasets and between the climatological 30-year normal value at the GHCN station (see *Treatment of missing historical data*). While a single downscaling method is employed in this study, a comparison between our BCSD-derived daily projections and alternative methods that downscale to the daily level (e.g., Bias Correction/Constructed Analogs, Asynchronous Regional Regression Model) could be of interest (Maurer et al. 2010; Stoner et al. 2013).

#### c. 22nd century projections

For both SMME and MCP, we extend projections to 2200 by assuming that global mean temperature beyond 2100 follows the quantile of the MAGICC6 output that corresponds to that model’s position in the 2080–2099 average. We apply the model’s own pattern of forced change and use residuals that are equal to the residuals from 2000 to 2099. The residuals are run backwards to preserve continuity. (e.g., Jan. 2101 uses unforced variability from Dec. 2100, Feb. 2101 uses unforced variability from Nov. 2100, ect.) (Although some CMIP5 model runs extended beyond 2100, for consistency, we apply the same approach to all models.) As such, special caution should be used when considering 22nd century projections from this study, as they utilize residuals from the 21st century records of GCMs.

#### d. Treatment of missing historical data

As previously mentioned, to generate projections of daily temperature and precipitation, we map future monthly averages to historical daily weather variability using a 30-year record of observations (1981–2010). Observations are made at GHCN stations and missing data are addressed using the following methods for daily temperature and precipitation.

#### 1) DAILY TEMPERATURE

A complete set of daily  $T_{min}$  and  $T_{max}$  is constructed using daily records at GHCN stations across the U.S. (including Alaska and Hawaii) that have enough measurements for the NCDC to deem both the  $T_{min}$  and  $T_{max}$  record complete enough to calculate a 30-year monthly normal. (No more than five years are missing from the record and no more than three consecutive years are missing.) These stations may or may not be the same stations used to calculate a 30-year set of daily precipitation values (see below). In all, temperature records at 2688 stations are used.

Where daily  $T_{min}$  and  $T_{max}$  are missing within a month of GHCN station records, gridded monthly and daily data from 1981–2010 are sampled. For Alaska and Hawaii, the North American Regional Reanalysis (NARR) (Mesinger et al. 2006) data set is used (daily  $T_{min}$  and  $T_{max}$  are calculated from 3-hourly surface temperature) and for the CONUS, the Maurer et al. (2002) data set is used. If the number of missing daily observations within a particular month exceeds the World Meteorological Organization (1989) recommended 1–8 days, synthetic daily data (calculated from Eqn. A1) from the corresponding month and year is used to for each day in the month. However, if number of missing days is within the allowable recommended criteria, then the synthetic daily data is only sampled for the 1–8 missing days. In the latter case, the days within the month are then scaled to match the observed monthly mean that is calculated from all available observed daily values within the month. Daily values are not scaled if synthetic dailies are used for the entire month (i.e., the number of missing days is greater than 8).

$$T_{daily,syn} = T_{month,normal} + (T_{daily,gridded} - T_{month,gridded}) \quad (A1)$$

Daily average temperature ( $T_{avg}$ ) is not measured at the GHCN measurement stations. After complete 30-year records of daily  $T_{min}$  and  $T_{max}$  have been calculated, daily  $T_{avg}$  are approximated as  $(T_{min} + T_{max})/2$ . The 30-year  $T_{avg}$  normals are provided by the NCDC and are also approximated as the average of  $T_{min}$  and  $T_{max}$ .

## 2) DAILY PRECIPITATION

A complete set of daily precipitation totals is constructed using daily records of precipitation (liquid equivalent) at GHCN stations across the U.S. (including Alaska and Hawaii). Only stations that had enough measurements for the NCDC to deem the precipitation record complete enough to calculate a 30-year monthly normal<sup>1</sup>. These stations may or may not include those that were used to calculate daily  $T_{min}$  and  $T_{max}$  due to the completeness criteria. In all, 2722 stations were used.

Where daily precipitation amounts are missing with in a month, gridded monthly and daily data from 1981-2010 are sampled. For Alaska and Hawaii, the NARR data set is used and for the CONUS, the Maurer et al. (2002) data set is used. If the number of missing daily observations within a particular month exceeds the World Meteorological Organization (1989) recommended 1-8 days, synthetic daily data (calculated from Eqn. A2) from the corresponding month and year is used to replace the value for each day in the month. However, if the number of missing days is within the allowable recommended criteria, then synthetic daily data is only sampled for the 1-8 missing days. In the latter case, the daily precipitation totals within the month are then scaled to match the observed monthly precipitation total that is calculated from all available observed daily values with in the month.

Where daily precipitation projections exceed twice the historical daily maximum and ten times the model's mean daily precipitation rate for the month, we invoke a "spill over" routine that evenly distributes two-thirds of the incident daily precipitation to the nearest adjacent two days within the month. Daily maximum and minimum temperatures for Alaska and Hawaii were calculated from 3-hourly NARR data. For the rare case when the daily down-scaled  $T_{min} < T_{avg} < T_{max}$  is not satisfied,  $T_{min}$  and  $T_{max}$  are approximated as  $T_{avg} - 2.5^\circ\text{C}$  and  $T_{avg} + 2.5^\circ\text{C}$ , respectively.

$$P_{daily,syn} = \frac{P_{daily,gridded}}{P_{month,gridded}} P_{month} \quad (\text{A2})$$

If the number of missing daily observations is greater than 8, then the monthly average daily precipitation total is calculated as:

$$P_{month} = \frac{P_{month,normal}}{\hat{P}_{month,normal}} P_{month,gridded} \quad (\text{A3})$$

Where  $\hat{P}_{month,normal}$  is the monthly normal from the gridded dataset.

Daily precipitation totals and temperature at each GHCN observation station are mapped to the nearest county centroid latitude and longitude.

## e. Projection variance

For a fixed location at year  $t$ , the annual local temperature ( $X_{m,s}(t)$ ) for each model ( $m$ ) and scenario ( $s$ ) can be expressed as the sum of the forced component of climate change ( $x_{m,s}(t)$ ) and unforced variability ( $\epsilon_{m,s}(t)$ ). The forced component of climate change ( $x$ ) is estimated as a 30-year running average of annual temperature. Unforced variability is estimated as the difference between the annual projection and the forced component of climate change,

$$X_{m,s}(t) = x_{m,s}(t) + \epsilon_{m,s}(t). \quad (\text{A4})$$

Following Hawkins and Sutton (2009), assuming each source of uncertainty is independent, the total variance can be expressed as the sum of the variances of the forced uncertainty component  $F(t)$ , the unforced component  $U(t)$ , and scenario uncertainty  $S(t)$ .

$$T(t) = F(t) + U(t) + S(t). \quad (\text{A5})$$

Assuming each of the scenarios are equally probable, we estimate the average scenario forced model uncertainty  $F(t)$  as the weighted variance of forced climate change.

$$F(t) = \frac{1}{N_s} \sum_s \text{var}_m^{W_m}(x_{m,s}(t)), \quad (\text{A6})$$

where  $N_s$  is the number of emissions scenarios and  $W_m$  are the probability weights calculated in Section 2 (weights are equal for the MCPR method).

Unlike Hawkins and Sutton (2009), we assume unforced (i.e., natural) variability is not independent of time and scenario, and calculate the average scenario unforced model uncertainty as

$$U(t) = \frac{1}{N_s} \sum_s \text{var}_m^{W_m}(\epsilon_{m,s}(t)), \quad (\text{A7})$$

The scenario uncertainty is estimated as the standard deviation of the weighted multi-model means,

$$S(t) = \text{var}_s \left( \sum_m W_m x_{m,s}(t) \right). \quad (\text{A8})$$

The fraction of forced and scenario variability is assumed to be 0% prior to 2000, while unforced variability is assumed to comprise 100% of total variability prior to 2000.

<sup>1</sup>No more than five years are missing from the record and no more than three consecutive years are missing

## APPENDIX B

## Guidance

While uses of the probabilistic projections are many, we particularly note their utility as input for sector-specific impacts models and damage functions such as those used for agriculture (Schlenker and Roberts 2009), human mortality (Deschn  s and Greenstone 2011), energy demand (Auffhammer and Aroonruengsawat 2011), assessing future heat humid heat stress, and for projecting heating, cooling, and growing degree days (Houser et al. 2015). Some guidance is given here for user selection of forcing scenarios and the coincident anticipated median contiguous U.S. (CONUS) warming.

Depending on the application, one may desire to choose one probabilistic method over the other. For instance, the MCPR is not bound to the global mean temperature trajectories of the CMIP5 ensemble, while the SMME is. Applications wishing to remain more rooted in GCM projections may opt for the SMME, as it relies less on pattern scaling and is more true to modeled pairs of forced and unforced variability. Where available, the use of multiple realizations and patterns that are not constant with temperature or include other covariates could allow a similar complexity in the MCPR framework, but this extension is beyond the scope of this paper.

## References

- Arguez, A., I. Durre, S. Applequist, R. S. Vose, M. F. Squires, X. Yin, R. R. Heim Jr, and T. W. Owen, 2012: NOAA's 1981–2010 US climate normals: An overview. *Bulletin of the American Meteorological Society*, **93** (11), 1687–1697.
- Auffhammer, M., and A. Aroonruengsawat, 2011: Simulating the impacts of climate change, prices and population on California's residential electricity consumption. *Climatic Change*, **109** (1), 191–210, doi:10.1007/s10584-011-0299-y.
- Brekke, L., B. L. Thrasher, E. P. Maurer, and T. Pruitt, 2013: *Downscaled CMIP3 and CMIP5 Climate Projections: Release of Downscaled CMIP5 Climate Projections, Comparison with Preceding Information, and Summary of User Needs*. U.S. Department of the Interior, Bureau of Reclamation, Technical Service Center, Denver, Colorado, 116 pp., URL [http://gdo-dcp.ucllnl.org/downscaled\\_cmip\\_projections/techmemo/downscaled\\_climate.pdf](http://gdo-dcp.ucllnl.org/downscaled_cmip_projections/techmemo/downscaled_climate.pdf).
- Delworth, T. L., and Coauthors, 2012: Simulated climate and climate change in the GFDL CM2.5 high-resolution coupled climate model. *Journal of Climate*, **25** (8).
- Deschn  s, O., and M. Greenstone, 2011: Climate change, mortality, and adaptation: Evidence from annual fluctuations in weather in the U.S. *American Economic Journal: Applied Economics*, **3** (4), 152–85, doi:10.1257/app.3.4.152.
- Flato, G., and Coauthors, 2013: *Evaluation of Climate Models*, book section 9, 741–866. Cambridge University Press, Cambridge, United Kingdom and New York, NY, USA, doi:10.1017/CBO9781107415324.020.
- Hawkins, E., and R. Sutton, 2009: The Potential to Narrow Uncertainty in Regional Climate Predictions. *Bulletin of the American Meteorological Society*, **90** (8), 1095–1107, doi:10.1175/2009BAMS2607.1.
- Ho, C. K., D. B. Stephenson, M. Collins, C. A. T. Ferro, and S. J. Brown, 2011: Calibration Strategies: A Source of Additional Uncertainty in Climate Change Projections. *Bull. Am. Meteorol. Soc.*, **93** (1), 21–26, doi:10.1175/2011BAMS3110.1.
- Houser, T., and Coauthors, 2015: *Economic Risks of Climate Change: An American Prospectus*. Columbia University Press, New York, New York, 384 pp.
- Mahmood, R., and M. S. Babel, 2013: Evaluation of SDSM developed by annual and monthly sub-models for downscaling temperature and precipitation in the Jhelum Basin, Pakistan and India. *Theoretical and Applied Climatology*, **113** (1-2), 27–44, doi:10.1007/s00704-012-0765-0.
- Maurer, E. P., H. G. Hidalgo, T. Das, M. D. Dettinger, and D. R. Cayan, 2010: The utility of daily large-scale climate data in the assessment of climate change impacts on daily streamflow in California. *Hydrology and Earth System Sciences*, **14** (6), 1125–1138, doi:10.5194/hess-14-1125-2010.
- Maurer, E. P., A. W. Wood, J. C. Adam, D. P. Lettenmaier, and B. Nijssen, 2002: A long-term hydrologically based dataset of land surface fluxes and states for the conterminous United States. *Journal of Climate*, **15** (22), 3237–3251.
- McGinnis, S., D. Nychka, and L. O. Mearns, 2015: A new distribution mapping technique for climate model bias correction. *Machine learning and data mining approaches to climate science: proceedings of the Fourth International Workshop on Climate Informatics*, V. Lakshmanan, E. Gilleland, A. McGovern, and M. Tingley, Eds., Springer.
- Meinshausen, M., and Coauthors, 2011: The RCP greenhouse gas concentrations and their extensions from 1765 to 2300. *Climatic Change*, **109** (1-2), 213–241, doi:10.1007/s10584-011-0156-z.
- Mesinger, F., and Coauthors, 2006: North american regional reanalysis. *Bulletin of the American Meteorological Society*, **87** (3).
- O'Neill, B. C., E. Kriegler, K. Riahi, K. L. Ebi, S. Hallegatte, T. R. Carter, R. Mathur, and D. P. Van Vuuren, 2014: A new scenario framework for climate change research: the concept of shared socioeconomic pathways. *Clim. Change*, **122** (3), 387–400, doi:10.1007/s10584-013-0905-2.
- O'Neill, B. C., E. Kriegler, K. Riahi, K. L. Ebi, S. Hallegatte, T. R. Carter, R. Mathur, and D. P. Vuuren, 2013: A new scenario framework for climate change research: the concept of shared socioeconomic pathways. *Climatic Change*, **122** (3), 387–400, doi:10.1007/s10584-013-0905-2.
- O'Neill, B. C., and Coauthors, 2015: The roads ahead: Narratives for shared socioeconomic pathways describing world futures in the 21st century. *Glob. Environ. Chang.*, doi:10.1016/j.gloenvcha.2015.01.004.
- Ramirez-Villegas, J., and A. Jarvis, 2010: Downscaling Global Circulation Model Outputs: The Delta Method Decision and Policy Analysis Working Paper No. 1. Tech. rep., Centro Internacional de Agricultura Tropical (CIAT), Valle del Cauca, Colombia. URL <http://www.ccafs-climate.org/downloads/docs/Downscaling-WP-01.pdf>.
- Riahi, K., 2013: Preliminary IAM scenarios based on the RCP/SSP framework. *Preliminary IAM scenarios based on the RCP/SSP*

*framework*, Energy Modeling Forum, Snowmass, CO, URL [http://emf.stanford.edu/files/docs/340/Riahi\\_SSP\\_Snowmass2013.pdf](http://emf.stanford.edu/files/docs/340/Riahi_SSP_Snowmass2013.pdf).

Schlenker, W., and M. J. Roberts, 2009: Nonlinear temperature effects indicate severe damages to U.S. crop yields under climate change. *Proceedings of the National Academy of Sciences*, **106** (37), 15 594–15 598, doi:10.1073/pnas.0906865106, <http://www.pnas.org/content/106/37/15594.full.pdf+html>.

Stoner, A. M. K., K. Hayhoe, X. Yang, and D. J. Wuebbles, 2013: An asynchronous regional regression model for statistical downscaling of daily climate variables. *International Journal of Climatology*, **33** (11), 2473–2494, doi:10.1002/joc.3603.

Van Vuuren, D. P., and Coauthors, 2011: The representative concentration pathways: an overview. *Climatic Change*, **109**, 5–31, doi:10.1007/s10584-011-0148-z.

Wood, A. W., L. R. Leung, V. Sridhar, and D. P. Lettenmaier, 2004: Hydrologic Implications of Dynamical and Statistical Approaches to Downscaling Climate Model Outputs. *Climatic Change*, **62** (1-3), 189–216, doi:10.1023/B:CLIM.0000013685.99609.9e.

Wood, A. W., E. P. Maurer, A. Kumar, and D. P. Lettenmaier, 2002: Long-range experimental hydrologic forecasting for the eastern United States. *Journal of Geophysical Research: Atmospheres*, **107** (D20), ACL 6–1–ACL 6–15, doi:10.1029/2001JD000659.

World Meteorological Organization, 1989: Calculation of monthly and annual 30-year standard normals. WCDP, Washington, D.C., World Meteorological Organization (WMO), Vol. 10.

TABLE A1. Percentiles of projected global mean temperature change (°C), relative to 1981-2010.

|         | 2040-2059 |      |      |      |      | 2080-2099 |      |      |      |      | 2140-2159 |      |      |      |      |
|---------|-----------|------|------|------|------|-----------|------|------|------|------|-----------|------|------|------|------|
|         | 5th       | 17th | 50th | 83rd | 95th | 5th       | 17th | 50th | 83rd | 95th | 5th       | 17th | 50th | 83rd | 95th |
| RCP 8.5 | 1.1       | 1.2  | 1.6  | 2.1  | 2.5  | 2.3       | 2.6  | 3.5  | 4.9  | 6.2  | 3.9       | 4.5  | 6.1  | 9.3  | 11.9 |
| RCP 6.0 | 0.7       | 0.8  | 1.1  | 1.4  | 1.6  | 1.3       | 1.5  | 2.1  | 3.0  | 3.8  | 1.7       | 2.1  | 3.0  | 4.5  | 5.7  |
| RCP 4.5 | 0.7       | 0.9  | 1.2  | 1.6  | 1.9  | 0.9       | 1.1  | 1.8  | 2.5  | 3.2  | 1.0       | 1.2  | 2.0  | 3.0  | 4.1  |
| RCP 2.6 | 0.5       | 0.6  | 0.9  | 1.2  | 1.5  | 0.4       | 0.5  | 0.9  | 1.4  | 1.8  | 0.3       | 0.4  | 0.7  | 1.4  | 1.9  |

TABLE A2. CMIP5 models included in this analysis

| Model          | RCP 2.6 | RCP 4.5 | RCP 6.0 | RCP 8.5 |
|----------------|---------|---------|---------|---------|
| access1-0      |         | X       |         | X       |
| access1-3      |         | X       |         | X       |
| bcc-csm1-1     | X       | X       | X       | X       |
| bcc-csm1-1-m   |         | X       |         | X       |
| bnu-esm        | X       | X       |         | X       |
| canesm2        | X       | X       |         | X       |
| ccsm4          | X       | X       | X       | X       |
| cesm1-bgc      |         | X       |         | X       |
| cesm1-cam5     | X       | X       | X       | X       |
| cmcc-cm        |         | X       |         | X       |
| cnrm-cm5       |         | X       |         | X       |
| csiro-mk3-6-0  | X       | X       |         | X       |
| fgoals-g2      | X       | X       |         | X       |
| fio-esm        | X       | X       | X       | X       |
| gfdl-cm3       | X       | X       | X       | X       |
| gfdl-esm2g     | X       | X       | X       | X       |
| gfdl-esm2m     | X       | X       | X       | X       |
| giss-e2-r      | X       | X       | X       | X       |
| hadgem2-ao     | X       | X       | X       | X       |
| hadgem2-cc     |         | X       |         | X       |
| hadgem2-es     | X       | X       | X       | X       |
| inmcm4         |         | X       |         | X       |
| ipsl-cm5a-lr   | X       | X       | X       | X       |
| ipsl-cm5a-mr   | X       | X       | X       | X       |
| ipsl-cm5b-lr   |         | X       |         | X       |
| miroc-esm      | X       | X       | X       | X       |
| miroc-esm-chem | X       | X       | X       | X       |
| miroc5         | X       | X       | X       | X       |
| mpi-esm-lr     | X       | X       |         | X       |
| mpi-esm-mr     | X       | X       |         | X       |
| mri-cgcm3      | X       | X       | X       | X       |
| noresm1-m      | X       | X       | X       | X       |
| noresm1-me     | X       | X       | X       | X       |

TABLE A3. Selected patterns and surrogate/model mixed ensemble probability weights used for RCP 2.6. “Scaled” models are surrogates used to populate the respective quantile of the temperature distribution. FIO-ESM is not used because its global mean temperature is outside the range of the MAGICC PDF.

| Quantile | SMME bin | Model                 | SMME weight | 2080–2099 global $\Delta T$ ( $^{\circ}\text{C}$ ) | 2080–2099 CONUS $\Delta P$ (%) |
|----------|----------|-----------------------|-------------|----------------------------------------------------|--------------------------------|
| 0.00     | 1        | gfdl-esm2g            | 0.0400      | 0.25                                               | -1.41                          |
| 0.04     | 1        | scaled fio-esm        | 0.0400      | 0.39                                               | -0.70                          |
| 0.10     | 2        | giss-e2-r             | 0.0200      | 0.46                                               | 2.42                           |
| 0.10     | 2        | scaled giss-e2-r      | 0.0200      | 0.46                                               | 2.39                           |
| 0.16     | 3        | scaled fgoals-g2      | 0.0400      | 0.52                                               | 2.99                           |
| 0.20     | 3        | fgoals-g2             | 0.0400      | 0.58                                               | 3.34                           |
| 0.30     | 4        | scaled mpi-esm-lr     | 0.1000      | 0.64                                               | 3.38                           |
| 0.40     | 4        | mpi-esm-lr            | 0.1000      | 0.78                                               | 4.13                           |
| 0.40     | 5        | mpi-esm-mr            | 0.0333      | 0.78                                               | 2.57                           |
| 0.43     | 5        | bcc-csm1-1            | 0.0333      | 0.82                                               | 0.33                           |
| 0.46     | 5        | noresm1-m             | 0.0333      | 0.84                                               | 0.59                           |
| 0.47     | 5        | ccsm4                 | 0.0333      | 0.86                                               | 5.01                           |
| 0.55     | 5        | noresm1-me            | 0.0333      | 0.94                                               | 6.42                           |
| 0.55     | 5        | mri-cgcm3             | 0.0333      | 0.92                                               | 3.78                           |
| 0.63     | 6        | miroc5                | 0.0400      | 1.03                                               | 4.11                           |
| 0.65     | 6        | ipsl-cm5a-mr          | 0.0400      | 1.07                                               | -1.39                          |
| 0.66     | 6        | hadgem2-ao            | 0.0400      | 1.08                                               | -0.23                          |
| 0.68     | 6        | bnu-esm               | 0.0400      | 1.13                                               | 1.02                           |
| 0.76     | 6        | ipsl-cm5a-lr          | 0.0400      | 1.25                                               | 6.10                           |
| 0.82     | 7        | hadgem2-es            | 0.0200      | 1.40                                               | 9.26                           |
| 0.84     | 7        | cesm1-cam5            | 0.0200      | 1.46                                               | 13.56                          |
| 0.85     | 7        | csiro-mk3-6-0         | 0.0200      | 1.45                                               | 10.41                          |
| 0.85     | 7        | canesm2               | 0.0200      | 1.47                                               | 7.79                           |
| 0.90     | 8        | scaled miroc-esm-chem | 0.0200      | 1.62                                               | 7.43                           |
| 0.91     | 8        | miroc-esm             | 0.0200      | 1.65                                               | 7.25                           |
| 0.93     | 9        | miroc-esm-chem        | 0.0300      | 1.69                                               | 7.78                           |
| 0.97     | 9        | gfdl-cm3              | 0.0300      | 1.92                                               | 6.14                           |
| 0.99     | 10       | scaled hadgem2-es     | 0.0100      | 2.18                                               | 14.41                          |
| 0.99     | 10       | scaled miroc-esm-chem | 0.0100      | 2.18                                               | 10.05                          |

TABLE A4. Selected patterns and surrogate/model mixed ensemble probability weights used for RCP 4.5. “Scaled” models are surrogates used to populate the respective quantile of the temperature distribution.

| Quantile | SMME bin | Model                 | SMME weight | 2080–2099 global $\Delta T$ ( $^{\circ}\text{C}$ ) | 2080–2099 CONUS $\Delta P$ (%) |
|----------|----------|-----------------------|-------------|----------------------------------------------------|--------------------------------|
| 0.04     | 1        | scaled gfdl-esm2g     | 0.0400      | 0.93                                               | 4.63                           |
| 0.07     | 1        | gfdl-esm2g            | 0.0400      | 0.99                                               | 4.93                           |
| 0.09     | 2        | fio-esm               | 0.0200      | 1.03                                               | 1.64                           |
| 0.10     | 2        | scaled gfdl-esm2m     | 0.0200      | 1.03                                               | 2.37                           |
| 0.17     | 3        | gfdl-esm2m            | 0.0267      | 1.17                                               | 2.70                           |
| 0.18     | 3        | giss-e2-r-cc          | 0.0267      | 1.17                                               | 1.98                           |
| 0.20     | 3        | giss-e2-r             | 0.0267      | 1.19                                               | 2.02                           |
| 0.21     | 4        | inmcm4                | 0.0500      | 1.21                                               | 7.65                           |
| 0.25     | 4        | fgoals-g2             | 0.0500      | 1.31                                               | 2.89                           |
| 0.29     | 4        | giss-e2-h-cc          | 0.0500      | 1.36                                               | 6.51                           |
| 0.37     | 4        | bcc-csm1-l-m          | 0.0500      | 1.49                                               | -4.01                          |
| 0.41     | 5        | cesm1-bgc             | 0.0182      | 1.56                                               | 4.52                           |
| 0.42     | 5        | bcc-csm1-l            | 0.0182      | 1.57                                               | 4.23                           |
| 0.44     | 5        | mpi-esm-lr            | 0.0182      | 1.62                                               | 5.52                           |
| 0.45     | 5        | noresm1-m             | 0.0182      | 1.60                                               | 5.92                           |
| 0.45     | 5        | ipsl-cm5b-lr          | 0.0182      | 1.62                                               | 9.24                           |
| 0.45     | 5        | ccsm4                 | 0.0182      | 1.62                                               | 6.16                           |
| 0.45     | 5        | mri-cgcm3             | 0.0182      | 1.63                                               | 10.28                          |
| 0.46     | 5        | noresm1-me            | 0.0182      | 1.67                                               | 1.67                           |
| 0.48     | 5        | mpi-esm-mr            | 0.0182      | 1.68                                               | 4.53                           |
| 0.48     | 5        | miroc5                | 0.0182      | 1.71                                               | 0.34                           |
| 0.58     | 5        | cnrm-cm5              | 0.0182      | 1.88                                               | 6.97                           |
| 0.70     | 6        | access1-3             | 0.0182      | 2.10                                               | 9.22                           |
| 0.71     | 6        | cmcc-cm               | 0.0182      | 2.14                                               | 0.21                           |
| 0.71     | 6        | bnu-esm               | 0.0182      | 2.13                                               | 1.06                           |
| 0.72     | 6        | ipsl-cm5a-lr          | 0.0182      | 2.17                                               | -2.60                          |
| 0.74     | 6        | access1-0             | 0.0182      | 2.21                                               | 3.10                           |
| 0.74     | 6        | ipsl-cm5a-mr          | 0.0182      | 2.23                                               | -4.01                          |
| 0.74     | 6        | csiro-mk3-6-0         | 0.0182      | 2.24                                               | 13.46                          |
| 0.77     | 6        | canesm2               | 0.0182      | 2.30                                               | 13.32                          |
| 0.78     | 6        | hadgem2-cc            | 0.0182      | 2.31                                               | 2.77                           |
| 0.78     | 6        | cesm1-cam5            | 0.0182      | 2.30                                               | 6.44                           |
| 0.79     | 6        | hadgem2-ao            | 0.0182      | 2.36                                               | -1.42                          |
| 0.82     | 7        | miroc-esm             | 0.0200      | 2.46                                               | 4.19                           |
| 0.84     | 7        | hadgem2-es            | 0.0200      | 2.55                                               | 8.15                           |
| 0.85     | 7        | miroc-esm-chem        | 0.0200      | 2.53                                               | 11.40                          |
| 0.88     | 7        | gfdl-cm3              | 0.0200      | 2.70                                               | 10.00                          |
| 0.90     | 8        | scaled miroc-esm-chem | 0.0200      | 2.80                                               | 12.58                          |
| 0.90     | 8        | scaled hadgem2-ao     | 0.0200      | 2.80                                               | -1.68                          |
| 0.95     | 9        | scaled miroc-esm-chem | 0.0300      | 3.23                                               | 14.51                          |
| 0.95     | 9        | scaled hadgem2-ao     | 0.0300      | 3.23                                               | -1.94                          |
| 0.99     | 10       | scaled miroc-esm-chem | 0.0100      | 4.12                                               | 18.54                          |
| 0.99     | 10       | scaled hadgem2-ao     | 0.0100      | 4.12                                               | -2.47                          |

TABLE A5. Selected patterns and surrogate/model mixed ensemble probability weights used for RCP 6.0. “Scaled” models are surrogates used to populate the respective quantile of the temperature distribution.

| Quantile | SMME bin | Model                 | SMME weight | 2080–2099 global $\Delta T$ ( $^{\circ}\text{C}$ ) | 2080–2099 CONUS $\Delta P$ (%) |
|----------|----------|-----------------------|-------------|----------------------------------------------------|--------------------------------|
| 0.04     | 1        | scaled gfdl-esm2m     | 0.0400      | 1.31                                               | 2.22                           |
| 0.04     | 1        | scaled fio-esm        | 0.0400      | 1.31                                               | -0.78                          |
| 0.10     | 2        | scaled gfdl-esm2m     | 0.0200      | 1.42                                               | 2.42                           |
| 0.10     | 2        | scaled fio-esm        | 0.0200      | 1.42                                               | -0.85                          |
| 0.15     | 3        | gfdl-esm2g            | 0.0400      | 1.50                                               | 2.40                           |
| 0.18     | 3        | fio-esm               | 0.0400      | 1.56                                               | -0.93                          |
| 0.24     | 4        | giss-e2-r             | 0.0667      | 1.62                                               | 3.23                           |
| 0.25     | 4        | gfdl-esm2m            | 0.0667      | 1.66                                               | 2.82                           |
| 0.36     | 4        | noresm1-m             | 0.0667      | 1.85                                               | 7.76                           |
| 0.41     | 5        | noresm1-me            | 0.0500      | 1.94                                               | 4.27                           |
| 0.43     | 5        | bcc-csm1-l            | 0.0500      | 1.96                                               | 5.09                           |
| 0.44     | 5        | miroc5                | 0.0500      | 1.98                                               | 1.39                           |
| 0.49     | 5        | ccsm4                 | 0.0500      | 2.11                                               | 8.42                           |
| 0.65     | 6        | csiro-mk3-6-0         | 0.0400      | 2.41                                               | 1.45                           |
| 0.67     | 6        | hadgem2-ao            | 0.0400      | 2.49                                               | -1.54                          |
| 0.69     | 6        | ipsl-cm5a-lr          | 0.0400      | 2.55                                               | -1.53                          |
| 0.72     | 6        | ipsl-cm5a-mr          | 0.0400      | 2.61                                               | -5.75                          |
| 0.78     | 6        | cesm1-cam5            | 0.0400      | 2.76                                               | 17.36                          |
| 0.82     | 7        | miroc-esm             | 0.0200      | 2.93                                               | 10.84                          |
| 0.85     | 7        | miroc-esm-chem        | 0.0200      | 3.03                                               | 9.40                           |
| 0.86     | 7        | hadgem2-es            | 0.0200      | 3.06                                               | 6.42                           |
| 0.87     | 7        | gfdl-cm3              | 0.0200      | 3.10                                               | 11.80                          |
| 0.90     | 8        | scaled miroc-esm-chem | 0.0200      | 3.25                                               | 10.08                          |
| 0.90     | 8        | scaled hadgem2-es     | 0.0200      | 3.25                                               | 6.83                           |
| 0.95     | 9        | scaled miroc-esm-chem | 0.0300      | 3.79                                               | 11.74                          |
| 0.95     | 9        | scaled hadgem2-es     | 0.0300      | 3.79                                               | 7.95                           |
| 0.99     | 10       | scaled miroc-esm-chem | 0.0100      | 4.47                                               | 13.87                          |
| 0.99     | 10       | scaled hadgem2-es     | 0.0100      | 4.47                                               | 9.40                           |

TABLE A6. Selected patterns and surrogate/model mixed ensemble probability weights used for RCP 8.5. “Scaled” models are surrogates used to populate the respective quantile of the temperature distribution.

| Quantile | SMME bin | Model                 | SMME weight | 2080–2099 global $\Delta T$ ( $^{\circ}\text{C}$ ) | 2080–2099 CONUS $\Delta P$ (%) |
|----------|----------|-----------------------|-------------|----------------------------------------------------|--------------------------------|
| 0.04     | 1        | scaled giss-e2-r      | 0.0400      | 2.26                                               | 8.37                           |
| 0.04     | 1        | scaled inmcm4         | 0.0400      | 2.26                                               | 1.58                           |
| 0.10     | 2        | scaled giss-e2-r      | 0.0200      | 2.43                                               | 9.00                           |
| 0.10     | 2        | scaled inmcm4         | 0.0200      | 2.43                                               | 1.70                           |
| 0.12     | 3        | giss-e2-r             | 0.0267      | 2.50                                               | 9.26                           |
| 0.14     | 3        | inmcm4                | 0.0267      | 2.58                                               | 1.81                           |
| 0.18     | 3        | gfdl-esm2m            | 0.0267      | 2.64                                               | 5.29                           |
| 0.22     | 4        | gfdl-esm2g            | 0.0500      | 2.77                                               | 7.20                           |
| 0.33     | 4        | fgoals-g2             | 0.0500      | 3.03                                               | 1.52                           |
| 0.39     | 4        | noresm1-m             | 0.0500      | 3.14                                               | 6.60                           |
| 0.40     | 4        | mri-cgcm3             | 0.0500      | 3.19                                               | 13.38                          |
| 0.43     | 5        | bcc-csm1-1-m          | 0.0182      | 3.24                                               | 4.85                           |
| 0.45     | 5        | miroc5                | 0.0182      | 3.31                                               | -0.33                          |
| 0.46     | 5        | ipsl-cm5b-lr          | 0.0182      | 3.33                                               | 9.32                           |
| 0.46     | 5        | noresm1-me            | 0.0182      | 3.32                                               | 2.98                           |
| 0.47     | 5        | bcc-csm1-1            | 0.0182      | 3.34                                               | 2.00                           |
| 0.50     | 5        | fio-esm               | 0.0182      | 3.42                                               | 6.50                           |
| 0.50     | 5        | cnrm-cm5              | 0.0182      | 3.47                                               | 11.10                          |
| 0.51     | 5        | cesm1-bgc             | 0.0182      | 3.48                                               | 6.61                           |
| 0.51     | 5        | mpi-esm-mr            | 0.0182      | 3.52                                               | 5.63                           |
| 0.53     | 5        | mpi-esm-lr            | 0.0182      | 3.55                                               | 5.33                           |
| 0.53     | 5        | ccsm4                 | 0.0182      | 3.59                                               | 5.39                           |
| 0.64     | 6        | access1-3             | 0.0143      | 3.96                                               | 15.44                          |
| 0.65     | 6        | csiro-mk3-6-0         | 0.0143      | 3.97                                               | 11.92                          |
| 0.66     | 6        | hadgem2-ao            | 0.0143      | 4.04                                               | 2.02                           |
| 0.66     | 6        | access1-0             | 0.0143      | 4.05                                               | 0.81                           |
| 0.67     | 6        | cesm1-cam5            | 0.0143      | 4.04                                               | 10.92                          |
| 0.69     | 6        | cmcc-cm               | 0.0143      | 4.14                                               | 5.39                           |
| 0.71     | 6        | bnu-esm               | 0.0143      | 4.27                                               | 3.41                           |
| 0.73     | 6        | ipsl-cm5a-mr          | 0.0143      | 4.36                                               | -10.46                         |
| 0.75     | 6        | canesm2               | 0.0143      | 4.41                                               | 22.06                          |
| 0.75     | 6        | ipsl-cm5a-lr          | 0.0143      | 4.43                                               | -5.31                          |
| 0.78     | 6        | hadgem2-cc            | 0.0143      | 4.60                                               | 5.97                           |
| 0.78     | 6        | gfdl-cm3              | 0.0143      | 4.61                                               | 12.92                          |
| 0.78     | 6        | miroc-esm             | 0.0143      | 4.62                                               | 5.09                           |
| 0.78     | 6        | hadgem2-es            | 0.0143      | 4.63                                               | 6.94                           |
| 0.83     | 7        | miroc-esm-chem        | 0.0400      | 4.90                                               | 4.90                           |
| 0.84     | 7        | scaled miroc-esm-chem | 0.0400      | 4.93                                               | 4.93                           |
| 0.90     | 8        | scaled gfdl-cm3       | 0.0200      | 5.45                                               | 15.26                          |
| 0.90     | 8        | scaled miroc-esm-chem | 0.0200      | 5.45                                               | 5.45                           |
| 0.95     | 9        | scaled gfdl-cm3       | 0.0300      | 6.20                                               | 17.35                          |
| 0.95     | 9        | scaled miroc-esm-chem | 0.0300      | 6.20                                               | 6.20                           |
| 0.99     | 10       | scaled gfdl-cm3       | 0.0100      | 8.07                                               | 22.59                          |
| 0.99     | 10       | scaled miroc-esm-chem | 0.0100      | 8.07                                               | 8.07                           |

TABLE A7. Projected regional JJA temperature change (°C) under all RCPs for 2080-2099

| JJA<br>2080-2099                                 | RCP 8.5 |         |          | RCP 6.0 |         |         | RCP 4.5 |         |         | RCP 2.6 |         |         |
|--------------------------------------------------|---------|---------|----------|---------|---------|---------|---------|---------|---------|---------|---------|---------|
|                                                  | 50      | 17-83   | 5-95     | 50      | 17-83   | 5-95    | 50      | 17-83   | 5-95    | 50      | 17-83   | 5-95    |
| CONUS (1981–2010 normal: 22.6°C)                 |         |         |          |         |         |         |         |         |         |         |         |         |
| CMIP5                                            | 5.3     | 4.4–6.9 | 3.8–7.4  | 3.4     | 2.8–4.5 | 1.6–5.0 | 2.7     | 1.8–3.9 | 1.5–4.4 | 1.4     | 0.9–2.1 | 0.6–2.6 |
| SMME                                             | 5.2     | 3.9–7.4 | 3.6–9.3  | 3.2     | 2.5–4.6 | 1.5–5.7 | 2.4     | 1.8–4.0 | 1.7–5.1 | 1.3     | 0.9–2.0 | 0.6–2.9 |
| MCPR                                             | 5.0     | 3.9–7.3 | 3.5–9.2  | 3.2     | 2.4–4.5 | 2.1–5.7 | 2.6     | 1.8–3.9 | 1.4–4.9 | 1.4     | 0.8–2.2 | 0.5–2.6 |
| Northeast (1981–2010 normal: 20.2°C)             |         |         |          |         |         |         |         |         |         |         |         |         |
| CMIP5                                            | 5.5     | 4.3–6.7 | 3.3–8.2  | 3.2     | 2.4–4.4 | 1.7–5.7 | 2.7     | 1.5–3.4 | 1.3–4.7 | 1.6     | 1.0–2.2 | 0.6–2.4 |
| SMME                                             | 5.4     | 3.3–7.1 | 2.6–9.3  | 3.2     | 2.2–4.8 | 1.6–5.7 | 2.6     | 1.4–4.0 | 1.2–5.1 | 1.4     | 1.0–2.0 | 0.5–2.9 |
| MCPR                                             | 4.9     | 3.9–7.6 | 3.4–9.2  | 3.2     | 2.3–4.7 | 2.0–5.8 | 2.4     | 1.7–3.6 | 1.4–5.2 | 1.3     | 0.8–2.1 | 0.6–2.7 |
| Southeast (1981–2010 normal: 25.6°C)             |         |         |          |         |         |         |         |         |         |         |         |         |
| CMIP5                                            | 4.7     | 4.1–6.1 | 3.1–7.0  | 3.0     | 2.5–3.8 | 1.6–4.8 | 2.4     | 1.6–3.1 | 1.2–4.0 | 1.3     | 0.9–1.9 | 0.8–2.1 |
| SMME                                             | 4.5     | 3.1–6.5 | 2.8–8.2  | 2.8     | 2.3–4.0 | 1.5–5.1 | 2.3     | 1.6–3.5 | 1.2–4.7 | 1.1     | 0.9–1.6 | 0.7–2.5 |
| MCPR                                             | 4.4     | 3.5–6.6 | 3.1–7.8  | 2.9     | 2.2–4.0 | 1.8–4.9 | 2.2     | 1.5–3.3 | 1.2–4.6 | 1.1     | 0.7–1.7 | 0.4–2.4 |
| South Central (1981–2010 normal: 27.2°C)         |         |         |          |         |         |         |         |         |         |         |         |         |
| CMIP5                                            | 4.9     | 4.0–6.5 | 3.5–7.1  | 3.2     | 2.7–4.0 | 1.3–5.0 | 2.5     | 1.6–3.1 | 1.0–4.0 | 1.3     | 0.9–2.0 | 0.8–2.2 |
| SMME                                             | 4.7     | 3.8–6.7 | 3.3–8.5  | 3.2     | 2.5–4.1 | 1.2–5.0 | 2.5     | 1.6–3.8 | 1.0–4.9 | 1.1     | 0.7–1.9 | 0.7–2.5 |
| MCPR                                             | 4.8     | 3.7–6.8 | 3.0–8.3  | 3.1     | 2.2–4.3 | 2.0–5.6 | 2.4     | 1.5–3.9 | 1.1–5.0 | 1.2     | 0.6–2.1 | 0.2–2.8 |
| Upper Great Plains (1981–2010 normal: 22.1°C)    |         |         |          |         |         |         |         |         |         |         |         |         |
| CMIP5                                            | 6.3     | 4.2–7.5 | 3.6–8.2  | 3.9     | 2.9–4.7 | 1.6–5.2 | 3.0     | 1.8–4.3 | 1.1–4.7 | 1.6     | 0.9–2.4 | 0.6–2.7 |
| SMME                                             | 6.0     | 4.0–7.8 | 3.6–9.8  | 3.8     | 2.0–4.8 | 1.5–5.5 | 2.9     | 1.8–4.6 | 1.6–5.8 | 1.4     | 0.9–2.1 | 0.6–2.7 |
| MCPR                                             | 5.6     | 4.1–8.1 | 3.4–9.9  | 3.5     | 2.5–5.3 | 2.0–6.2 | 2.8     | 1.9–4.1 | 1.4–5.9 | 1.6     | 0.7–2.4 | 0.4–3.5 |
| Midwest (1981–2010 normal: 21.5°C)               |         |         |          |         |         |         |         |         |         |         |         |         |
| CMIP5                                            | 5.7     | 4.3–7.8 | 3.5–8.2  | 3.7     | 2.6–5.0 | 1.8–5.4 | 2.8     | 1.8–4.5 | 1.2–5.2 | 1.6     | 0.9–2.5 | 0.8–3.0 |
| SMME                                             | 5.5     | 3.6–8.0 | 3.3–9.9  | 3.5     | 2.3–5.0 | 1.7–6.2 | 2.5     | 1.5–4.9 | 1.4–6.2 | 1.3     | 0.9–2.3 | 0.5–3.2 |
| MCPR                                             | 5.3     | 4.0–7.9 | 3.7–9.3  | 3.4     | 2.5–5.1 | 2.2–6.0 | 2.6     | 1.7–3.8 | 1.3–5.4 | 1.4     | 0.8–2.5 | 0.5–3.1 |
| Northwest (1981–2010 normal: 18.2°C)             |         |         |          |         |         |         |         |         |         |         |         |         |
| CMIP5                                            | 5.8     | 4.5–7.2 | 3.5–7.9  | 3.6     | 3.0–4.5 | 1.7–5.3 | 2.6     | 1.9–4.2 | 1.2–4.4 | 1.7     | 1.0–2.4 | 0.4–2.9 |
| SMME                                             | 5.7     | 3.9–7.8 | 3.3–9.5  | 3.5     | 1.8–4.9 | 1.5–6.1 | 2.6     | 1.9–4.4 | 1.5–5.5 | 1.4     | 0.8–2.1 | 0.4–2.9 |
| MCPR                                             | 5.3     | 4.1–7.9 | 3.5–9.4  | 3.3     | 2.3–5.1 | 1.7–5.9 | 2.6     | 1.7–4.0 | 1.2–5.5 | 1.4     | 0.7–2.2 | 0.5–3.2 |
| California (1981–2010 normal: 23.7°C)            |         |         |          |         |         |         |         |         |         |         |         |         |
| CMIP5                                            | 4.7     | 4.0–5.7 | 3.6–6.4  | 2.9     | 2.4–4.0 | 1.2–4.8 | 2.4     | 1.9–3.1 | 1.7–3.8 | 1.3     | 0.9–2.0 | 0.4–2.8 |
| SMME                                             | 4.5     | 3.9–6.8 | 3.6–8.3  | 2.8     | 2.3–4.2 | 1.1–5.2 | 2.4     | 1.8–3.8 | 1.7–4.5 | 1.3     | 0.7–1.7 | 0.1–2.8 |
| MCPR                                             | 4.6     | 3.5–6.6 | 2.9–7.9  | 2.8     | 2.0–4.1 | 1.8–5.6 | 2.4     | 1.6–3.5 | 1.1–4.8 | 1.2     | 0.7–1.9 | 0.4–2.5 |
| Southwest (1981–2010 normal: 24.1°C)             |         |         |          |         |         |         |         |         |         |         |         |         |
| CMIP5                                            | 5.3     | 4.2–6.7 | 3.9–7.4  | 3.4     | 2.5–4.5 | 1.4–5.2 | 2.7     | 2.0–3.6 | 1.3–4.4 | 1.4     | 0.9–2.1 | 0.8–2.4 |
| SMME                                             | 5.0     | 4.2–7.2 | 4.0–9.1  | 3.2     | 2.2–4.5 | 1.3–5.2 | 2.4     | 1.8–4.0 | 1.5–4.9 | 1.4     | 0.9–1.9 | 0.6–2.9 |
| MCPR                                             | 4.9     | 3.7–7.2 | 3.0–8.8  | 3.1     | 2.3–4.3 | 2.0–5.8 | 2.5     | 1.6–3.8 | 1.3–5.1 | 1.4     | 0.7–2.2 | 0.2–2.9 |
| Rocky Mountain States (1981–2010 normal: 19.6°C) |         |         |          |         |         |         |         |         |         |         |         |         |
| CMIP5                                            | 5.8     | 4.7–7.7 | 3.9–8.0  | 3.5     | 2.8–4.8 | 1.6–5.3 | 2.8     | 2.0–4.0 | 1.4–4.7 | 1.5     | 0.8–2.1 | 0.4–2.8 |
| SMME                                             | 5.6     | 4.3–8.1 | 4.3–10.3 | 3.4     | 2.4–4.9 | 1.5–6.0 | 2.8     | 2.0–4.4 | 1.8–5.5 | 1.4     | 0.7–2.0 | 0.4–2.8 |
| MCPR                                             | 5.6     | 4.1–7.8 | 3.5–9.9  | 3.4     | 2.5–5.0 | 2.1–6.2 | 2.7     | 1.9–4.2 | 1.4–5.7 | 1.3     | 0.7–2.2 | 0.5–2.9 |
| Alaska (1981–2010 normal: 13.1°C)                |         |         |          |         |         |         |         |         |         |         |         |         |
| CMIP5                                            | 5.4     | 3.3–6.6 | 2.6–8.2  | 3.4     | 2.0–4.6 | 1.6–5.2 | 2.6     | 1.3–3.8 | 1.0–4.6 | 1.6     | 0.8–2.8 | 0.6–3.1 |
| SMME                                             | 4.7     | 2.6–7.7 | 2.2–9.3  | 3.3     | 1.9–4.6 | 1.6–5.2 | 2.3     | 1.2–4.3 | 1.0–5.7 | 1.3     | 0.8–2.7 | 0.6–3.6 |
| MCPR                                             | 4.6     | 3.4–7.4 | 2.7–9.4  | 2.8     | 2.0–4.8 | 1.6–6.2 | 2.5     | 1.4–3.4 | 1.1–4.1 | 1.5     | 0.5–2.5 | 0.2–3.5 |
| Hawaii (1981–2010 normal: 24.9°C)                |         |         |          |         |         |         |         |         |         |         |         |         |
| CMIP5                                            | 3.0     | 2.5–4.2 | 1.9–4.9  | 1.9     | 1.2–2.9 | 1.1–3.5 | 1.5     | 1.0–2.4 | 0.8–2.7 | 1.0     | 0.6–1.6 | 0.4–2.0 |
| SMME                                             | 2.9     | 1.9–4.4 | 1.7–5.3  | 1.6     | 1.2–2.9 | 1.1–3.8 | 1.4     | 1.0–2.4 | 0.8–3.0 | 0.7     | 0.4–1.4 | 0.4–2.0 |
| MCPR                                             | 2.9     | 2.3–4.3 | 2.0–5.5  | 1.8     | 1.4–2.7 | 1.1–3.5 | 1.5     | 0.9–2.3 | 0.7–3.1 | 0.8     | 0.5–1.4 | 0.3–2.1 |

TABLE A8. Projected number of days with maximum daily temperature greater than 35°C (population-weighted using county population) under all RCPs for 2080-2099

| 2080-2099                                           | RCP 8.5 |             |             | RCP 6.0 |             |             | RCP 4.5 |             |             | RCP 2.6 |             |             |
|-----------------------------------------------------|---------|-------------|-------------|---------|-------------|-------------|---------|-------------|-------------|---------|-------------|-------------|
|                                                     | 50      | 17-83       | 5-95        | 50      | 17-83       | 5-95        | 50      | 17-83       | 5-95        | 50      | 17-83       | 5-95        |
| CONUS (1981–2010 normal: 14.9 days)                 |         |             |             |         |             |             |         |             |             |         |             |             |
| CMIP5                                               | 70.8    | 58.3–90.2   | 45.7–96.9   | 44.7    | 41.0–59.7   | 28.1–66.9   | 39.0    | 28.6–51.5   | 24.7–57.2   | 26.7    | 22.3–33.6   | 21.4–36.4   |
| SMME                                                | 69.0    | 45.7–95.8   | 41.6–118.7  | 43.1    | 36.4–59.8   | 25.7–71.5   | 38.7    | 28.6–56.6   | 24.7–68.8   | 24.9    | 21.5–30.8   | 19.7–43.0   |
| MCPR                                                | 66.4    | 53.0–98.3   | 48.4–118.1  | 45.4    | 35.0–61.7   | 32.4–78.6   | 37.0    | 29.1–52.1   | 25.3–68.9   | 26.2    | 20.8–31.2   | 18.9–39.0   |
| Northeast (1981–2010 normal: 2.6 days)              |         |             |             |         |             |             |         |             |             |         |             |             |
| CMIP5                                               | 37.0    | 25.2–54.0   | 17.4–63.5   | 17.0    | 13.6–26.4   | 8.0–36.1    | 13.0    | 7.5–16.7    | 5.7–29.0    | 7.7     | 5.5–9.4     | 4.3–9.9     |
| SMME                                                | 37.0    | 17.4–59.5   | 9.8–83.0    | 17.0    | 10.1–29.6   | 7.9–36.4    | 12.7    | 6.7–25.1    | 5.7–35.3    | 7.1     | 5.5–9.0     | 3.6–13.8    |
| MCPR                                                | 34.1    | 22.3–61.6   | 18.3–83.6   | 17.7    | 11.3–28.3   | 9.8–42.3    | 11.9    | 8.0–20.8    | 6.1–35.3    | 5.9     | 4.2–10.1    | 3.5–12.6    |
| Southeast (1981–2010 normal: 8.2 days)              |         |             |             |         |             |             |         |             |             |         |             |             |
| CMIP5                                               | 88.4    | 73.1–115.1  | 53.9–122.3  | 52.7    | 44.0–75.9   | 30.7–85.8   | 43.2    | 27.8–57.7   | 21.2–69.1   | 25.3    | 18.6–33.6   | 17.0–36.4   |
| SMME                                                | 87.8    | 53.9–121.9  | 41.3–147.1  | 50.8    | 43.8–77.5   | 27.8–91.8   | 43.0    | 27.8–65.2   | 21.2–82.6   | 21.7    | 17.5–32.4   | 15.6–46.0   |
| MCPR                                                | 85.2    | 65.6–121.7  | 55.5–148.5  | 52.1    | 39.7–76.4   | 33.4–95.8   | 39.0    | 28.7–62.1   | 22.2–81.8   | 21.6    | 16.7–31.8   | 13.6–43.6   |
| South Central (1981–2010 normal: 35.7 days)         |         |             |             |         |             |             |         |             |             |         |             |             |
| CMIP5                                               | 126.5   | 107.6–144.6 | 95.3–148.0  | 98.2    | 85.6–111.6  | 63.0–121.6  | 84.6    | 65.5–98.6   | 51.9–115.1  | 62.7    | 53.5–74.9   | 49.1–77.4   |
| SMME                                                | 124.9   | 96.1–152.9  | 87.5–177.2  | 95.8    | 83.8–113.0  | 55.6–126.8  | 84.8    | 65.5–105.4  | 51.9–132.2  | 61.0    | 48.9–74.1   | 43.0–88.6   |
| MCPR                                                | 120.2   | 104.1–153.9 | 95.2–176.6  | 96.6    | 79.4–116.0  | 74.8–132.9  | 80.3    | 64.9–106.6  | 58.9–129.9  | 62.5    | 49.6–74.3   | 43.0–87.0   |
| Upper Great Plains (1981–2010 normal: 12.5 days)    |         |             |             |         |             |             |         |             |             |         |             |             |
| CMIP5                                               | 70.4    | 53.2–85.2   | 45.5–94.3   | 47.5    | 36.4–54.5   | 24.6–60.1   | 36.5    | 26.3–52.5   | 22.3–56.8   | 27.3    | 18.1–31.2   | 17.8–39.9   |
| SMME                                                | 70.4    | 47.1–95.8   | 41.8–111.0  | 45.2    | 33.8–58.0   | 23.6–67.8   | 35.7    | 26.6–56.6   | 23.9–72.9   | 23.6    | 17.9–30.8   | 17.2–42.8   |
| MCPR                                                | 66.8    | 51.0–89.4   | 46.1–112.8  | 45.8    | 33.8–60.8   | 28.2–73.6   | 35.2    | 28.1–48.5   | 22.7–69.7   | 24.6    | 18.7–33.4   | 16.1–42.9   |
| Midwest (1981–2010 normal: 2.7 days)                |         |             |             |         |             |             |         |             |             |         |             |             |
| CMIP5                                               | 48.5    | 31.6–73.8   | 22.4–82.6   | 24.6    | 16.8–38.9   | 10.9–45.0   | 16.3    | 9.7–33.5    | 7.9–41.8    | 10.3    | 6.6–17.2    | 5.1–21.8    |
| SMME                                                | 45.9    | 22.4–77.2   | 18.9–98.8   | 24.4    | 13.4–41.1   | 10.2–49.4   | 15.9    | 9.7–40.5    | 8.5–56.6    | 9.5     | 6.6–14.4    | 5.1–23.2    |
| MCPR                                                | 43.2    | 29.8–74.6   | 23.4–91.5   | 23.5    | 15.0–40.5   | 12.7–54.8   | 16.1    | 10.6–27.8   | 8.4–46.4    | 8.2     | 6.1–14.9    | 5.1–19.8    |
| Northwest (1981–2010 normal: 3.5 days)              |         |             |             |         |             |             |         |             |             |         |             |             |
| CMIP5                                               | 26.3    | 20.6–37.2   | 14.8–42.5   | 14.9    | 13.3–20.6   | 8.3–25.1    | 11.9    | 8.9–18.4    | 7.9–19.0    | 7.8     | 6.4–10.2    | 5.5–13.0    |
| SMME                                                | 24.8    | 18.6–40.9   | 12.8–53.4   | 14.9    | 10.7–20.7   | 7.4–25.1    | 11.8    | 8.8–18.7    | 8.4–25.4    | 7.5     | 6.2–9.9     | 4.7–13.3    |
| MCPR                                                | 25.0    | 18.4–39.3   | 13.4–52.7   | 14.4    | 10.7–24.6   | 8.7–30.2    | 11.4    | 8.8–17.1    | 6.6–28.3    | 7.3     | 5.3–9.9     | 4.7–13.1    |
| California (1981–2010 normal: 31.6 days)            |         |             |             |         |             |             |         |             |             |         |             |             |
| CMIP5                                               | 71.7    | 62.3–81.1   | 58.7–92.5   | 54.2    | 49.3–63.3   | 37.5–69.8   | 47.4    | 43.3–55.7   | 40.5–58.4   | 38.6    | 36.9–44.7   | 35.0–50.6   |
| SMME                                                | 71.7    | 59.0–94.1   | 54.7–116.1  | 52.6    | 46.0–65.1   | 33.9–74.8   | 47.6    | 43.8–57.5   | 42.2–69.5   | 38.1    | 35.3–43.6   | 29.6–52.3   |
| MCPR                                                | 68.9    | 57.7–94.1   | 50.9–117.2  | 51.8    | 45.0–65.2   | 42.1–78.9   | 48.3    | 41.9–59.8   | 37.9–75.3   | 39.0    | 35.4–44.5   | 32.6–49.1   |
| Southwest (1981–2010 normal: 92.0 days)             |         |             |             |         |             |             |         |             |             |         |             |             |
| CMIP5                                               | 155.7   | 145.7–169.6 | 135.8–184.1 | 132.5   | 129.5–143.5 | 111.6–153.0 | 124.8   | 116.1–134.1 | 108.5–144.2 | 111.4   | 105.6–118.3 | 104.4–123.9 |
| SMME                                                | 155.7   | 141.4–185.1 | 137.7–210.2 | 131.8   | 122.9–147.4 | 107.4–156.4 | 124.9   | 116.1–143.0 | 110.5–154.9 | 110.3   | 102.5–115.1 | 94.2–133.1  |
| MCPR                                                | 152.5   | 137.6–178.3 | 131.7–201.1 | 132.0   | 121.6–151.7 | 116.5–165.8 | 123.6   | 114.7–141.8 | 108.2–158.6 | 110.2   | 102.6–117.7 | 98.9–125.9  |
| Rocky Mountain States (1981–2010 normal: 23.0 days) |         |             |             |         |             |             |         |             |             |         |             |             |
| CMIP5                                               | 74.5    | 66.2–92.9   | 58.4–95.5   | 53.0    | 48.4–66.0   | 34.2–72.5   | 45.9    | 39.9–54.9   | 38.0–63.9   | 33.8    | 31.4–41.1   | 29.2–44.4   |
| SMME                                                | 73.7    | 64.5–95.6   | 58.4–115.5  | 52.0    | 47.3–67.0   | 31.0–72.5   | 45.9    | 41.4–61.0   | 38.8–76.4   | 33.7    | 30.3–39.7   | 24.8–48.4   |
| MCPR                                                | 71.3    | 58.5–95.8   | 53.4–113.8  | 52.8    | 43.5–66.5   | 39.5–80.4   | 46.5    | 38.5–63.2   | 35.2–71.3   | 34.0    | 30.0–40.9   | 27.2–45.8   |
| Alaska (1981–2010 normal: 0.0 days)                 |         |             |             |         |             |             |         |             |             |         |             |             |
| CMIP5                                               | 0.7     | 0.1–1.8     | 0.0–5.2     | 0.1     | 0.1–0.5     | 0.0–0.8     | 0.0     | 0.0–0.3     | 0.0–0.5     | 0.0     | 0.0–0.1     | 0.0–0.3     |
| SMME                                                | 0.5     | 0.0–3.5     | 0.0–6.4     | 0.1     | 0.1–0.6     | 0.0–0.8     | 0.0     | 0.0–0.3     | 0.0–0.5     | 0.0     | 0.0–0.1     | 0.0–0.3     |
| MCPR                                                | 0.5     | 0.2–2.8     | 0.1–7.9     | 0.1     | 0.1–0.6     | 0.0–1.5     | 0.1     | 0.0–0.2     | 0.0–0.5     | 0.0     | 0.0–0.1     | 0.0–0.3     |
| Hawaii (1981–2010 normal: 0.0 days)                 |         |             |             |         |             |             |         |             |             |         |             |             |
| CMIP5                                               | 19.3    | 5.8–71.3    | 1.7–97.0    | 1.2     | 0.2–10.7    | 0.2–27.5    | 0.5     | 0.1–3.2     | 0.0–10.3    | 0.1     | 0.0–0.3     | 0.0–1.0     |
| SMME                                                | 13.0    | 1.7–84.4    | 0.9–121.2   | 0.7     | 0.2–10.7    | 0.1–27.6    | 0.3     | 0.1–3.0     | 0.1–10.5    | 0.1     | 0.0–0.2     | 0.0–1.0     |
| MCPR                                                | 14.3    | 3.9–72.3    | 1.5–129.6   | 1.0     | 0.2–5.9     | 0.1–30.8    | 0.3     | 0.1–2.5     | 0.0–14.0    | 0.1     | 0.0–0.2     | 0.0–1.8     |

TABLE A9. Projected number of days with minimum daily temperature less than 0°C (population-weighted using county population) under all RCPs for 2080-2099. Note that ranges are presented as cool to warm.

| 2080-2099                                            | RCP 8.5 |             |            | RCP 6.0 |             |             | RCP 4.5 |             |             | RCP 2.6 |             |             |
|------------------------------------------------------|---------|-------------|------------|---------|-------------|-------------|---------|-------------|-------------|---------|-------------|-------------|
|                                                      | 50      | 83-17       | 95-5       | 50      | 83-17       | 95-5        | 50      | 83-17       | 95-5        | 50      | 83-17       | 95-5        |
| CONUS (1981–2010 normal: 74.1 days)                  |         |             |            |         |             |             |         |             |             |         |             |             |
| CMIP5                                                | 36.8    | 45.4–29.7   | 46.6–27.1  | 47.0    | 54.7–44.2   | 62.2–35.3   | 52.4    | 61.0–47.1   | 65.2–43.5   | 61.3    | 65.6–58.1   | 71.9–53.2   |
| SMME                                                 | 36.5    | 46.5–27.9   | 49.8–19.0  | 49.4    | 61.3–42.8   | 66.0–33.0   | 52.8    | 61.0–44.4   | 62.2–36.1   | 61.9    | 71.9–59.6   | 72.7–51.8   |
| MCPR                                                 | 39.1    | 48.1–26.6   | 51.3–15.3  | 49.6    | 57.8–40.2   | 61.3–31.2   | 56.1    | 60.6–45.4   | 64.9–36.0   | 65.0    | 69.5–57.2   | 71.4–51.8   |
| Northeast (1981–2010 normal: 102.9 days)             |         |             |            |         |             |             |         |             |             |         |             |             |
| CMIP5                                                | 49.9    | 61.8–39.9   | 63.7–35.4  | 66.4    | 77.0–61.6   | 88.1–47.0   | 72.0    | 84.9–65.3   | 89.3–59.9   | 85.4    | 91.2–80.4   | 102.9–73.7  |
| SMME                                                 | 49.9    | 63.6–32.1   | 68.7–23.0  | 67.6    | 84.1–57.4   | 93.3–43.2   | 72.2    | 84.2–61.2   | 87.3–52.1   | 87.8    | 102.9–81.2  | 103.5–69.8  |
| MCPR                                                 | 53.3    | 65.8–37.9   | 71.5–22.5  | 68.8    | 81.7–53.2   | 87.5–43.0   | 76.5    | 86.3–62.8   | 90.8–46.6   | 89.5    | 98.0–78.0   | 101.8–69.9  |
| Southeast (1981–2010 normal: 47.3 days)              |         |             |            |         |             |             |         |             |             |         |             |             |
| CMIP5                                                | 21.9    | 28.3–17.3   | 30.0–15.0  | 30.7    | 34.0–26.6   | 39.5–22.4   | 32.3    | 39.4–29.2   | 40.7–25.7   | 39.1    | 43.5–35.4   | 47.4–35.1   |
| SMME                                                 | 21.9    | 29.0–15.7   | 31.5–11.8  | 30.9    | 39.4–26.3   | 43.6–22.4   | 32.4    | 39.4–28.3   | 40.7–23.4   | 40.4    | 47.0–36.4   | 47.6–34.0   |
| MCPR                                                 | 23.1    | 29.8–14.3   | 33.3–8.7   | 31.1    | 37.3–23.4   | 39.7–18.8   | 34.3    | 39.7–26.2   | 40.8–17.5   | 41.0    | 44.7–35.7   | 48.7–32.5   |
| South Central (1981–2010 normal: 30.3 days)          |         |             |            |         |             |             |         |             |             |         |             |             |
| CMIP5                                                | 12.4    | 16.9–8.6    | 18.2–8.0   | 19.7    | 20.8–14.8   | 25.6–13.2   | 20.9    | 25.2–18.1   | 27.6–15.8   | 25.5    | 28.6–22.2   | 30.9–21.9   |
| SMME                                                 | 12.6    | 18.0–8.3    | 19.3–6.5   | 20.1    | 25.6–14.4   | 27.9–11.5   | 21.1    | 25.5–17.4   | 26.9–11.6   | 26.4    | 30.8–22.6   | 32.3–21.3   |
| MCPR                                                 | 13.5    | 17.9–8.0    | 19.9–3.1   | 19.3    | 22.7–13.8   | 24.2–11.6   | 22.1    | 25.4–16.1   | 28.1–12.3   | 27.4    | 30.0–23.3   | 32.9–20.6   |
| Upper Great Plains (1981–2010 normal: 130.6 days)    |         |             |            |         |             |             |         |             |             |         |             |             |
| CMIP5                                                | 82.1    | 93.5–66.5   | 102.8–59.6 | 97.4    | 107.6–91.5  | 116.6–81.6  | 105.2   | 114.7–96.7  | 120.3–87.2  | 115.5   | 122.4–109.6 | 125.1–106.0 |
| SMME                                                 | 81.2    | 98.4–61.7   | 102.8–55.8 | 97.8    | 114.9–88.3  | 118.6–69.0  | 105.2   | 114.5–89.8  | 118.0–71.9  | 119.6   | 126.0–109.7 | 126.7–105.2 |
| MCPR                                                 | 86.2    | 99.2–66.1   | 104.2–37.9 | 100.5   | 112.6–88.2  | 115.9–78.2  | 108.5   | 116.0–94.9  | 120.4–82.7  | 119.2   | 125.9–110.8 | 127.8–101.8 |
| Midwest (1981–2010 normal: 122.4 days)               |         |             |            |         |             |             |         |             |             |         |             |             |
| CMIP5                                                | 67.3    | 79.1–55.3   | 84.2–49.2  | 84.9    | 97.2–75.7   | 107.4–60.6  | 92.6    | 102.6–79.4  | 110.7–73.6  | 103.8   | 110.3–99.0  | 117.8–90.9  |
| SMME                                                 | 66.9    | 82.9–50.2   | 85.8–34.2  | 85.0    | 102.7–74.9  | 112.0–56.4  | 92.8    | 102.6–76.4  | 105.4–58.9  | 106.9   | 118.8–99.6  | 120.4–88.4  |
| MCPR                                                 | 72.5    | 86.0–50.4   | 90.2–28.0  | 86.9    | 99.6–70.3   | 105.5–57.2  | 96.7    | 103.6–79.4  | 110.3–64.2  | 108.9   | 115.6–97.3  | 118.6–88.8  |
| Northwest (1981–2010 normal: 63.3 days)              |         |             |            |         |             |             |         |             |             |         |             |             |
| CMIP5                                                | 18.8    | 26.5–13.7   | 30.7–10.6  | 29.8    | 39.8–21.0   | 44.8–19.0   | 33.9    | 45.3–27.8   | 49.5–23.3   | 42.6    | 50.5–34.4   | 51.0–32.6   |
| SMME                                                 | 19.6    | 30.7–12.5   | 35.5–7.7   | 31.4    | 43.0–20.5   | 44.8–16.5   | 34.4    | 48.5–23.9   | 49.5–16.8   | 45.2    | 53.7–36.2   | 62.9–26.8   |
| MCPR                                                 | 21.3    | 28.7–11.7   | 32.7–7.0   | 31.0    | 40.4–21.3   | 44.0–16.2   | 36.7    | 47.2–26.5   | 52.2–13.5   | 43.9    | 54.2–35.9   | 57.8–25.1   |
| California (1981–2010 normal: 15.8 days)             |         |             |            |         |             |             |         |             |             |         |             |             |
| CMIP5                                                | 3.6     | 5.2–2.2     | 6.7–1.5    | 6.5     | 8.8–4.4     | 10.4–3.5    | 8.0     | 10.7–6.5    | 14.3–5.8    | 10.6    | 13.1–9.0    | 13.8–7.9    |
| SMME                                                 | 3.6     | 6.7–2.0     | 7.4–1.2    | 7.4     | 10.4–4.4    | 12.0–3.5    | 9.0     | 11.1–6.0    | 12.1–4.0    | 12.1    | 14.5–9.4    | 15.7–6.8    |
| MCPR                                                 | 3.8     | 6.0–2.0     | 7.2–0.9    | 7.0     | 9.4–4.4     | 10.6–3.3    | 8.9     | 11.5–6.2    | 13.2–4.6    | 11.9    | 14.1–9.2    | 15.8–6.8    |
| Southwest (1981–2010 normal: 47.4 days)              |         |             |            |         |             |             |         |             |             |         |             |             |
| CMIP5                                                | 22.0    | 26.6–18.1   | 29.6–15.7  | 30.3    | 34.1–25.3   | 38.1–23.4   | 33.5    | 38.5–29.6   | 41.5–27.4   | 39.1    | 43.1–35.5   | 44.0–32.8   |
| SMME                                                 | 21.4    | 29.6–15.9   | 33.2–12.6  | 31.7    | 35.4–24.0   | 40.5–21.0   | 33.7    | 38.5–27.7   | 39.3–25.1   | 41.0    | 44.1–37.0   | 44.7–32.5   |
| MCPR                                                 | 23.4    | 29.2–16.2   | 32.3–10.8  | 31.3    | 35.8–25.5   | 37.8–21.3   | 35.0    | 39.5–29.0   | 41.5–24.4   | 41.3    | 44.4–36.7   | 45.1–32.3   |
| Rocky Mountain States (1981–2010 normal: 133.9 days) |         |             |            |         |             |             |         |             |             |         |             |             |
| CMIP5                                                | 71.5    | 83.2–60.3   | 92.4–54.5  | 89.8    | 100.8–78.3  | 111.1–71.3  | 95.8    | 110.6–89.5  | 116.0–80.2  | 111.3   | 118.7–102.4 | 124.1–92.5  |
| SMME                                                 | 71.5    | 92.4–54.5   | 96.7–44.7  | 93.5    | 108.5–75.3  | 116.5–66.4  | 97.6    | 114.9–82.2  | 116.0–67.3  | 115.7   | 123.5–103.2 | 125.1–92.0  |
| MCPR                                                 | 77.7    | 90.8–56.5   | 98.5–37.7  | 95.6    | 104.9–78.8  | 110.2–69.8  | 104.1   | 113.5–87.9  | 118.4–73.6  | 116.1   | 121.6–103.6 | 124.4–95.1  |
| Alaska (1981–2010 normal: 187.7 days)                |         |             |            |         |             |             |         |             |             |         |             |             |
| CMIP5                                                | 113.5   | 126.4–102.0 | 149.3–88.6 | 138.0   | 149.9–132.7 | 163.0–123.8 | 147.4   | 165.2–137.3 | 171.8–130.3 | 158.6   | 171.4–152.1 | 177.9–143.9 |
| SMME                                                 | 117.4   | 133.5–93.9  | 151.3–83.8 | 141.7   | 156.1–125.7 | 163.0–121.0 | 148.8   | 165.7–132.4 | 171.8–121.0 | 162.5   | 171.7–152.6 | 179.1–143.9 |
| MCPR                                                 | 119.4   | 139.1–98.6  | 145.0–67.7 | 141.9   | 158.0–127.7 | 165.8–115.6 | 150.8   | 164.5–134.4 | 175.9–113.6 | 164.5   | 175.9–149.5 | 181.3–135.6 |
| Hawaii (1981–2010 normal: 0.0 days)                  |         |             |            |         |             |             |         |             |             |         |             |             |
| CMIP5                                                | 0.0     | 0.0–0.0     | 0.0–0.0    | 0.0     | 0.0–0.0     | 0.0–0.0     | 0.0     | 0.0–0.0     | 0.0–0.0     | 0.0     | 0.0–0.0     | 0.0–0.0     |
| SMME                                                 | 0.0     | 0.0–0.0     | 0.0–0.0    | 0.0     | 0.0–0.0     | 0.0–0.0     | 0.0     | 0.0–0.0     | 0.0–0.0     | 0.0     | 0.0–0.0     | 0.0–0.0     |
| MCPR                                                 | 0.0     | 0.0–0.0     | 0.0–0.0    | 0.0     | 0.0–0.0     | 0.0–0.0     | 0.0     | 0.0–0.0     | 0.0–0.0     | 0.0     | 0.0–0.0     | 0.0–0.0     |

TABLE A10. Projected regional DJF precipitation change (%) under all RCPs for 2080-2099

| DJF<br>2080-2099                                 | RCP 8.5 |            |            | RCP 6.0 |            |            | RCP 4.5 |            |            | RCP 2.6 |            |            |
|--------------------------------------------------|---------|------------|------------|---------|------------|------------|---------|------------|------------|---------|------------|------------|
|                                                  | 50      | 17-83      | 5-95       | 50      | 17-83      | 5-95       | 50      | 17-83      | 5-95       | 50      | 17-83      | 5-95       |
| CONUS (1981-2010 normal: 159.7mm)                |         |            |            |         |            |            |         |            |            |         |            |            |
| CMIP5                                            | 11.2    | 1.6-24.2   | -9.5-29.2  | 4.0     | -1.6-11.3  | -4.7-17.1  | 5.7     | -1.3-13.5  | -5.2-15.5  | 2.1     | -3.9-6.1   | -5.0-7.7   |
| SMME                                             | 7.3     | -1.4-21.4  | -1.7-25.6  | 2.5     | -1.7-11.3  | -4.5-14.5  | 3.6     | -1.8-13.1  | -4.6-15.0  | 0.1     | -2.5-5.5   | -5.0-7.7   |
| MCPR                                             | 13.4    | 2.1-27.0   | -4.6-38.6  | 8.2     | -0.0-15.6  | -3.0-19.8  | 6.1     | 0.2-13.7   | -4.8-20.2  | 3.8     | -3.2-10.0  | -9.4-13.9  |
| Northeast (1981-2010 normal: 228.4mm)            |         |            |            |         |            |            |         |            |            |         |            |            |
| CMIP5                                            | 23.3    | 8.6-33.9   | 1.7-44.4   | 11.2    | 5.1-22.7   | -1.8-24.9  | 13.8    | 0.0-26.5   | -4.7-30.0  | 2.6     | -2.6-9.8   | -3.9-13.9  |
| SMME                                             | 15.8    | -0.8-33.0  | -1.8-37.8  | 10.7    | -1.5-21.2  | -1.9-23.8  | 9.4     | -1.8-22.9  | -4.7-28.2  | 1.4     | -2.4-7.3   | -3.9-12.4  |
| MCPR                                             | 20.1    | 5.3-39.4   | 0.9-54.3   | 15.4    | 5.3-23.7   | -0.4-36.7  | 13.0    | 4.9-25.2   | -4.5-32.7  | 5.6     | -3.4-12.9  | -16.0-16.9 |
| Southeast (1981-2010 normal: 315.1mm)            |         |            |            |         |            |            |         |            |            |         |            |            |
| CMIP5                                            | 5.8     | -5.2-26.0  | -19.8-36.8 | -0.9    | -6.7-7.8   | -22.3-17.6 | 6.0     | -5.9-13.9  | -12.9-16.9 | 0.6     | -5.6-6.8   | -8.4-8.5   |
| SMME                                             | -0.5    | -2.5-17.6  | -13.8-35.5 | -1.3    | -4.8-7.8   | -10.9-10.4 | 0.1     | -4.5-12.7  | -12.9-15.4 | -0.2    | -5.2-6.8   | -8.4-8.5   |
| MCPR                                             | 6.2     | -7.3-22.0  | -19.8-35.7 | 3.5     | -3.0-13.2  | -10.8-18.9 | 5.2     | -6.7-12.8  | -12.8-23.6 | 1.0     | -6.8-7.8   | -15.3-13.3 |
| South Central (1981-2010 normal: 184.7mm)        |         |            |            |         |            |            |         |            |            |         |            |            |
| CMIP5                                            | -2.5    | -17.1-15.3 | -36.4-28.5 | -5.8    | -14.9-6.5  | -31.5-13.0 | 1.4     | -12.2-7.2  | -17.7-13.6 | -2.2    | -10.1-9.3  | -15.1-13.6 |
| SMME                                             | -1.5    | -12.5-8.7  | -22.5-24.6 | -1.8    | -11.0-6.5  | -16.6-13.0 | -2.0    | -8.3-6.4   | -15.3-11.1 | -2.2    | -8.6-8.2   | -15.1-13.6 |
| MCPR                                             | -1.7    | -16.3-14.3 | -30.0-24.4 | 0.4     | -8.8-12.2  | -17.7-16.6 | -1.5    | -14.2-8.8  | -22.7-20.4 | 0.6     | -10.0-9.5  | -16.2-13.8 |
| Upper Great Plains (1981-2010 normal: 47.6mm)    |         |            |            |         |            |            |         |            |            |         |            |            |
| CMIP5                                            | 23.8    | 11.1-44.4  | 0.8-67.5   | 10.7    | 0.5-23.6   | -6.3-43.8  | 12.7    | 2.4-22.0   | -9.5-27.8  | 5.1     | -3.2-20.6  | -8.8-25.2  |
| SMME                                             | 20.3    | -0.3-37.8  | -1.3-51.7  | 9.4     | -1.7-20.6  | -4.8-41.4  | 10.6    | -1.0-19.8  | -5.4-26.6  | 0.2     | -1.9-13.4  | -8.8-25.2  |
| MCPR                                             | 25.7    | 7.7-47.7   | -2.7-73.0  | 13.8    | -0.8-28.0  | -8.3-37.1  | 11.4    | -1.3-22.6  | -12.0-35.4 | 9.6     | -6.0-22.5  | -14.0-28.8 |
| Midwest (1981-2010 normal: 135.0mm)              |         |            |            |         |            |            |         |            |            |         |            |            |
| CMIP5                                            | 21.7    | 10.1-35.1  | -11.1-39.8 | 13.2    | -0.6-20.9  | -15.1-26.4 | 10.0    | -1.5-17.4  | -5.7-35.5  | 2.8     | -4.1-11.9  | -10.1-17.9 |
| SMME                                             | 17.0    | -0.5-32.3  | -1.4-35.5  | 5.3     | -1.8-20.9  | -5.2-22.6  | 6.6     | -1.6-16.5  | -4.0-30.9  | -1.2    | -3.1-9.7   | -10.1-17.9 |
| MCPR                                             | 20.7    | 6.5-41.8   | -6.3-54.9  | 12.6    | 1.2-26.4   | -13.9-35.2 | 11.3    | 0.7-23.2   | -2.5-34.5  | 5.4     | -5.2-15.0  | -12.6-24.2 |
| Northwest (1981-2010 normal: 300.4mm)            |         |            |            |         |            |            |         |            |            |         |            |            |
| CMIP5                                            | 11.1    | -5.2-22.9  | -15.7-40.5 | 9.6     | 2.5-19.9   | -8.7-25.1  | 6.1     | -4.0-18.1  | -8.7-23.9  | 0.4     | -5.7-12.9  | -8.0-14.9  |
| SMME                                             | 3.2     | -2.3-22.9  | -10.5-40.5 | 8.8     | -1.8-19.9  | -8.7-22.9  | 5.3     | -1.9-16.6  | -8.3-20.2  | -1.6    | -4.1-8.2   | -8.0-14.9  |
| MCPR                                             | 14.4    | -2.5-25.9  | -18.0-43.0 | 11.4    | -0.9-21.9  | -8.2-37.2  | 7.9     | -2.2-21.8  | -10.5-37.8 | 3.5     | -7.6-11.4  | -13.5-19.8 |
| California (1981-2010 normal: 274.8mm)           |         |            |            |         |            |            |         |            |            |         |            |            |
| CMIP5                                            | 10.8    | -4.6-38.2  | -26.4-65.5 | 8.9     | -9.0-20.3  | -28.0-40.7 | 4.2     | -12.1-28.9 | -24.1-36.8 | 0.4     | -15.1-11.8 | -17.9-15.0 |
| SMME                                             | 1.1     | -2.9-32.7  | -26.4-59.6 | 1.5     | -7.3-20.3  | -22.6-33.0 | -0.6    | -9.4-22.6  | -17.1-30.5 | -0.5    | -8.9-11.7  | -17.9-15.0 |
| MCPR                                             | 20.2    | -2.5-42.5  | -12.6-59.9 | 8.9     | -13.9-29.4 | -30.9-38.0 | 4.8     | -16.9-28.6 | -27.5-37.8 | 9.4     | -8.1-23.9  | -28.1-30.2 |
| Southwest (1981-2010 normal: 62.9mm)             |         |            |            |         |            |            |         |            |            |         |            |            |
| CMIP5                                            | 1.1     | -22.9-21.3 | -31.9-33.7 | -7.6    | -26.9-9.2  | -39.8-18.3 | -7.6    | -26.3-12.4 | -32.0-26.3 | -4.9    | -13.7-9.0  | -25.1-14.8 |
| SMME                                             | -0.9    | -21.7-14.6 | -31.9-33.7 | -2.6    | -20.8-9.2  | -35.3-18.3 | -2.9    | -24.8-8.7  | -31.7-17.3 | -1.6    | -10.3-9.0  | -16.2-14.8 |
| MCPR                                             | 0.8     | -17.3-29.9 | -41.9-43.9 | 6.5     | -31.8-23.3 | -45.5-38.5 | -4.1    | -27.1-18.4 | -50.5-36.2 | 3.3     | -14.3-23.0 | -22.7-33.9 |
| Rocky Mountain States (1981-2010 normal: 62.6mm) |         |            |            |         |            |            |         |            |            |         |            |            |
| CMIP5                                            | 30.5    | 15.0-50.2  | -12.6-63.5 | 15.3    | 5.8-25.9   | -8.7-35.0  | 14.4    | 0.6-26.0   | -10.2-36.6 | 1.9     | -3.0-15.8  | -5.6-18.1  |
| SMME                                             | 19.9    | -1.3-48.2  | -1.6-62.3  | 13.0    | -1.2-25.9  | -2.1-29.4  | 10.5    | -1.7-23.8  | -5.4-32.7  | 1.2     | -2.2-11.3  | -5.6-18.1  |
| MCPR                                             | 33.9    | 14.5-59.6  | -3.0-83.4  | 18.5    | 2.7-36.7   | -16.7-51.8 | 17.4    | -0.8-33.2  | -12.2-49.7 | 9.9     | -5.0-21.7  | -13.6-33.8 |
| Alaska (1981-2010 normal: 105.8mm)               |         |            |            |         |            |            |         |            |            |         |            |            |
| CMIP5                                            | 30.6    | 15.0-42.1  | 5.6-65.2   | 16.6    | 5.4-28.6   | 1.3-50.2   | 12.3    | 4.2-26.2   | -2.3-34.4  | 6.4     | -2.4-21.1  | -3.4-24.2  |
| SMME                                             | 15.5    | 0.3-40.4   | -1.4-65.2  | 14.3    | -0.8-22.0  | -1.5-29.4  | 7.8     | -0.6-20.7  | -1.8-32.5  | -0.8    | -1.8-17.5  | -3.4-24.2  |
| MCPR                                             | 24.3    | 11.7-41.6  | 6.7-57.2   | 15.3    | 6.4-27.0   | 0.5-33.9   | 11.4    | 2.4-22.2   | -4.0-28.2  | 5.8     | -1.0-14.3  | -6.7-19.0  |
| Hawaii (1981-2010 normal: 601.1mm)               |         |            |            |         |            |            |         |            |            |         |            |            |
| CMIP5                                            | -3.9    | -13.8-8.4  | -28.3-28.0 | -5.5    | -18.1-1.6  | -35.8-4.5  | -4.8    | -20.6-3.7  | -27.9-12.5 | -7.0    | -10.7-7.3  | -17.5-10.9 |
| SMME                                             | -3.1    | -13.0-6.7  | -28.3-16.4 | -3.5    | -18.1-1.6  | -29.9-4.1  | -3.3    | -11.8-2.5  | -24.2-8.9  | -2.6    | -9.5-2.8   | -17.5-10.9 |
| MCPR                                             | -4.7    | -21.5-10.1 | -29.4-19.3 | -4.8    | -20.4-5.1  | -30.0-11.7 | -4.8    | -15.7-8.6  | -28.0-17.9 | -0.2    | -13.5-8.3  | -23.8-15.3 |

TABLE A11. Projected regional MAM precipitation change (%) under all RCPs for 2080-2099

| MAM<br>2080-2099                                 | RCP 8.5 |            |            | RCP 6.0 |            |            | RCP 4.5 |            |            | RCP 2.6 |            |            |
|--------------------------------------------------|---------|------------|------------|---------|------------|------------|---------|------------|------------|---------|------------|------------|
|                                                  | 50      | 17-83      | 5-95       | 50      | 17-83      | 5-95       | 50      | 17-83      | 5-95       | 50      | 17-83      | 5-95       |
| CONUS (1981–2010 normal: 196.1mm)                |         |            |            |         |            |            |         |            |            |         |            |            |
| CMIP5                                            | 10.7    | 2.2–17.6   | -5.0–22.2  | 8.2     | 3.5–17.2   | -1.2–21.7  | 8.3     | 0.1–13.7   | -2.8–18.3  | 6.5     | 2.4–15.1   | 0.6–22.0   |
| SMME                                             | 7.0     | 0.7–15.8   | -3.3–18.7  | 4.1     | 0.4–12.2   | 0.1–20.1   | 4.9     | 0.1–10.9   | -2.8–17.0  | 3.2     | 0.2–10.3   | -0.0–22.0  |
| MCPR                                             | 13.0    | 3.5–23.1   | -5.5–32.6  | 10.1    | 2.4–19.9   | -1.3–26.0  | 7.7     | 1.1–16.4   | -2.5–21.5  | 4.9     | -0.0–13.9  | -3.1–19.0  |
| Northeast (1981–2010 normal: 277.5mm)            |         |            |            |         |            |            |         |            |            |         |            |            |
| CMIP5                                            | 15.7    | 10.5–24.5  | 5.9–32.7   | 16.1    | 8.1–19.8   | 5.5–24.5   | 9.3     | 1.3–15.8   | -3.7–22.5  | 7.7     | 3.7–20.6   | -3.6–21.2  |
| SMME                                             | 12.9    | 1.0–23.4   | 0.4–30.3   | 8.1     | 0.7–19.1   | 0.2–23.0   | 7.1     | 0.4–14.0   | -3.7–22.4  | 5.7     | -0.1–12.2  | -3.6–21.2  |
| MCPR                                             | 17.4    | 8.7–29.8   | 2.4–38.0   | 15.3    | 9.2–22.4   | 3.0–30.6   | 10.4    | 1.7–18.6   | -4.8–26.8  | 6.5     | -2.9–15.1  | -10.0–24.4 |
| Southeast (1981–2010 normal: 318.6mm)            |         |            |            |         |            |            |         |            |            |         |            |            |
| CMIP5                                            | 7.4     | -7.0–19.3  | -16.8–32.2 | 6.2     | -3.0–16.0  | -8.1–21.0  | 4.7     | -2.0–19.3  | -5.6–26.9  | 9.0     | 0.4–18.2   | -5.3–29.6  |
| SMME                                             | 1.6     | -2.9–19.3  | -16.8–25.3 | 0.5     | -3.0–16.0  | -6.9–19.2  | 2.7     | -2.1–13.2  | -5.6–25.8  | 1.3     | 0.3–16.1   | -5.3–29.6  |
| MCPR                                             | 9.8     | -7.2–26.1  | -17.8–35.1 | 8.4     | -1.2–20.5  | -14.1–26.8 | 8.0     | -1.9–18.4  | -9.2–29.8  | 5.8     | -4.5–18.4  | -9.3–28.3  |
| South Central (1981–2010 normal: 242.6mm)        |         |            |            |         |            |            |         |            |            |         |            |            |
| CMIP5                                            | -3.1    | -12.2–8.0  | -21.4–15.3 | 0.4     | -8.9–9.3   | -14.7–12.4 | 0.8     | -7.2–8.9   | -14.7–13.9 | 2.2     | -2.2–13.5  | -3.3–20.8  |
| SMME                                             | 0.0     | -9.3–4.7   | -14.3–15.3 | 0.2     | -8.9–7.2   | -10.8–12.4 | -0.4    | -6.5–7.7   | -8.2–13.3  | 1.5     | -1.7–8.6   | -3.3–20.8  |
| MCPR                                             | 1.1     | -13.2–14.7 | -23.3–24.6 | -0.7    | -15.2–11.6 | -23.9–16.8 | 1.6     | -8.5–12.5  | -15.3–21.8 | 4.1     | -6.8–17.6  | -15.3–25.3 |
| Upper Great Plains (1981–2010 normal: 176.6mm)   |         |            |            |         |            |            |         |            |            |         |            |            |
| CMIP5                                            | 20.3    | 6.5–31.7   | 0.1–43.6   | 13.3    | 6.8–30.9   | -0.3–43.7  | 13.9    | 3.5–21.0   | -2.8–31.8  | 6.5     | 3.7–14.4   | -6.3–21.5  |
| SMME                                             | 13.8    | 1.8–29.6   | 1.0–40.5   | 11.7    | 0.9–20.4   | 0.4–33.2   | 7.1     | 0.1–19.1   | -1.9–28.5  | 5.5     | 0.4–12.8   | -6.3–21.5  |
| MCPR                                             | 22.6    | 9.7–38.1   | -1.8–61.9  | 16.6    | 4.4–27.6   | -3.5–42.9  | 13.9    | 3.7–26.1   | -2.9–35.2  | 6.8     | -3.5–17.2  | -10.4–23.8 |
| Midwest (1981–2010 normal: 250.7mm)              |         |            |            |         |            |            |         |            |            |         |            |            |
| CMIP5                                            | 20.5    | 11.7–30.7  | 7.2–36.7   | 12.9    | 10.3–21.5  | 0.7–38.8   | 9.5     | 1.4–20.6   | -3.0–25.7  | 6.2     | 2.7–13.9   | 1.2–19.5   |
| SMME                                             | 16.0    | 1.4–28.6   | 0.8–36.7   | 11.5    | 0.7–21.3   | 0.3–21.8   | 7.8     | 0.2–16.2   | -3.0–23.8  | 6.1     | 0.2–9.6    | -0.0–19.5  |
| MCPR                                             | 20.4    | 12.3–32.5  | 6.7–53.1   | 14.0    | 5.1–28.0   | -1.8–38.5  | 12.9    | 1.1–22.2   | -3.5–33.7  | 4.7     | -1.6–13.2  | -3.5–20.3  |
| Northwest (1981–2010 normal: 192.2mm)            |         |            |            |         |            |            |         |            |            |         |            |            |
| CMIP5                                            | 2.7     | -3.3–11.9  | -9.9–16.0  | 3.6     | -2.4–15.2  | -10.4–23.5 | 2.4     | -5.3–14.1  | -11.1–18.0 | 5.2     | -3.9–13.5  | -6.9–14.7  |
| SMME                                             | 1.4     | -0.5–11.7  | -6.7–15.4  | 1.5     | -2.4–9.3   | -8.2–18.9  | 0.4     | -3.8–13.2  | -9.9–18.0  | 0.1     | -3.0–8.4   | -6.9–14.7  |
| MCPR                                             | 3.4     | -7.8–16.1  | -14.5–35.7 | 5.2     | -6.2–16.9  | -13.5–39.0 | 7.0     | -6.4–18.7  | -14.5–25.2 | 0.9     | -9.9–11.6  | -16.4–26.1 |
| California (1981–2010 normal: 137.4mm)           |         |            |            |         |            |            |         |            |            |         |            |            |
| CMIP5                                            | -9.4    | -27.6–2.3  | -35.4–12.1 | -0.6    | -20.1–12.5 | -26.6–21.5 | -6.4    | -18.0–11.9 | -25.0–18.6 | 1.9     | -11.8–23.9 | -14.2–30.3 |
| SMME                                             | -3.8    | -25.8–0.6  | -35.4–10.9 | -0.5    | -7.7–10.3  | -26.6–17.3 | -1.4    | -17.9–8.4  | -23.5–18.2 | -0.5    | -12.2–13.4 | -14.2–30.3 |
| MCPR                                             | -8.1    | -25.3–15.3 | -37.5–28.4 | 2.2     | -24.7–18.7 | -35.8–27.5 | -6.0    | -23.1–21.0 | -34.0–31.3 | 1.4     | -15.5–21.5 | -30.1–38.7 |
| Southwest (1981–2010 normal: 51.2mm)             |         |            |            |         |            |            |         |            |            |         |            |            |
| CMIP5                                            | -23.0   | -38.6–9.9  | -44.8–9.0  | -14.8   | -22.7–4.7  | -27.8–15.6 | -7.5    | -18.2–2.1  | -32.1–10.8 | 8.4     | -6.4–19.2  | -21.6–26.3 |
| SMME                                             | -15.9   | -34.7–0.9  | -40.3–0.5  | -11.5   | -22.7–0.7  | -24.6–11.5 | -5.6    | -15.1–0.3  | -26.9–7.6  | 0.6     | -6.0–14.6  | -21.6–25.4 |
| MCPR                                             | -18.3   | -38.9–5.7  | -58.5–7.0  | -10.4   | -32.8–1.2  | -50.0–18.6 | -9.2    | -29.8–6.6  | -41.5–16.3 | 7.4     | -17.0–22.4 | -29.6–38.7 |
| Rocky Mountain States (1981–2010 normal: 98.7mm) |         |            |            |         |            |            |         |            |            |         |            |            |
| CMIP5                                            | 14.8    | 6.8–29.8   | -8.1–47.0  | 16.0    | 9.3–42.1   | -0.0–66.2  | 12.5    | -3.2–24.7  | -7.4–40.1  | 11.6    | 2.2–25.1   | -2.6–41.5  |
| SMME                                             | 11.6    | 1.1–24.7   | -3.2–44.8  | 12.9    | 0.7–21.5   | 0.0–49.5   | 4.9     | -0.3–21.5  | -7.4–29.0  | 9.2     | 0.0–21.7   | -2.6–41.5  |
| MCPR                                             | 20.2    | 3.2–36.8   | -1.8–58.2  | 21.8    | 7.2–47.4   | -4.2–67.7  | 12.1    | 0.8–29.9   | -8.8–52.5  | 8.8     | -2.0–26.6  | -9.4–40.6  |
| Alaska (1981–2010 normal: 80.7mm)                |         |            |            |         |            |            |         |            |            |         |            |            |
| CMIP5                                            | 38.6    | 23.0–53.9  | 9.3–70.9   | 18.1    | 12.3–24.8  | 1.2–38.2   | 18.2    | 3.5–28.0   | -1.2–37.2  | 10.4    | 1.2–21.5   | -3.9–23.4  |
| SMME                                             | 35.6    | 1.6–52.0   | 1.1–60.7   | 16.1    | 1.1–20.5   | 0.3–25.6   | 14.3    | 1.0–25.7   | 0.6–36.6   | 7.2     | 0.4–16.0   | -3.9–23.4  |
| MCPR                                             | 33.1    | 16.8–51.8  | 7.5–71.7   | 15.8    | 7.7–22.4   | 0.1–32.4   | 11.8    | 3.7–24.7   | -3.2–42.0  | 8.6     | -5.2–18.9  | -13.3–25.7 |
| Hawaii (1981–2010 normal: 586.1mm)               |         |            |            |         |            |            |         |            |            |         |            |            |
| CMIP5                                            | -4.2    | -23.8–19.8 | -34.7–32.7 | -10.2   | -22.3–6.6  | -30.6–24.3 | -1.5    | -16.8–11.3 | -27.1–24.0 | -1.7    | -13.0–12.2 | -20.1–31.7 |
| SMME                                             | -0.9    | -21.3–8.9  | -34.7–25.5 | -4.9    | -22.3–5.8  | -29.4–16.9 | -0.8    | -11.8–11.3 | -24.0–18.9 | -0.2    | -13.0–12.2 | -20.1–31.7 |
| MCPR                                             | -4.4    | -20.3–16.7 | -28.3–25.4 | -5.1    | -20.2–11.9 | -29.2–23.9 | -0.4    | -14.6–12.4 | -21.6–22.0 | 0.5     | -9.7–17.6  | -16.9–24.7 |

TABLE A12. Projected regional SON precipitation change (%) under all RCPs for 2080-2099

| SON<br>2080-2099                                 | RCP 8.5 |            |            | RCP 6.0 |            |            | RCP 4.5 |            |            | RCP 2.6 |            |            |
|--------------------------------------------------|---------|------------|------------|---------|------------|------------|---------|------------|------------|---------|------------|------------|
|                                                  | 50      | 17-83      | 5-95       | 50      | 17-83      | 5-95       | 50      | 17-83      | 5-95       | 50      | 17-83      | 5-95       |
| CONUS (1981–2010 normal: 182.0mm)                |         |            |            |         |            |            |         |            |            |         |            |            |
| CMIP5                                            | 5.8     | -1.9–10.9  | -7.0–19.9  | 3.5     | -2.2–9.5   | -9.8–22.5  | 3.6     | -2.4–9.9   | -6.6–12.8  | 1.9     | -3.0–9.3   | -4.2–10.1  |
| SMME                                             | 3.3     | -0.1–8.9   | -7.0–18.8  | 0.5     | -2.2–9.5   | -9.8–11.8  | 2.4     | -2.4–8.7   | -4.7–11.6  | 0.6     | -2.5–4.1   | -4.2–10.1  |
| MCPR                                             | 5.7     | 1.3–13.3   | -6.8–19.1  | 4.7     | -2.3–9.7   | -6.8–14.1  | 5.2     | -1.1–11.4  | -4.7–19.3  | 1.3     | -4.7–7.5   | -8.4–13.7  |
| Northeast (1981–2010 normal: 288.2mm)            |         |            |            |         |            |            |         |            |            |         |            |            |
| CMIP5                                            | 6.9     | -0.6–13.5  | -9.0–15.9  | 5.3     | -5.8–11.3  | -11.8–18.3 | 5.2     | -5.0–9.3   | -8.0–13.6  | 0.2     | -6.9–8.5   | -8.7–12.2  |
| SMME                                             | 3.1     | -0.2–12.0  | -9.0–13.9  | 0.8     | -5.8–8.0   | -11.8–18.3 | 1.0     | -5.0–7.9   | -7.5–12.0  | 0.3     | -5.3–6.5   | -8.7–12.2  |
| MCPR                                             | 6.3     | -1.1–16.3  | -10.9–23.0 | 5.6     | -1.4–14.9  | -10.6–21.6 | 5.3     | -3.3–16.1  | -10.7–20.5 | 0.4     | -5.7–8.0   | -8.7–17.0  |
| Southeast (1981–2010 normal: 295.2mm)            |         |            |            |         |            |            |         |            |            |         |            |            |
| CMIP5                                            | 10.3    | 1.5–22.7   | -13.0–29.6 | 11.2    | -0.3–17.1  | -21.3–26.3 | 9.1     | -0.2–18.4  | -9.2–22.3  | 4.2     | -3.9–11.7  | -6.1–15.2  |
| SMME                                             | 4.3     | -0.0–21.9  | -13.0–29.6 | 10.4    | -0.3–15.5  | -21.3–22.1 | 5.6     | -0.2–16.1  | -9.2–21.4  | 2.9     | -0.6–7.9   | -6.1–15.2  |
| MCPR                                             | 11.9    | 4.7–24.8   | -6.4–35.4  | 10.2    | -3.7–20.9  | -9.9–29.8  | 8.3     | -0.9–21.8  | -6.7–28.1  | 1.2     | -6.3–13.6  | -11.3–24.5 |
| South Central (1981–2010 normal: 243.7mm)        |         |            |            |         |            |            |         |            |            |         |            |            |
| CMIP5                                            | 2.3     | -10.2–14.8 | -26.1–25.8 | 2.6     | -9.9–8.3   | -26.8–23.3 | 2.1     | -6.5–8.9   | -16.4–20.1 | -2.4    | -10.1–8.4  | -12.5–14.6 |
| SMME                                             | 0.4     | -10.2–9.8  | -26.1–19.5 | 0.5     | -9.9–8.2   | -26.8–21.3 | 1.4     | -4.4–6.7   | -13.4–20.1 | 0.0     | -7.1–7.1   | -12.5–14.6 |
| MCPR                                             | 3.2     | -12.1–14.7 | -32.8–29.8 | -1.6    | -15.4–8.6  | -27.6–18.6 | 1.1     | -8.7–9.2   | -21.4–19.1 | 0.1     | -12.5–12.4 | -25.3–24.2 |
| Upper Great Plains (1981–2010 normal: 125.2mm)   |         |            |            |         |            |            |         |            |            |         |            |            |
| CMIP5                                            | 2.0     | -5.5–19.1  | -13.5–27.3 | 1.4     | -6.6–11.5  | -18.2–32.0 | 1.5     | -7.6–14.9  | -13.7–19.0 | 2.2     | -10.0–9.1  | -11.9–10.8 |
| SMME                                             | -0.2    | -5.2–8.8   | -11.4–24.7 | 0.8     | -6.6–8.1   | -12.0–20.1 | 0.7     | -4.7–10.7  | -11.8–17.7 | 1.0     | -4.3–9.4   | -11.9–10.8 |
| MCPR                                             | 4.5     | -5.4–13.1  | -14.6–28.1 | 2.5     | -7.8–14.4  | -13.6–28.5 | 4.1     | -7.7–16.0  | -18.8–23.4 | -1.3    | -9.7–7.5   | -17.2–14.1 |
| Midwest (1981–2010 normal: 233.4mm)              |         |            |            |         |            |            |         |            |            |         |            |            |
| CMIP5                                            | 6.5     | -1.5–12.7  | -13.4–16.7 | 2.7     | 0.3–8.1    | -5.2–23.7  | 5.8     | -6.2–13.3  | -9.4–16.4  | 1.5     | -7.8–10.2  | -9.3–15.7  |
| SMME                                             | 3.5     | -0.2–11.0  | -13.4–16.0 | 0.7     | 0.2–6.9    | -5.2–18.3  | 2.6     | -3.0–11.5  | -8.1–16.4  | 1.5     | -6.2–4.6   | -9.3–15.7  |
| MCPR                                             | 6.5     | -1.8–15.4  | -13.2–24.2 | 3.0     | -4.2–12.7  | -7.0–23.1  | 5.9     | -5.0–13.9  | -8.0–23.5  | 0.5     | -7.5–6.5   | -11.3–10.7 |
| Northwest (1981–2010 normal: 202.5mm)            |         |            |            |         |            |            |         |            |            |         |            |            |
| CMIP5                                            | 6.6     | -5.8–17.9  | -14.4–26.5 | 6.2     | -3.5–15.0  | -12.7–38.2 | 4.8     | -6.7–15.8  | -17.6–25.2 | 4.4     | -7.1–11.2  | -9.2–15.9  |
| SMME                                             | 0.9     | -5.6–12.3  | -12.6–19.7 | 1.0     | -3.5–10.7  | -12.7–38.2 | 2.5     | -3.7–10.4  | -11.1–25.2 | 0.1     | -7.1–6.9   | -9.2–11.3  |
| MCPR                                             | 8.8     | -9.7–24.1  | -22.1–37.6 | 5.2     | -7.6–18.6  | -16.2–32.9 | 4.8     | -9.8–23.0  | -18.5–34.9 | 0.8     | -11.7–17.9 | -17.5–32.8 |
| California (1981–2010 normal: 101.3mm)           |         |            |            |         |            |            |         |            |            |         |            |            |
| CMIP5                                            | -12.5   | -25.8–10.2 | -36.5–20.9 | -5.5    | -15.1–5.6  | -33.2–12.9 | -5.4    | -18.6–7.4  | -29.5–17.2 | -6.6    | -14.8–14.6 | -16.4–17.2 |
| SMME                                             | -3.1    | -23.2–0.1  | -36.5–12.5 | -0.9    | -11.7–4.6  | -16.0–5.9  | -0.6    | -9.1–6.4   | -25.0–17.2 | -0.8    | -16.1–10.1 | -16.4–17.2 |
| MCPR                                             | -12.9   | -30.6–9.1  | -54.3–27.1 | -5.5    | -17.3–6.4  | -25.0–11.8 | -4.8    | -22.6–11.3 | -32.7–41.1 | -1.6    | -24.2–15.6 | -33.9–28.3 |
| Southwest (1981–2010 normal: 77.8mm)             |         |            |            |         |            |            |         |            |            |         |            |            |
| CMIP5                                            | 1.9     | -14.1–20.2 | -29.1–42.5 | 4.2     | -18.3–25.7 | -35.9–40.7 | 3.7     | -10.9–17.9 | -20.1–36.3 | 3.8     | -8.4–18.8  | -14.2–22.2 |
| SMME                                             | 0.9     | -5.4–13.2  | -23.2–42.2 | 0.8     | -18.3–19.9 | -28.8–26.9 | 1.2     | -9.4–15.1  | -20.0–27.9 | 0.1     | -8.4–11.2  | -14.2–22.2 |
| MCPR                                             | 1.2     | -17.7–27.9 | -50.8–47.7 | 4.6     | -25.1–24.5 | -30.5–34.6 | 1.5     | -21.5–22.4 | -35.8–31.0 | 7.0     | -12.6–19.1 | -33.1–29.6 |
| Rocky Mountain States (1981–2010 normal: 77.0mm) |         |            |            |         |            |            |         |            |            |         |            |            |
| CMIP5                                            | 7.7     | -2.2–17.6  | -20.1–28.4 | 7.0     | -1.4–12.6  | -16.0–22.5 | 2.4     | -4.3–14.6  | -7.3–22.6  | 2.6     | -5.5–9.2   | -10.2–15.6 |
| SMME                                             | 0.8     | -0.6–17.6  | -10.7–26.2 | 5.5     | 0.3–12.4   | -15.3–13.7 | 0.6     | -3.2–11.4  | -7.3–16.9  | 0.4     | -4.6–8.0   | -10.2–15.6 |
| MCPR                                             | 3.9     | -7.2–23.3  | -20.9–40.8 | 8.6     | -0.9–15.8  | -12.7–21.7 | 5.1     | -8.4–18.6  | -17.2–29.8 | 0.3     | -10.1–10.4 | -18.9–22.9 |
| Alaska (1981–2010 normal: 170.1mm)               |         |            |            |         |            |            |         |            |            |         |            |            |
| CMIP5                                            | 32.4    | 25.4–40.1  | 22.6–48.2  | 17.8    | 14.9–25.8  | 8.0–48.9   | 16.9    | 8.8–20.8   | 5.6–26.4   | 10.3    | 5.9–17.4   | 3.0–23.0   |
| SMME                                             | 31.2    | 1.4–36.8   | 0.9–41.3   | 17.3    | 0.9–20.8   | 0.2–29.7   | 14.3    | 1.2–20.0   | 0.4–26.1   | 7.1     | 0.1–14.9   | -0.0–23.0  |
| MCPR                                             | 27.3    | 17.0–41.8  | 12.3–51.9  | 15.8    | 10.1–25.9  | 6.4–38.3   | 12.4    | 6.2–22.1   | 3.4–30.6   | 7.0     | 1.5–12.4   | -1.8–17.6  |
| Hawaii (1981–2010 normal: 627.7mm)               |         |            |            |         |            |            |         |            |            |         |            |            |
| CMIP5                                            | 13.3    | -2.5–43.8  | -15.4–64.0 | 10.8    | 0.7–40.2   | -26.0–61.0 | 7.0     | -1.3–16.6  | -16.0–42.7 | 7.0     | -0.7–23.0  | -5.1–35.5  |
| SMME                                             | 5.1     | -0.3–35.8  | -15.4–44.3 | 4.5     | -0.2–29.5  | -23.0–45.2 | 3.0     | -0.2–13.5  | -6.1–32.5  | 3.9     | -0.4–21.0  | -5.1–35.5  |
| MCPR                                             | 13.6    | -3.5–26.2  | -22.1–61.7 | 10.6    | -6.7–28.4  | -26.6–37.2 | 5.8     | -7.6–14.2  | -18.2–24.4 | 5.5     | -5.7–20.9  | -12.5–32.5 |

TABLE A13. Projected regional annual temperature change (°C) under all RCPs for 2040-2059

| Annual<br>2040-2059                             | RCP 8.5 |         |         | RCP 6.0 |         |         | RCP 4.5 |         |         | RCP 2.6 |         |         |
|-------------------------------------------------|---------|---------|---------|---------|---------|---------|---------|---------|---------|---------|---------|---------|
|                                                 | 50      | 17-83   | 5-95    | 50      | 17-83   | 5-95    | 50      | 17-83   | 5-95    | 50      | 17-83   | 5-95    |
| CONUS (1981-2010 normal: 11.9°C)                |         |         |         |         |         |         |         |         |         |         |         |         |
| CMIP5                                           | 2.5     | 1.8-3.1 | 1.4-3.5 | 1.5     | 1.3-1.9 | 0.8-2.4 | 1.8     | 1.3-2.4 | 0.8-2.8 | 1.5     | 1.2-1.9 | 0.8-2.3 |
| SMME                                            | 2.5     | 1.5-3.2 | 1.4-3.5 | 1.5     | 1.2-1.9 | 0.7-2.5 | 1.9     | 1.3-2.7 | 0.9-3.0 | 1.4     | 1.0-1.9 | 0.8-2.4 |
| MCPR                                            | 2.1     | 1.6-2.9 | 1.5-3.7 | 1.5     | 1.1-2.0 | 0.9-2.4 | 1.7     | 1.3-2.2 | 1.1-3.0 | 1.4     | 0.9-1.9 | 0.7-2.3 |
| Northeast (1981-2010 normal: 8.8°C)             |         |         |         |         |         |         |         |         |         |         |         |         |
| CMIP5                                           | 2.5     | 1.9-3.1 | 1.6-3.8 | 1.5     | 1.1-1.9 | 0.9-2.7 | 1.9     | 1.5-2.4 | 0.9-3.0 | 1.6     | 1.2-2.3 | 0.8-2.6 |
| SMME                                            | 2.5     | 1.7-3.5 | 1.3-3.9 | 1.5     | 1.1-2.1 | 0.8-2.7 | 1.9     | 1.5-2.9 | 1.0-3.1 | 1.6     | 1.1-2.3 | 0.7-2.7 |
| MCPR                                            | 2.2     | 1.8-3.1 | 1.5-4.0 | 1.4     | 1.1-2.1 | 0.9-2.5 | 1.8     | 1.4-2.4 | 1.2-3.2 | 1.4     | 0.8-2.0 | 0.5-2.7 |
| Southeast (1981-2010 normal: 16.6°C)            |         |         |         |         |         |         |         |         |         |         |         |         |
| CMIP5                                           | 2.1     | 1.6-2.5 | 1.3-2.9 | 1.2     | 1.1-1.6 | 0.7-2.0 | 1.6     | 1.2-2.0 | 0.7-2.4 | 1.2     | 0.9-1.7 | 0.7-1.9 |
| SMME                                            | 2.2     | 1.4-2.8 | 1.1-3.1 | 1.3     | 1.1-1.7 | 0.6-1.9 | 1.7     | 1.3-2.2 | 0.8-2.6 | 1.2     | 0.9-1.7 | 0.5-2.0 |
| MCPR                                            | 1.8     | 1.5-2.6 | 1.2-3.3 | 1.2     | 0.8-1.7 | 0.7-2.0 | 1.5     | 1.2-2.0 | 0.8-2.6 | 1.1     | 0.7-1.6 | 0.4-2.0 |
| South Central (1981-2010 normal: 17.8°C)        |         |         |         |         |         |         |         |         |         |         |         |         |
| CMIP5                                           | 2.4     | 1.7-2.8 | 1.3-3.1 | 1.5     | 1.3-1.9 | 0.7-2.1 | 1.7     | 1.4-2.3 | 0.7-2.6 | 1.4     | 1.1-1.9 | 1.0-1.9 |
| SMME                                            | 2.4     | 1.6-2.8 | 1.3-3.2 | 1.5     | 1.3-1.9 | 0.6-2.1 | 1.8     | 1.4-2.4 | 0.9-2.8 | 1.4     | 1.1-1.8 | 0.7-2.0 |
| MCPR                                            | 2.0     | 1.5-2.7 | 1.3-3.4 | 1.4     | 1.1-1.9 | 0.8-2.2 | 1.6     | 1.2-2.3 | 1.0-2.7 | 1.3     | 0.8-1.8 | 0.6-2.4 |
| Upper Great Plains (1981-2010 normal: 8.9°C)    |         |         |         |         |         |         |         |         |         |         |         |         |
| CMIP5                                           | 2.6     | 1.8-3.3 | 1.2-3.8 | 1.6     | 1.2-2.2 | 0.8-2.5 | 1.9     | 1.3-2.6 | 1.0-3.2 | 1.6     | 1.2-2.2 | 0.8-2.5 |
| SMME                                            | 2.7     | 1.7-3.5 | 1.4-3.9 | 1.6     | 1.2-2.2 | 0.7-2.7 | 2.0     | 1.4-3.1 | 1.0-3.5 | 1.5     | 1.1-2.2 | 0.8-2.7 |
| MCPR                                            | 2.3     | 1.7-3.2 | 1.4-4.1 | 1.5     | 1.1-2.2 | 0.9-2.6 | 1.9     | 1.4-2.4 | 1.1-3.2 | 1.5     | 0.9-2.2 | 0.7-2.7 |
| Midwest (1981-2010 normal: 9.0°C)               |         |         |         |         |         |         |         |         |         |         |         |         |
| CMIP5                                           | 2.7     | 1.9-3.3 | 1.6-4.1 | 1.7     | 1.2-2.1 | 1.0-2.8 | 2.0     | 1.5-2.6 | 1.1-3.3 | 1.7     | 1.1-2.4 | 0.9-2.8 |
| SMME                                            | 2.8     | 1.6-3.8 | 1.6-4.1 | 1.7     | 1.1-2.1 | 0.8-2.9 | 2.1     | 1.4-3.3 | 1.1-3.7 | 1.7     | 1.0-2.4 | 0.8-2.8 |
| MCPR                                            | 2.4     | 1.8-3.2 | 1.5-4.2 | 1.6     | 1.1-2.2 | 0.9-2.8 | 1.9     | 1.5-2.5 | 1.2-3.4 | 1.5     | 1.0-2.2 | 0.7-2.8 |
| Northwest (1981-2010 normal: 9.5°C)             |         |         |         |         |         |         |         |         |         |         |         |         |
| CMIP5                                           | 2.2     | 1.6-2.9 | 1.2-3.3 | 1.4     | 1.0-1.8 | 0.7-2.2 | 1.7     | 0.9-2.2 | 0.7-2.5 | 1.4     | 1.1-2.0 | 0.9-2.5 |
| SMME                                            | 2.2     | 1.2-3.0 | 1.1-3.5 | 1.4     | 0.8-2.0 | 0.7-2.6 | 1.7     | 1.0-2.5 | 0.7-3.0 | 1.3     | 0.9-2.0 | 0.6-2.6 |
| MCPR                                            | 2.0     | 1.5-2.8 | 1.2-3.3 | 1.4     | 1.0-1.8 | 0.7-2.3 | 1.5     | 1.1-2.2 | 0.8-3.0 | 1.4     | 0.9-1.8 | 0.7-2.4 |
| California (1981-2010 normal: 15.5°C)           |         |         |         |         |         |         |         |         |         |         |         |         |
| CMIP5                                           | 2.1     | 1.6-2.6 | 1.2-2.8 | 1.4     | 1.1-1.7 | 0.7-2.1 | 1.6     | 1.0-2.0 | 0.7-2.3 | 1.3     | 1.0-1.7 | 0.7-2.1 |
| SMME                                            | 2.2     | 1.3-2.7 | 1.2-2.9 | 1.4     | 1.0-1.8 | 0.6-2.1 | 1.7     | 1.0-2.3 | 0.7-2.5 | 1.2     | 0.9-1.7 | 0.6-2.2 |
| MCPR                                            | 1.9     | 1.4-2.5 | 1.2-3.0 | 1.3     | 1.0-1.7 | 0.8-2.2 | 1.4     | 1.0-2.0 | 0.8-2.5 | 1.2     | 0.8-1.6 | 0.6-2.0 |
| Southwest (1981-2010 normal: 14.2°C)            |         |         |         |         |         |         |         |         |         |         |         |         |
| CMIP5                                           | 2.4     | 1.8-2.9 | 1.6-3.4 | 1.6     | 1.4-2.0 | 0.8-2.2 | 1.7     | 1.3-2.3 | 0.7-2.6 | 1.6     | 1.0-1.7 | 0.9-2.3 |
| SMME                                            | 2.5     | 1.6-3.2 | 1.4-3.4 | 1.6     | 1.3-2.0 | 0.6-2.2 | 1.8     | 1.4-2.6 | 0.8-2.8 | 1.4     | 1.0-1.7 | 0.8-2.3 |
| MCPR                                            | 2.1     | 1.7-2.9 | 1.4-3.5 | 1.5     | 1.1-2.0 | 0.7-2.4 | 1.7     | 1.3-2.3 | 1.0-2.7 | 1.3     | 0.9-1.9 | 0.6-2.2 |
| Rocky Mountain States (1981-2010 normal: 8.1°C) |         |         |         |         |         |         |         |         |         |         |         |         |
| CMIP5                                           | 2.6     | 1.8-3.3 | 1.4-3.9 | 1.6     | 1.2-2.0 | 0.9-2.6 | 1.9     | 1.1-2.5 | 0.8-3.0 | 1.5     | 1.2-2.1 | 0.9-2.7 |
| SMME                                            | 2.6     | 1.6-3.6 | 1.4-3.9 | 1.6     | 1.2-2.1 | 0.7-2.8 | 2.0     | 1.2-2.9 | 0.9-3.3 | 1.5     | 1.0-2.1 | 0.8-2.7 |
| MCPR                                            | 2.2     | 1.6-3.1 | 1.4-3.8 | 1.6     | 1.1-2.1 | 0.9-2.6 | 1.8     | 1.3-2.5 | 1.1-2.9 | 1.4     | 1.0-1.9 | 0.8-2.5 |
| Alaska (1981-2010 normal: -1.7°C)               |         |         |         |         |         |         |         |         |         |         |         |         |
| CMIP5                                           | 3.2     | 2.2-4.0 | 2.0-4.8 | 1.8     | 1.6-2.7 | 0.8-3.2 | 2.2     | 1.6-3.3 | 1.3-3.8 | 2.0     | 1.4-3.0 | 1.0-3.4 |
| SMME                                            | 3.2     | 2.2-4.4 | 1.4-5.1 | 1.8     | 1.5-3.0 | 0.8-3.2 | 2.5     | 1.6-3.6 | 1.6-4.1 | 1.9     | 1.4-2.8 | 1.0-3.4 |
| MCPR                                            | 3.0     | 2.1-4.4 | 1.8-5.2 | 2.0     | 1.3-2.8 | 1.0-3.4 | 2.3     | 1.6-3.5 | 1.1-4.5 | 1.9     | 1.2-2.6 | 0.8-3.2 |
| Hawaii (1981-2010 normal: 23.6°C)               |         |         |         |         |         |         |         |         |         |         |         |         |
| CMIP5                                           | 1.4     | 1.0-1.9 | 0.9-2.2 | 0.8     | 0.7-1.4 | 0.6-1.6 | 1.0     | 0.7-1.4 | 0.4-1.8 | 0.9     | 0.6-1.3 | 0.6-1.4 |
| SMME                                            | 1.4     | 0.9-2.0 | 0.7-2.4 | 0.8     | 0.7-1.5 | 0.6-1.8 | 1.0     | 0.8-1.5 | 0.7-1.8 | 0.8     | 0.6-1.3 | 0.5-1.5 |
| MCPR                                            | 1.3     | 1.0-1.8 | 0.9-2.3 | 0.9     | 0.6-1.2 | 0.5-1.5 | 1.0     | 0.7-1.4 | 0.5-1.7 | 0.8     | 0.5-1.3 | 0.4-1.7 |

TABLE A14. Projected regional DJF temperature change (°C) under all RCPs for 2040-2059

| DJF<br>2040-2059                                 | RCP 8.5 |         |         | RCP 6.0 |         |          | RCP 4.5 |         |         | RCP 2.6 |         |          |
|--------------------------------------------------|---------|---------|---------|---------|---------|----------|---------|---------|---------|---------|---------|----------|
|                                                  | 50      | 17-83   | 5-95    | 50      | 17-83   | 5-95     | 50      | 17-83   | 5-95    | 50      | 17-83   | 5-95     |
| CONUS (1981–2010 normal: 0.9°C)                  |         |         |         |         |         |          |         |         |         |         |         |          |
| CMIP5                                            | 2.2     | 1.7–3.0 | 1.2–3.9 | 1.4     | 1.1–1.9 | 0.7–2.9  | 1.9     | 1.3–2.3 | 1.0–3.2 | 1.5     | 1.1–2.0 | 0.5–2.3  |
| SMME                                             | 2.2     | 1.4–3.3 | 1.2–3.9 | 1.4     | 0.8–1.9 | 0.6–2.8  | 1.8     | 1.5–2.8 | 1.0–3.4 | 1.4     | 1.0–1.9 | 0.5–2.5  |
| MCPR                                             | 2.0     | 1.6–2.9 | 0.9–4.0 | 1.4     | 0.8–2.0 | 0.5–2.6  | 1.7     | 1.3–2.4 | 1.0–2.8 | 1.2     | 0.7–1.9 | 0.5–2.4  |
| Northeast (1981–2010 normal: -3.2°C)             |         |         |         |         |         |          |         |         |         |         |         |          |
| CMIP5                                            | 2.8     | 1.9–3.5 | 1.4–3.7 | 1.6     | 1.0–2.3 | 0.5–3.1  | 2.1     | 1.7–2.8 | 0.8–3.7 | 1.7     | 1.1–2.4 | 0.7–2.9  |
| SMME                                             | 2.8     | 1.6–3.6 | 1.4–4.3 | 1.3     | 0.9–2.3 | 0.3–3.1  | 2.0     | 1.7–3.0 | 1.0–3.7 | 1.4     | 1.0–2.2 | 0.2–3.2  |
| MCPR                                             | 2.3     | 1.7–3.2 | 1.4–4.4 | 1.4     | 0.8–2.4 | 0.3–3.0  | 2.0     | 1.2–2.8 | 0.9–3.8 | 1.5     | 0.4–2.2 | -0.4–3.0 |
| Southeast (1981–2010 normal: 7.2°C)              |         |         |         |         |         |          |         |         |         |         |         |          |
| CMIP5                                            | 1.9     | 1.1–2.5 | 0.9–2.8 | 1.0     | 0.5–1.5 | 0.1–1.7  | 1.5     | 0.9–2.0 | 0.6–2.4 | 1.3     | 0.8–1.6 | 0.5–1.7  |
| SMME                                             | 1.9     | 1.1–2.5 | 0.5–2.8 | 1.0     | 0.5–1.5 | 0.0–1.7  | 1.5     | 0.9–1.9 | 0.7–2.4 | 0.9     | 0.7–1.5 | 0.1–1.8  |
| MCPR                                             | 1.6     | 1.1–2.4 | 0.8–2.7 | 0.8     | 0.4–1.5 | -0.0–1.9 | 1.3     | 0.6–1.9 | 0.3–2.8 | 1.0     | 0.2–1.6 | -0.3–2.2 |
| South Central (1981–2010 normal: 7.8°C)          |         |         |         |         |         |          |         |         |         |         |         |          |
| CMIP5                                            | 2.1     | 1.7–2.9 | 1.2–2.9 | 1.3     | 1.0–1.8 | 0.4–2.0  | 1.6     | 1.2–2.1 | 0.7–3.0 | 1.4     | 1.1–1.9 | 0.8–2.1  |
| SMME                                             | 2.1     | 1.4–2.9 | 0.7–3.1 | 1.4     | 1.0–1.8 | 0.2–2.0  | 1.6     | 1.3–2.1 | 0.7–3.2 | 1.3     | 1.1–1.7 | 0.4–2.1  |
| MCPR                                             | 1.9     | 1.4–2.7 | 0.6–3.6 | 1.1     | 0.7–1.7 | 0.3–2.2  | 1.5     | 1.0–2.2 | 0.7–2.6 | 1.1     | 0.6–1.8 | 0.1–2.3  |
| Upper Great Plains (1981–2010 normal: -4.7°C)    |         |         |         |         |         |          |         |         |         |         |         |          |
| CMIP5                                            | 2.8     | 1.9–3.7 | 0.8–5.0 | 1.5     | 1.0–2.8 | 0.4–3.6  | 2.3     | 1.4–3.1 | 1.1–4.2 | 1.6     | 1.0–2.5 | 0.4–2.6  |
| SMME                                             | 2.6     | 1.5–4.0 | 0.8–4.9 | 1.4     | 0.6–2.9 | 0.4–3.6  | 2.3     | 1.4–3.4 | 1.1–4.8 | 1.5     | 1.1–2.4 | 0.4–3.0  |
| MCPR                                             | 2.5     | 1.5–3.7 | 0.7–5.2 | 1.6     | 0.8–2.5 | 0.3–3.0  | 2.0     | 1.3–2.9 | 0.8–3.9 | 1.4     | 0.6–2.1 | 0.2–3.0  |
| Midwest (1981–2010 normal: -4.5°C)               |         |         |         |         |         |          |         |         |         |         |         |          |
| CMIP5                                            | 2.8     | 2.0–3.9 | 1.4–4.9 | 1.7     | 1.1–2.5 | 0.5–3.9  | 2.3     | 1.8–3.0 | 1.2–4.0 | 1.8     | 1.3–2.6 | 0.4–3.0  |
| SMME                                             | 2.7     | 1.6–4.3 | 1.4–5.0 | 1.5     | 1.0–2.6 | 0.5–3.9  | 2.3     | 1.8–3.9 | 1.4–4.5 | 1.6     | 0.8–2.3 | 0.4–3.4  |
| MCPR                                             | 2.5     | 1.7–3.6 | 0.9–5.0 | 1.6     | 0.8–2.6 | 0.1–3.5  | 2.1     | 1.6–3.1 | 1.0–3.8 | 1.5     | 0.8–2.5 | -0.3–3.0 |
| Northwest (1981–2010 normal: 1.1°C)              |         |         |         |         |         |          |         |         |         |         |         |          |
| CMIP5                                            | 2.2     | 1.3–2.8 | 0.9–3.6 | 1.4     | 1.1–2.0 | 0.0–2.8  | 1.6     | 1.1–2.4 | 0.9–2.7 | 1.4     | 0.9–2.4 | 0.6–2.6  |
| SMME                                             | 2.2     | 1.2–3.0 | 0.8–3.8 | 1.4     | 0.9–1.9 | 0.8–2.8  | 1.6     | 1.1–2.6 | 0.9–3.4 | 1.3     | 0.9–2.0 | 0.6–2.6  |
| MCPR                                             | 1.9     | 1.3–2.7 | 1.0–3.3 | 1.3     | 0.9–2.1 | 0.4–2.3  | 1.6     | 1.0–2.3 | 0.5–3.2 | 1.3     | 0.6–2.0 | 0.3–2.5  |
| California (1981–2010 normal: 7.7°C)             |         |         |         |         |         |          |         |         |         |         |         |          |
| CMIP5                                            | 1.9     | 1.3–2.3 | 0.8–2.6 | 1.3     | 1.1–1.7 | 0.4–2.1  | 1.4     | 1.0–2.0 | 0.5–2.1 | 1.2     | 0.8–1.8 | 0.6–1.9  |
| SMME                                             | 1.8     | 1.0–2.3 | 0.7–2.7 | 1.2     | 1.1–1.7 | 0.6–2.1  | 1.4     | 1.1–2.1 | 0.5–2.6 | 1.1     | 0.8–1.6 | 0.6–1.9  |
| MCPR                                             | 1.6     | 1.2–2.3 | 0.9–2.7 | 1.2     | 0.8–1.6 | 0.6–2.0  | 1.4     | 0.9–1.8 | 0.7–2.3 | 1.2     | 0.6–1.6 | 0.4–1.9  |
| Southwest (1981–2010 normal: 4.6°C)              |         |         |         |         |         |          |         |         |         |         |         |          |
| CMIP5                                            | 2.2     | 1.6–2.5 | 1.2–3.2 | 1.5     | 1.2–1.9 | 0.7–2.4  | 1.7     | 1.2–2.3 | 0.7–2.6 | 1.4     | 1.0–1.8 | 0.6–2.1  |
| SMME                                             | 2.2     | 1.3–3.0 | 1.0–3.2 | 1.4     | 1.2–1.7 | 0.7–2.2  | 1.6     | 1.2–2.4 | 0.7–3.0 | 1.4     | 1.0–1.7 | 0.6–2.1  |
| MCPR                                             | 1.9     | 1.4–2.7 | 1.0–3.2 | 1.3     | 0.9–1.9 | 0.7–2.3  | 1.6     | 1.1–2.0 | 1.0–2.5 | 1.2     | 0.7–1.8 | 0.5–2.1  |
| Rocky Mountain States (1981–2010 normal: -3.2°C) |         |         |         |         |         |          |         |         |         |         |         |          |
| CMIP5                                            | 2.4     | 1.7–3.3 | 1.2–4.6 | 1.6     | 1.1–2.3 | -0.0–3.4 | 2.0     | 1.2–2.8 | 0.9–3.2 | 1.5     | 0.8–2.3 | 0.7–2.9  |
| SMME                                             | 2.4     | 1.5–3.6 | 1.2–4.7 | 1.4     | 1.1–2.2 | 0.8–3.4  | 1.7     | 1.4–3.1 | 0.9–4.1 | 1.4     | 0.8–2.1 | 0.7–3.0  |
| MCPR                                             | 2.2     | 1.5–3.1 | 1.1–3.9 | 1.5     | 0.9–2.2 | 0.5–3.0  | 1.8     | 1.2–2.6 | 1.0–3.3 | 1.4     | 0.8–2.0 | 0.5–2.6  |
| Alaska (1981–2010 normal: -15.4°C)               |         |         |         |         |         |          |         |         |         |         |         |          |
| CMIP5                                            | 4.0     | 3.1–6.1 | 1.9–7.0 | 2.9     | 1.7–3.9 | 0.9–4.8  | 3.3     | 1.8–4.8 | 1.2–5.2 | 2.4     | 1.4–3.9 | 0.0–4.2  |
| SMME                                             | 4.4     | 2.5–6.1 | 1.1–6.5 | 2.7     | 1.1–3.8 | 0.9–4.3  | 3.3     | 1.9–5.0 | 1.2–5.6 | 2.0     | 1.5–3.6 | 0.0–4.2  |
| MCPR                                             | 4.2     | 2.6–5.9 | 1.4–7.7 | 2.5     | 1.3–4.0 | 0.5–5.0  | 3.1     | 1.5–4.7 | 0.6–6.2 | 2.2     | 1.1–3.5 | 0.2–5.4  |
| Hawaii (1981–2010 normal: 22.1°C)                |         |         |         |         |         |          |         |         |         |         |         |          |
| CMIP5                                            | 1.4     | 1.1–1.9 | 0.8–2.1 | 0.9     | 0.8–1.3 | 0.6–1.7  | 1.0     | 0.8–1.5 | 0.6–1.7 | 0.8     | 0.6–1.2 | 0.5–1.2  |
| SMME                                             | 1.3     | 0.9–1.9 | 0.8–2.1 | 0.9     | 0.6–1.3 | 0.6–1.7  | 1.0     | 0.8–1.5 | 0.6–1.8 | 0.8     | 0.5–1.2 | 0.5–1.2  |
| MCPR                                             | 1.2     | 1.0–1.7 | 0.8–2.0 | 0.9     | 0.6–1.1 | 0.3–1.4  | 0.9     | 0.7–1.4 | 0.5–1.7 | 0.7     | 0.5–1.1 | 0.4–1.5  |

TABLE A15. Projected regional MAM temperature change (°C) under all RCPs for 2040-2059

| MAM<br>2040-2059                                | RCP 8.5 |         |         | RCP 6.0 |         |         | RCP 4.5 |         |         | RCP 2.6 |         |         |
|-------------------------------------------------|---------|---------|---------|---------|---------|---------|---------|---------|---------|---------|---------|---------|
|                                                 | 50      | 17-83   | 5-95    | 50      | 17-83   | 5-95    | 50      | 17-83   | 5-95    | 50      | 17-83   | 5-95    |
| CONUS (1981-2010 normal: 11.4°C)                |         |         |         |         |         |         |         |         |         |         |         |         |
| CMIP5                                           | 2.2     | 1.6-2.8 | 1.1-3.4 | 1.5     | 1.2-1.9 | 0.7-2.7 | 1.8     | 1.1-2.3 | 0.8-3.0 | 1.4     | 0.9-2.3 | 0.9-2.6 |
| SMME                                            | 2.2     | 1.3-3.2 | 1.1-3.5 | 1.4     | 1.1-1.9 | 0.6-2.6 | 1.7     | 1.1-2.5 | 0.8-3.0 | 1.3     | 0.8-2.2 | 0.6-2.6 |
| MCPR                                            | 1.9     | 1.5-2.6 | 1.2-3.4 | 1.4     | 0.9-1.9 | 0.7-2.4 | 1.6     | 1.1-2.2 | 0.9-3.0 | 1.3     | 0.8-1.9 | 0.6-2.5 |
| Northeast (1981-2010 normal: 7.8°C)             |         |         |         |         |         |         |         |         |         |         |         |         |
| CMIP5                                           | 2.3     | 1.6-3.1 | 1.5-4.0 | 1.5     | 1.1-2.0 | 1.0-3.4 | 1.8     | 1.2-2.6 | 1.0-3.1 | 1.6     | 0.9-2.4 | 0.8-3.0 |
| SMME                                            | 2.3     | 1.5-3.8 | 1.5-4.1 | 1.4     | 1.0-2.0 | 1.0-3.3 | 1.8     | 1.2-2.6 | 1.0-3.3 | 1.4     | 0.8-2.4 | 0.6-3.1 |
| MCPR                                            | 2.0     | 1.5-2.9 | 1.0-3.7 | 1.5     | 0.9-2.1 | 0.7-2.6 | 1.7     | 1.2-2.2 | 0.9-3.0 | 1.5     | 0.7-2.2 | 0.2-3.0 |
| Southeast (1981-2010 normal: 16.3°C)            |         |         |         |         |         |         |         |         |         |         |         |         |
| CMIP5                                           | 2.1     | 1.5-2.5 | 1.2-2.8 | 1.4     | 1.0-1.6 | 0.8-2.2 | 1.7     | 1.1-2.1 | 0.7-2.5 | 1.3     | 0.7-1.9 | 0.7-2.2 |
| SMME                                            | 2.1     | 1.3-2.6 | 1.1-2.8 | 1.4     | 0.9-1.6 | 0.7-2.0 | 1.6     | 1.2-2.2 | 0.7-2.5 | 1.2     | 0.6-1.7 | 0.5-2.2 |
| MCPR                                            | 1.8     | 1.3-2.4 | 1.1-3.2 | 1.3     | 0.8-1.8 | 0.6-2.0 | 1.4     | 1.1-2.0 | 0.8-2.6 | 1.2     | 0.5-1.8 | 0.1-2.3 |
| South Central (1981-2010 normal: 17.7°C)        |         |         |         |         |         |         |         |         |         |         |         |         |
| CMIP5                                           | 2.2     | 1.6-2.8 | 1.1-3.0 | 1.5     | 1.3-1.8 | 0.8-2.6 | 1.6     | 1.2-2.3 | 0.8-2.6 | 1.4     | 1.1-1.9 | 0.7-2.0 |
| SMME                                            | 2.2     | 1.3-2.9 | 1.1-3.1 | 1.5     | 1.2-1.8 | 0.7-2.2 | 1.6     | 1.2-2.4 | 0.8-2.6 | 1.2     | 1.1-1.8 | 0.6-2.0 |
| MCPR                                            | 1.9     | 1.4-2.6 | 1.1-3.3 | 1.4     | 1.0-1.9 | 0.7-2.2 | 1.5     | 1.1-2.2 | 0.8-2.9 | 1.2     | 0.6-2.0 | 0.4-2.3 |
| Upper Great Plains (1981-2010 normal: 8.6°C)    |         |         |         |         |         |         |         |         |         |         |         |         |
| CMIP5                                           | 2.1     | 1.4-3.1 | 1.1-3.6 | 1.3     | 1.1-2.0 | 0.6-2.8 | 1.7     | 1.2-2.6 | 0.8-3.3 | 1.5     | 1.0-2.7 | 0.8-2.8 |
| SMME                                            | 2.1     | 1.4-3.2 | 1.1-3.6 | 1.3     | 1.0-2.0 | 0.4-2.8 | 1.7     | 1.2-3.0 | 0.8-3.4 | 1.3     | 0.8-2.4 | 0.7-3.0 |
| MCPR                                            | 2.0     | 1.2-2.9 | 1.0-3.9 | 1.4     | 0.8-2.0 | 0.5-2.6 | 1.6     | 1.0-2.4 | 0.8-3.3 | 1.4     | 0.7-2.2 | 0.4-3.0 |
| Midwest (1981-2010 normal: 8.8°C)               |         |         |         |         |         |         |         |         |         |         |         |         |
| CMIP5                                           | 2.3     | 1.5-3.0 | 1.1-4.2 | 1.4     | 1.1-1.9 | 0.8-3.0 | 1.9     | 1.2-2.5 | 0.8-3.7 | 1.5     | 1.0-2.9 | 0.8-3.3 |
| SMME                                            | 2.3     | 1.5-3.7 | 1.1-4.3 | 1.4     | 1.0-1.9 | 0.8-3.0 | 1.8     | 1.2-2.8 | 0.8-3.8 | 1.3     | 0.8-2.2 | 0.7-3.3 |
| MCPR                                            | 2.0     | 1.3-2.9 | 1.0-4.2 | 1.4     | 0.9-2.1 | 0.6-2.8 | 1.7     | 1.2-2.5 | 0.8-3.5 | 1.5     | 0.7-2.2 | 0.3-3.1 |
| Northwest (1981-2010 normal: 9.0°C)             |         |         |         |         |         |         |         |         |         |         |         |         |
| CMIP5                                           | 2.0     | 1.2-2.5 | 1.0-2.8 | 1.4     | 0.8-1.9 | 0.6-2.4 | 1.5     | 0.9-2.3 | 0.5-2.7 | 1.3     | 1.0-2.0 | 0.8-2.4 |
| SMME                                            | 2.0     | 1.2-2.6 | 0.9-3.0 | 1.3     | 0.7-1.9 | 0.4-2.4 | 1.5     | 0.9-2.4 | 0.5-2.9 | 1.1     | 0.8-2.0 | 0.6-2.6 |
| MCPR                                            | 1.7     | 1.3-2.3 | 1.0-2.9 | 1.3     | 0.8-1.7 | 0.6-2.1 | 1.3     | 0.8-2.2 | 0.5-2.8 | 1.2     | 0.7-1.9 | 0.3-2.3 |
| California (1981-2010 normal: 14.2°C)           |         |         |         |         |         |         |         |         |         |         |         |         |
| CMIP5                                           | 2.0     | 1.3-2.3 | 0.9-2.5 | 1.4     | 1.0-1.6 | 0.4-1.9 | 1.5     | 1.0-1.9 | 0.4-2.2 | 1.1     | 0.9-1.6 | 0.7-1.7 |
| SMME                                            | 1.9     | 1.2-2.3 | 0.7-2.5 | 1.4     | 0.6-1.6 | 0.3-1.9 | 1.6     | 1.0-2.0 | 0.4-2.3 | 1.0     | 0.6-1.6 | 0.6-2.0 |
| MCPR                                            | 1.6     | 1.2-2.3 | 1.0-2.6 | 1.1     | 0.7-1.7 | 0.5-2.1 | 1.3     | 0.8-2.0 | 0.5-2.8 | 1.1     | 0.5-1.6 | 0.2-2.0 |
| Southwest (1981-2010 normal: 13.4°C)            |         |         |         |         |         |         |         |         |         |         |         |         |
| CMIP5                                           | 2.3     | 1.9-3.0 | 1.2-3.1 | 1.6     | 1.3-1.9 | 0.6-2.1 | 1.9     | 1.2-2.4 | 0.7-2.9 | 1.5     | 1.1-1.9 | 0.7-2.2 |
| SMME                                            | 2.3     | 1.2-3.1 | 0.8-3.8 | 1.6     | 1.0-1.9 | 0.4-2.1 | 1.9     | 1.2-2.4 | 0.7-3.1 | 1.4     | 1.1-1.8 | 0.7-2.2 |
| MCPR                                            | 2.0     | 1.5-2.8 | 1.2-3.4 | 1.4     | 0.9-2.0 | 0.6-2.4 | 1.6     | 1.1-2.3 | 0.8-3.1 | 1.3     | 0.6-1.9 | 0.3-2.4 |
| Rocky Mountain States (1981-2010 normal: 7.6°C) |         |         |         |         |         |         |         |         |         |         |         |         |
| CMIP5                                           | 2.4     | 1.7-3.0 | 1.1-4.1 | 1.5     | 1.1-2.4 | 0.4-3.4 | 1.9     | 1.0-2.6 | 0.6-3.6 | 1.5     | 1.0-2.8 | 0.9-3.1 |
| SMME                                            | 2.4     | 1.1-3.9 | 1.1-4.2 | 1.5     | 0.7-2.0 | 0.3-3.4 | 1.9     | 1.0-2.7 | 0.6-3.8 | 1.3     | 0.8-2.6 | 0.6-3.1 |
| MCPR                                            | 2.0     | 1.5-2.8 | 1.2-3.5 | 1.6     | 0.9-2.2 | 0.5-2.9 | 1.6     | 1.0-2.5 | 0.7-3.4 | 1.5     | 0.8-2.2 | 0.6-2.8 |
| Alaska (1981-2010 normal: -1.9°C)               |         |         |         |         |         |         |         |         |         |         |         |         |
| CMIP5                                           | 2.8     | 1.8-4.5 | 1.5-4.9 | 1.8     | 1.4-3.0 | 1.0-4.1 | 2.5     | 1.6-3.4 | 1.2-3.9 | 1.6     | 1.2-3.1 | 0.9-3.4 |
| SMME                                            | 2.6     | 1.8-4.6 | 1.6-5.0 | 1.7     | 1.2-3.0 | 1.0-4.1 | 2.2     | 1.6-3.6 | 1.3-4.1 | 1.6     | 1.2-2.9 | 0.9-3.5 |
| MCPR                                            | 2.6     | 1.7-4.1 | 1.1-5.1 | 2.0     | 1.2-2.6 | 0.9-3.4 | 2.4     | 1.1-3.3 | 0.7-4.2 | 1.8     | 0.8-2.6 | 0.4-3.1 |
| Hawaii (1981-2010 normal: 22.8°C)               |         |         |         |         |         |         |         |         |         |         |         |         |
| CMIP5                                           | 1.5     | 0.9-1.9 | 0.8-2.1 | 0.9     | 0.7-1.4 | 0.4-1.6 | 1.0     | 0.8-1.5 | 0.6-1.8 | 0.9     | 0.6-1.2 | 0.6-1.3 |
| SMME                                            | 1.4     | 0.8-1.8 | 0.7-2.1 | 0.9     | 0.7-1.4 | 0.4-1.6 | 0.9     | 0.8-1.4 | 0.6-1.7 | 0.7     | 0.6-1.2 | 0.5-1.3 |
| MCPR                                            | 1.2     | 1.0-1.8 | 0.8-2.1 | 0.9     | 0.6-1.2 | 0.4-1.4 | 1.0     | 0.7-1.4 | 0.5-1.7 | 0.8     | 0.5-1.2 | 0.3-1.6 |

TABLE A16. Projected regional JJA temperature change (°C) under all RCPs for 2040-2059

| JJA<br>2040-2059                                 | RCP 8.5 |         |         | RCP 6.0 |         |         | RCP 4.5 |         |         | RCP 2.6 |         |         |
|--------------------------------------------------|---------|---------|---------|---------|---------|---------|---------|---------|---------|---------|---------|---------|
|                                                  | 50      | 17-83   | 5-95    | 50      | 17-83   | 5-95    | 50      | 17-83   | 5-95    | 50      | 17-83   | 5-95    |
| CONUS (1981-2010 normal: 22.6°C)                 |         |         |         |         |         |         |         |         |         |         |         |         |
| CMIP5                                            | 2.7     | 1.9-3.3 | 1.6-3.8 | 1.8     | 1.5-2.2 | 0.9-2.7 | 2.0     | 1.5-2.6 | 1.0-3.0 | 1.5     | 1.2-2.2 | 1.0-2.3 |
| SMME                                             | 2.7     | 1.8-3.6 | 1.4-3.8 | 1.7     | 1.2-2.1 | 0.7-2.3 | 1.9     | 1.5-2.9 | 1.0-3.2 | 1.4     | 1.2-2.1 | 0.7-2.5 |
| MCPR                                             | 2.4     | 1.8-3.2 | 1.6-3.8 | 1.6     | 1.2-2.1 | 1.0-2.6 | 1.8     | 1.4-2.6 | 1.1-3.1 | 1.4     | 1.0-2.0 | 0.6-2.6 |
| Northeast (1981-2010 normal: 20.2°C)             |         |         |         |         |         |         |         |         |         |         |         |         |
| CMIP5                                            | 2.6     | 2.3-3.3 | 1.6-3.8 | 1.7     | 1.4-2.1 | 0.9-3.0 | 2.0     | 1.4-2.6 | 0.8-3.1 | 1.6     | 0.8-2.2 | 0.8-2.4 |
| SMME                                             | 2.5     | 1.6-3.4 | 1.1-4.3 | 1.6     | 1.0-2.0 | 0.8-2.3 | 2.0     | 1.4-2.6 | 0.8-3.5 | 1.4     | 0.8-2.1 | 0.7-2.5 |
| MCPR                                             | 2.4     | 1.8-3.3 | 1.6-3.9 | 1.6     | 1.1-2.0 | 0.8-2.6 | 1.7     | 1.3-2.4 | 1.1-3.1 | 1.4     | 1.0-1.9 | 0.6-2.3 |
| Southeast (1981-2010 normal: 25.6°C)             |         |         |         |         |         |         |         |         |         |         |         |         |
| CMIP5                                            | 2.4     | 1.9-3.0 | 1.4-3.4 | 1.5     | 1.2-2.1 | 0.8-2.5 | 1.8     | 1.2-2.5 | 0.9-2.7 | 1.3     | 1.0-1.9 | 0.9-2.0 |
| SMME                                             | 2.4     | 1.5-3.2 | 1.4-3.5 | 1.5     | 1.1-2.1 | 0.7-2.5 | 1.7     | 1.2-2.5 | 0.9-3.1 | 1.2     | 1.0-1.8 | 0.5-2.1 |
| MCPR                                             | 2.1     | 1.6-2.9 | 1.4-3.5 | 1.4     | 1.0-2.0 | 0.9-2.2 | 1.6     | 1.1-2.2 | 0.9-2.9 | 1.3     | 0.8-1.8 | 0.6-2.0 |
| South Central (1981-2010 normal: 27.2°C)         |         |         |         |         |         |         |         |         |         |         |         |         |
| CMIP5                                            | 2.5     | 1.8-3.1 | 1.6-3.5 | 1.9     | 1.6-2.4 | 0.8-2.6 | 1.9     | 1.3-2.4 | 0.9-2.8 | 1.6     | 1.2-1.8 | 0.7-2.2 |
| SMME                                             | 2.5     | 1.6-3.4 | 1.4-3.8 | 1.6     | 1.5-2.4 | 0.7-2.5 | 1.9     | 1.3-2.7 | 0.9-2.9 | 1.6     | 1.1-1.8 | 0.6-2.2 |
| MCPR                                             | 2.1     | 1.7-3.0 | 1.3-3.9 | 1.7     | 1.3-2.2 | 1.0-2.8 | 1.7     | 1.2-2.5 | 1.0-2.9 | 1.4     | 0.8-2.0 | 0.2-2.5 |
| Upper Great Plains (1981-2010 normal: 22.1°C)    |         |         |         |         |         |         |         |         |         |         |         |         |
| CMIP5                                            | 3.0     | 1.9-3.6 | 1.6-4.0 | 1.9     | 1.4-2.5 | 0.9-2.7 | 2.2     | 1.3-3.2 | 1.0-3.3 | 1.6     | 1.1-2.4 | 1.0-2.5 |
| SMME                                             | 2.9     | 1.7-3.7 | 1.5-4.0 | 1.7     | 1.0-2.4 | 0.8-2.6 | 1.9     | 1.2-3.2 | 1.0-3.5 | 1.5     | 1.1-2.4 | 0.7-2.6 |
| MCPR                                             | 2.6     | 1.8-3.6 | 1.4-4.2 | 1.7     | 1.1-2.4 | 0.7-2.9 | 1.9     | 1.4-2.7 | 0.9-3.6 | 1.5     | 0.8-2.2 | 0.7-3.3 |
| Midwest (1981-2010 normal: 21.5°C)               |         |         |         |         |         |         |         |         |         |         |         |         |
| CMIP5                                            | 2.9     | 2.0-3.8 | 1.7-4.1 | 1.9     | 1.4-2.4 | 1.0-2.9 | 2.2     | 1.2-3.0 | 1.0-3.5 | 1.6     | 1.1-2.5 | 0.9-2.6 |
| SMME                                             | 2.9     | 1.7-3.9 | 1.6-4.3 | 1.8     | 1.1-2.2 | 0.8-2.4 | 1.8     | 1.0-3.3 | 0.9-3.7 | 1.4     | 1.1-2.3 | 0.8-2.7 |
| MCPR                                             | 2.5     | 2.0-3.4 | 1.6-3.9 | 1.7     | 1.2-2.3 | 0.7-2.7 | 1.8     | 1.3-2.6 | 0.9-3.3 | 1.5     | 0.9-2.2 | 0.6-2.9 |
| Northwest (1981-2010 normal: 18.2°C)             |         |         |         |         |         |         |         |         |         |         |         |         |
| CMIP5                                            | 2.8     | 1.9-3.5 | 1.5-4.1 | 1.7     | 1.4-2.3 | 0.9-2.9 | 1.9     | 1.2-2.9 | 0.9-3.2 | 1.6     | 1.1-2.6 | 0.9-3.0 |
| SMME                                             | 2.6     | 1.5-3.7 | 1.1-4.1 | 1.6     | 0.9-2.3 | 0.7-2.9 | 2.0     | 1.2-3.1 | 1.1-3.4 | 1.4     | 1.1-2.4 | 0.9-3.1 |
| MCPR                                             | 2.4     | 1.8-3.3 | 1.4-4.0 | 1.6     | 1.0-2.1 | 0.6-2.6 | 1.8     | 1.2-2.6 | 0.9-3.2 | 1.5     | 0.9-2.3 | 0.6-2.8 |
| California (1981-2010 normal: 23.7°C)            |         |         |         |         |         |         |         |         |         |         |         |         |
| CMIP5                                            | 2.5     | 2.0-2.8 | 1.5-3.3 | 1.5     | 1.3-1.8 | 0.7-2.7 | 1.7     | 1.3-2.4 | 0.8-2.8 | 1.3     | 1.0-2.1 | 0.9-2.6 |
| SMME                                             | 2.3     | 1.7-3.1 | 1.5-3.4 | 1.4     | 1.1-1.8 | 0.6-2.5 | 1.9     | 1.3-2.6 | 0.8-2.9 | 1.2     | 1.0-1.9 | 0.8-2.6 |
| MCPR                                             | 2.2     | 1.6-2.8 | 1.2-3.3 | 1.4     | 1.0-2.0 | 0.8-2.4 | 1.7     | 1.1-2.3 | 0.7-2.9 | 1.3     | 0.9-1.9 | 0.6-2.4 |
| Southwest (1981-2010 normal: 24.1°C)             |         |         |         |         |         |         |         |         |         |         |         |         |
| CMIP5                                            | 2.5     | 1.9-3.3 | 1.3-3.8 | 1.8     | 1.6-2.2 | 0.8-2.9 | 2.1     | 1.5-2.7 | 1.0-3.2 | 1.6     | 1.1-2.0 | 0.8-2.2 |
| SMME                                             | 2.5     | 1.9-3.4 | 1.8-4.0 | 1.8     | 1.2-2.2 | 0.6-2.8 | 1.8     | 1.5-2.8 | 1.0-3.2 | 1.7     | 1.1-2.0 | 0.7-2.3 |
| MCPR                                             | 2.3     | 1.6-3.0 | 1.3-3.9 | 1.7     | 1.3-2.2 | 0.5-2.7 | 1.9     | 1.3-2.6 | 0.8-3.2 | 1.4     | 0.8-2.1 | 0.3-2.8 |
| Rocky Mountain States (1981-2010 normal: 19.6°C) |         |         |         |         |         |         |         |         |         |         |         |         |
| CMIP5                                            | 2.9     | 1.9-3.6 | 1.6-4.0 | 1.9     | 1.5-2.3 | 1.0-3.0 | 2.1     | 1.5-2.9 | 0.9-3.2 | 1.5     | 1.2-2.5 | 1.0-2.5 |
| SMME                                             | 2.8     | 1.8-3.8 | 1.5-4.1 | 1.8     | 1.3-2.2 | 0.8-2.5 | 2.0     | 1.5-2.9 | 1.2-3.5 | 1.5     | 1.2-2.2 | 0.9-2.7 |
| MCPR                                             | 2.5     | 1.8-3.4 | 1.4-4.0 | 1.7     | 1.2-2.3 | 0.8-2.7 | 2.0     | 1.4-2.6 | 1.1-3.4 | 1.5     | 1.0-2.2 | 0.7-3.1 |
| Alaska (1981-2010 normal: 13.1°C)                |         |         |         |         |         |         |         |         |         |         |         |         |
| CMIP5                                            | 2.3     | 1.6-3.5 | 1.4-4.1 | 2.0     | 1.1-2.3 | 0.6-3.1 | 1.8     | 1.2-3.1 | 0.6-3.9 | 1.6     | 0.8-2.9 | 0.6-3.1 |
| SMME                                             | 2.1     | 1.5-3.7 | 0.6-4.3 | 1.7     | 0.8-2.3 | 0.6-3.0 | 1.8     | 1.1-2.7 | 0.6-3.7 | 1.4     | 1.1-2.6 | 0.6-3.2 |
| MCPR                                             | 2.2     | 1.5-3.1 | 1.2-3.8 | 1.6     | 0.9-2.4 | 0.7-2.8 | 1.7     | 1.1-2.4 | 0.7-3.0 | 1.6     | 0.9-2.4 | 0.4-2.8 |
| Hawaii (1981-2010 normal: 24.9°C)                |         |         |         |         |         |         |         |         |         |         |         |         |
| CMIP5                                            | 1.7     | 1.0-2.1 | 0.8-2.4 | 1.1     | 0.6-1.6 | 0.6-1.8 | 1.0     | 0.7-1.6 | 0.6-2.1 | 0.9     | 0.6-1.4 | 0.6-1.6 |
| SMME                                             | 1.5     | 0.8-2.1 | 0.6-2.6 | 1.0     | 0.6-1.6 | 0.5-1.8 | 1.0     | 0.7-1.6 | 0.6-1.9 | 0.8     | 0.6-1.4 | 0.5-1.6 |
| MCPR                                             | 1.4     | 1.1-1.9 | 0.8-2.4 | 0.9     | 0.7-1.3 | 0.5-1.6 | 1.0     | 0.7-1.5 | 0.5-1.9 | 0.9     | 0.5-1.3 | 0.3-1.9 |

TABLE A17. Projected regional SON temperature change (°C) under all RCPs for 2040-2059

| SON<br>2040-2059                                | RCP 8.5 |         |         | RCP 6.0 |         |         | RCP 4.5 |         |         | RCP 2.6 |         |         |
|-------------------------------------------------|---------|---------|---------|---------|---------|---------|---------|---------|---------|---------|---------|---------|
|                                                 | 50      | 17-83   | 5-95    | 50      | 17-83   | 5-95    | 50      | 17-83   | 5-95    | 50      | 17-83   | 5-95    |
| CONUS (1981-2010 normal: 12.6°C)                |         |         |         |         |         |         |         |         |         |         |         |         |
| CMIP5                                           | 2.6     | 2.0-3.2 | 1.6-3.5 | 1.7     | 1.4-2.1 | 1.0-2.3 | 2.0     | 1.3-2.5 | 1.0-2.8 | 1.6     | 1.2-2.2 | 1.1-2.4 |
| SMME                                            | 2.5     | 1.8-3.2 | 1.5-3.5 | 1.6     | 1.1-2.0 | 0.9-2.3 | 2.0     | 1.3-2.6 | 1.0-3.0 | 1.6     | 1.1-1.9 | 0.9-2.5 |
| MCPR                                            | 2.2     | 1.7-3.0 | 1.5-3.7 | 1.5     | 1.0-2.1 | 0.8-2.4 | 1.7     | 1.2-2.3 | 0.9-2.9 | 1.4     | 1.0-2.0 | 0.8-2.5 |
| Northeast (1981-2010 normal: 10.2°C)            |         |         |         |         |         |         |         |         |         |         |         |         |
| CMIP5                                           | 2.6     | 2.0-3.1 | 1.5-3.9 | 1.6     | 1.4-2.2 | 1.1-2.5 | 2.0     | 1.5-2.8 | 1.1-3.2 | 1.9     | 1.3-2.4 | 1.0-2.7 |
| SMME                                            | 2.5     | 1.8-3.5 | 1.2-4.0 | 1.6     | 1.2-2.2 | 0.9-2.5 | 1.9     | 1.5-3.0 | 1.1-3.3 | 1.5     | 1.1-2.1 | 0.9-2.8 |
| MCPR                                            | 2.3     | 1.7-3.1 | 1.5-3.8 | 1.5     | 1.1-2.0 | 0.9-2.4 | 1.9     | 1.4-2.5 | 0.8-3.1 | 1.5     | 1.0-2.2 | 0.6-2.8 |
| Southeast (1981-2010 normal: 17.4°C)            |         |         |         |         |         |         |         |         |         |         |         |         |
| CMIP5                                           | 2.2     | 1.6-2.9 | 1.4-3.5 | 1.5     | 1.1-1.8 | 0.7-2.4 | 1.8     | 1.3-2.4 | 0.9-2.8 | 1.4     | 1.1-1.9 | 0.9-2.2 |
| SMME                                            | 2.2     | 1.4-3.2 | 1.2-3.6 | 1.4     | 1.1-1.8 | 0.8-2.1 | 1.9     | 1.4-2.5 | 1.0-3.0 | 1.2     | 1.0-1.9 | 0.7-2.3 |
| MCPR                                            | 2.0     | 1.6-2.8 | 1.2-3.6 | 1.3     | 0.8-1.8 | 0.7-2.2 | 1.7     | 1.2-2.3 | 0.8-2.9 | 1.2     | 0.8-1.8 | 0.6-2.2 |
| South Central (1981-2010 normal: 18.3°C)        |         |         |         |         |         |         |         |         |         |         |         |         |
| CMIP5                                           | 2.5     | 1.8-3.1 | 1.4-3.2 | 1.7     | 1.4-2.0 | 0.9-2.2 | 1.9     | 1.4-2.5 | 1.0-2.8 | 1.5     | 1.2-1.9 | 1.0-2.2 |
| SMME                                            | 2.5     | 1.7-3.1 | 1.2-3.3 | 1.7     | 1.1-2.0 | 0.8-2.2 | 1.9     | 1.4-2.6 | 1.0-2.9 | 1.4     | 1.2-1.8 | 0.7-2.4 |
| MCPR                                            | 2.2     | 1.7-3.0 | 1.3-3.8 | 1.5     | 1.0-2.1 | 0.6-2.5 | 1.8     | 1.2-2.4 | 0.8-3.2 | 1.3     | 0.9-2.0 | 0.5-2.4 |
| Upper Great Plains (1981-2010 normal: 9.6°C)    |         |         |         |         |         |         |         |         |         |         |         |         |
| CMIP5                                           | 2.7     | 2.1-3.3 | 1.7-3.7 | 1.9     | 1.4-2.2 | 1.0-2.4 | 2.2     | 1.3-2.6 | 1.0-3.2 | 1.8     | 1.2-2.1 | 1.1-2.6 |
| SMME                                            | 2.7     | 1.7-3.3 | 1.5-3.7 | 1.9     | 1.1-2.2 | 0.8-2.4 | 2.2     | 1.5-2.8 | 1.0-3.4 | 1.7     | 1.1-2.1 | 1.0-2.6 |
| MCPR                                            | 2.5     | 1.8-3.1 | 1.4-4.0 | 1.6     | 1.1-2.3 | 0.6-2.7 | 1.9     | 1.3-2.6 | 0.9-3.3 | 1.6     | 1.0-2.2 | 0.6-2.6 |
| Midwest (1981-2010 normal: 10.3°C)              |         |         |         |         |         |         |         |         |         |         |         |         |
| CMIP5                                           | 2.8     | 2.1-3.3 | 1.7-3.8 | 1.9     | 1.5-2.2 | 1.0-2.8 | 2.1     | 1.5-3.0 | 1.2-3.3 | 1.8     | 1.2-2.5 | 1.1-2.8 |
| SMME                                            | 2.6     | 1.7-3.5 | 1.6-3.9 | 1.7     | 1.1-2.2 | 1.0-2.8 | 2.1     | 1.5-3.1 | 1.2-3.7 | 1.7     | 1.0-2.0 | 1.0-2.8 |
| MCPR                                            | 2.5     | 1.9-3.3 | 1.5-4.0 | 1.6     | 1.2-2.3 | 0.8-2.8 | 1.9     | 1.4-2.6 | 0.9-3.4 | 1.6     | 1.1-2.4 | 0.6-2.9 |
| Northwest (1981-2010 normal: 9.7°C)             |         |         |         |         |         |         |         |         |         |         |         |         |
| CMIP5                                           | 2.3     | 1.7-3.1 | 1.4-3.4 | 1.6     | 1.3-2.0 | 0.3-2.3 | 1.6     | 1.1-2.2 | 0.4-2.5 | 1.5     | 0.9-1.8 | 0.5-2.5 |
| SMME                                            | 2.3     | 1.4-3.1 | 1.0-3.3 | 1.4     | 0.9-2.0 | 0.3-2.2 | 1.6     | 1.0-2.3 | 0.4-2.6 | 1.4     | 0.7-1.8 | 0.4-2.7 |
| MCPR                                            | 2.1     | 1.4-2.9 | 1.0-3.5 | 1.4     | 0.8-2.0 | 0.6-2.4 | 1.4     | 0.8-2.2 | 0.3-2.9 | 1.3     | 0.8-1.9 | 0.4-2.3 |
| California (1981-2010 normal: 16.3°C)           |         |         |         |         |         |         |         |         |         |         |         |         |
| CMIP5                                           | 2.5     | 1.9-3.2 | 1.5-3.4 | 1.6     | 1.3-2.1 | 0.8-2.3 | 1.7     | 1.1-2.4 | 0.8-2.5 | 1.4     | 1.0-2.0 | 0.9-2.4 |
| SMME                                            | 2.3     | 1.5-3.1 | 1.4-3.4 | 1.6     | 0.8-2.1 | 0.7-2.3 | 1.6     | 1.0-2.4 | 0.8-2.7 | 1.4     | 1.0-1.8 | 0.5-2.4 |
| MCPR                                            | 2.2     | 1.6-3.1 | 1.1-3.4 | 1.4     | 1.0-2.0 | 0.7-2.7 | 1.5     | 0.9-2.1 | 0.6-2.8 | 1.3     | 0.8-2.0 | 0.5-2.4 |
| Southwest (1981-2010 normal: 14.6°C)            |         |         |         |         |         |         |         |         |         |         |         |         |
| CMIP5                                           | 2.7     | 2.0-3.4 | 1.8-3.6 | 1.7     | 1.4-2.2 | 0.9-2.5 | 2.1     | 1.3-2.5 | 0.9-2.9 | 1.6     | 1.2-1.9 | 0.9-2.5 |
| SMME                                            | 2.7     | 1.8-3.4 | 1.6-3.8 | 1.7     | 1.1-2.2 | 0.8-2.5 | 2.0     | 1.3-2.5 | 0.9-3.2 | 1.6     | 1.2-1.9 | 0.9-2.6 |
| MCPR                                            | 2.4     | 1.8-3.2 | 1.5-4.0 | 1.6     | 1.0-2.2 | 0.7-2.8 | 1.8     | 1.2-2.6 | 0.9-2.9 | 1.4     | 1.0-1.9 | 0.8-2.5 |
| Rocky Mountain States (1981-2010 normal: 8.4°C) |         |         |         |         |         |         |         |         |         |         |         |         |
| CMIP5                                           | 2.7     | 1.9-3.2 | 1.8-3.6 | 1.8     | 1.5-2.1 | 1.0-2.3 | 2.0     | 1.1-2.5 | 0.8-2.7 | 1.6     | 1.0-2.0 | 0.9-2.4 |
| SMME                                            | 2.6     | 1.8-3.1 | 1.5-3.4 | 1.7     | 1.0-2.1 | 0.9-2.3 | 2.0     | 1.1-2.5 | 0.8-2.9 | 1.4     | 0.9-1.9 | 0.8-2.4 |
| MCPR                                            | 2.4     | 1.7-3.1 | 1.3-3.8 | 1.5     | 1.1-2.2 | 0.8-2.7 | 1.6     | 1.1-2.3 | 0.8-3.0 | 1.4     | 0.9-1.9 | 0.6-2.5 |
| Alaska (1981-2010 normal: -2.6°C)               |         |         |         |         |         |         |         |         |         |         |         |         |
| CMIP5                                           | 3.4     | 2.3-4.0 | 1.8-4.4 | 2.1     | 1.4-2.6 | 0.6-3.4 | 2.6     | 1.7-3.2 | 0.9-4.2 | 2.0     | 1.4-2.9 | 0.9-3.3 |
| SMME                                            | 3.3     | 2.1-4.0 | 1.8-4.5 | 2.0     | 1.1-2.6 | 0.5-3.4 | 2.6     | 1.8-3.4 | 1.3-4.2 | 1.7     | 1.2-2.8 | 0.9-3.3 |
| MCPR                                            | 3.1     | 2.4-4.2 | 2.0-5.1 | 2.0     | 1.3-2.9 | 0.7-3.3 | 2.4     | 1.6-3.3 | 1.2-5.0 | 2.1     | 1.1-2.8 | 0.7-3.4 |
| Hawaii (1981-2010 normal: 24.5°C)               |         |         |         |         |         |         |         |         |         |         |         |         |
| CMIP5                                           | 1.7     | 1.1-2.3 | 0.9-2.6 | 1.0     | 0.8-1.6 | 0.6-2.0 | 1.1     | 0.8-1.7 | 0.6-2.2 | 1.0     | 0.7-1.5 | 0.6-1.7 |
| SMME                                            | 1.6     | 0.9-2.3 | 0.7-2.8 | 0.9     | 0.6-1.6 | 0.6-2.0 | 1.1     | 0.8-1.7 | 0.6-2.2 | 0.9     | 0.6-1.4 | 0.5-1.7 |
| MCPR                                            | 1.4     | 1.1-1.9 | 1.0-2.5 | 0.9     | 0.7-1.3 | 0.4-1.6 | 1.0     | 0.7-1.6 | 0.4-2.0 | 0.9     | 0.6-1.4 | 0.3-1.9 |

TABLE A18. Projected regional DJF temperature change (°C) under all RCPs for 2080-2099

| DJF<br>2080-2099                                 | RCP 8.5 |          |          | RCP 6.0 |         |         | RCP 4.5 |         |         | RCP 2.6 |         |          |
|--------------------------------------------------|---------|----------|----------|---------|---------|---------|---------|---------|---------|---------|---------|----------|
|                                                  | 50      | 17-83    | 5-95     | 50      | 17-83   | 5-95    | 50      | 17-83   | 5-95    | 50      | 17-83   | 5-95     |
| CONUS (1981-2010 normal: 0.9°C)                  |         |          |          |         |         |         |         |         |         |         |         |          |
| CMIP5                                            | 4.9     | 3.6-5.8  | 2.9-6.6  | 3.3     | 2.3-4.2 | 1.7-5.0 | 2.7     | 1.6-3.6 | 1.3-3.9 | 1.7     | 0.9-2.2 | 0.8-2.7  |
| SMME                                             | 4.9     | 3.1-6.5  | 2.9-7.5  | 3.3     | 1.7-4.5 | 1.4-5.6 | 2.3     | 1.6-3.8 | 1.3-5.1 | 1.3     | 0.6-2.1 | 0.5-3.0  |
| MCPR                                             | 4.2     | 3.3-6.3  | 2.9-8.5  | 3.0     | 2.2-4.3 | 1.6-5.8 | 2.3     | 1.6-3.6 | 1.3-4.8 | 1.2     | 0.8-2.1 | 0.4-2.7  |
| Northeast (1981-2010 normal: -3.2°C)             |         |          |          |         |         |         |         |         |         |         |         |          |
| CMIP5                                            | 5.6     | 4.0-6.7  | 3.9-7.3  | 3.9     | 2.3-4.5 | 1.5-5.6 | 3.2     | 2.0-3.9 | 1.4-4.4 | 2.0     | 1.2-2.7 | 0.5-2.8  |
| SMME                                             | 5.6     | 3.9-7.3  | 3.6-8.1  | 3.8     | 1.6-5.0 | 1.3-6.0 | 2.7     | 1.6-4.0 | 1.5-4.5 | 1.8     | 0.4-2.6 | -0.0-3.3 |
| MCPR                                             | 5.1     | 3.6-6.9  | 3.1-9.6  | 3.5     | 2.0-5.2 | 1.2-6.7 | 2.6     | 1.6-4.2 | 1.2-6.3 | 1.4     | 0.6-2.5 | 0.2-3.5  |
| Southeast (1981-2010 normal: 7.2°C)              |         |          |          |         |         |         |         |         |         |         |         |          |
| CMIP5                                            | 3.8     | 2.6-4.6  | 2.3-5.1  | 2.3     | 1.5-3.2 | 0.9-3.9 | 2.1     | 1.1-2.6 | 0.7-3.0 | 1.2     | 0.5-1.7 | 0.2-2.1  |
| SMME                                             | 3.8     | 2.5-5.0  | 2.0-5.7  | 2.3     | 1.3-3.6 | 0.8-3.9 | 2.1     | 1.0-2.7 | 0.7-3.1 | 1.1     | 0.1-1.6 | 0.1-2.1  |
| MCPR                                             | 3.5     | 2.4-5.0  | 1.8-7.0  | 2.2     | 1.1-3.6 | 0.8-4.5 | 1.7     | 0.9-2.8 | 0.5-4.4 | 0.9     | 0.2-1.7 | -0.4-2.1 |
| South Central (1981-2010 normal: 7.8°C)          |         |          |          |         |         |         |         |         |         |         |         |          |
| CMIP5                                            | 4.3     | 3.0-5.5  | 2.7-5.9  | 2.7     | 2.1-3.8 | 1.4-4.0 | 2.4     | 1.3-3.0 | 0.9-3.4 | 1.4     | 0.7-1.9 | 0.5-2.2  |
| SMME                                             | 4.3     | 2.8-5.5  | 2.5-6.1  | 2.7     | 1.6-3.8 | 1.3-4.7 | 2.3     | 1.3-3.3 | 1.1-4.3 | 1.3     | 0.4-1.9 | 0.3-2.5  |
| MCPR                                             | 4.0     | 2.7-5.7  | 2.3-8.2  | 2.7     | 1.8-4.0 | 1.5-4.7 | 2.0     | 1.2-3.2 | 0.8-4.0 | 1.1     | 0.5-1.9 | -0.1-2.6 |
| Upper Great Plains (1981-2010 normal: -4.7°C)    |         |          |          |         |         |         |         |         |         |         |         |          |
| CMIP5                                            | 5.5     | 3.9-7.2  | 2.8-8.4  | 3.8     | 2.6-5.2 | 1.8-6.8 | 3.0     | 1.7-4.5 | 0.9-5.1 | 1.8     | 0.9-2.9 | 0.6-3.7  |
| SMME                                             | 5.3     | 3.4-8.0  | 2.5-8.8  | 3.8     | 2.1-5.2 | 1.5-7.6 | 2.7     | 1.7-4.7 | 0.9-6.5 | 1.5     | 0.7-2.8 | 0.6-4.1  |
| MCPR                                             | 4.5     | 3.5-7.6  | 3.0-10.6 | 3.6     | 2.5-4.9 | 2.0-6.5 | 2.7     | 1.7-4.5 | 1.2-5.2 | 1.4     | 0.7-2.7 | 0.2-3.4  |
| Midwest (1981-2010 normal: -4.5°C)               |         |          |          |         |         |         |         |         |         |         |         |          |
| CMIP5                                            | 5.6     | 4.3-7.4  | 3.5-8.3  | 3.7     | 2.7-5.3 | 1.7-6.9 | 3.2     | 1.9-4.6 | 1.3-5.0 | 1.8     | 1.4-2.5 | 0.9-3.5  |
| SMME                                             | 5.8     | 3.8-8.3  | 3.3-9.6  | 3.7     | 2.0-5.5 | 1.4-7.4 | 3.1     | 1.9-5.0 | 1.3-6.6 | 1.6     | 0.7-2.5 | 0.4-4.0  |
| MCPR                                             | 5.0     | 4.1-7.7  | 3.4-11.2 | 3.7     | 2.5-6.0 | 1.7-7.7 | 2.8     | 2.0-4.8 | 1.2-6.1 | 1.5     | 0.8-2.5 | -0.1-3.6 |
| Northwest (1981-2010 normal: 1.1°C)              |         |          |          |         |         |         |         |         |         |         |         |          |
| CMIP5                                            | 4.4     | 3.2-5.3  | 2.5-6.2  | 2.9     | 2.2-4.2 | 1.4-4.5 | 2.2     | 1.4-3.3 | 1.1-3.9 | 1.6     | 1.1-2.5 | 0.6-2.9  |
| SMME                                             | 4.2     | 2.9-5.7  | 2.2-6.9  | 2.7     | 1.9-4.4 | 1.4-5.2 | 2.2     | 1.4-3.7 | 1.1-5.0 | 1.4     | 0.8-2.2 | 0.4-3.1  |
| MCPR                                             | 3.8     | 3.0-5.7  | 2.7-6.9  | 2.9     | 1.9-3.9 | 1.6-5.3 | 2.2     | 1.3-3.1 | 1.0-5.7 | 1.5     | 0.8-2.4 | 0.4-3.2  |
| California (1981-2010 normal: 7.7°C)             |         |          |          |         |         |         |         |         |         |         |         |          |
| CMIP5                                            | 3.8     | 2.9-4.5  | 2.4-5.0  | 2.4     | 2.1-3.4 | 1.6-3.7 | 1.8     | 1.3-2.6 | 0.8-3.1 | 1.4     | 0.8-1.9 | 0.6-2.1  |
| SMME                                             | 3.7     | 2.6-5.1  | 2.2-5.7  | 2.3     | 1.6-3.5 | 1.4-4.3 | 1.8     | 1.3-2.9 | 0.8-3.7 | 1.2     | 0.7-1.8 | 0.4-2.1  |
| MCPR                                             | 3.5     | 2.6-5.1  | 2.3-6.5  | 2.5     | 1.8-3.4 | 1.5-4.3 | 1.9     | 1.2-2.7 | 0.9-4.0 | 1.2     | 0.7-1.9 | 0.4-2.2  |
| Southwest (1981-2010 normal: 4.6°C)              |         |          |          |         |         |         |         |         |         |         |         |          |
| CMIP5                                            | 4.5     | 3.2-5.3  | 2.8-6.0  | 3.0     | 2.3-3.8 | 1.8-4.3 | 2.3     | 1.4-3.1 | 1.0-3.5 | 1.4     | 0.8-2.0 | 0.6-2.4  |
| SMME                                             | 4.3     | 2.8-6.1  | 2.6-6.9  | 2.9     | 2.0-4.1 | 1.5-4.7 | 2.0     | 1.4-3.4 | 1.0-4.5 | 1.2     | 0.7-1.9 | 0.5-2.4  |
| MCPR                                             | 3.9     | 2.9-5.9  | 2.4-7.6  | 2.8     | 2.0-3.8 | 1.8-4.9 | 2.0     | 1.4-3.1 | 1.1-3.8 | 1.2     | 0.7-2.0 | 0.5-2.6  |
| Rocky Mountain States (1981-2010 normal: -3.2°C) |         |          |          |         |         |         |         |         |         |         |         |          |
| CMIP5                                            | 4.9     | 3.9-6.1  | 2.7-7.1  | 3.4     | 2.6-4.7 | 1.8-5.7 | 2.4     | 1.5-3.7 | 1.3-4.9 | 1.9     | 1.0-2.7 | 0.8-3.2  |
| SMME                                             | 4.9     | 3.2-7.0  | 2.7-8.5  | 3.3     | 1.9-5.1 | 1.6-6.3 | 2.1     | 1.5-4.7 | 1.3-6.2 | 1.3     | 0.9-2.3 | 0.7-3.7  |
| MCPR                                             | 4.4     | 3.4-6.5  | 2.8-9.2  | 3.3     | 2.4-4.6 | 1.8-6.1 | 2.3     | 1.5-3.9 | 1.2-5.2 | 1.4     | 0.8-2.4 | 0.4-3.2  |
| Alaska (1981-2010 normal: -15.4°C)               |         |          |          |         |         |         |         |         |         |         |         |          |
| CMIP5                                            | 8.5     | 6.0-11.3 | 4.8-12.3 | 5.0     | 3.8-7.1 | 3.1-8.3 | 4.2     | 2.9-6.4 | 2.1-7.0 | 2.2     | 1.4-3.6 | 0.8-4.4  |
| SMME                                             | 8.2     | 5.8-12.1 | 4.8-13.5 | 4.8     | 3.7-7.4 | 3.2-8.9 | 4.1     | 2.9-7.0 | 2.1-8.8 | 2.4     | 1.4-3.3 | 0.8-4.7  |
| MCPR                                             | 8.2     | 6.0-11.9 | 4.7-17.0 | 5.2     | 3.7-7.8 | 2.8-9.9 | 4.4     | 2.4-6.8 | 1.7-8.2 | 2.2     | 0.9-3.9 | 0.0-5.9  |
| Hawaii (1981-2010 normal: 22.1°C)                |         |          |          |         |         |         |         |         |         |         |         |          |
| CMIP5                                            | 3.0     | 2.4-3.9  | 1.9-4.3  | 1.7     | 1.4-2.5 | 1.2-3.2 | 1.4     | 1.1-2.0 | 0.8-2.4 | 0.9     | 0.5-1.2 | 0.4-1.6  |
| SMME                                             | 2.8     | 1.9-4.1  | 1.8-4.9  | 1.6     | 1.3-2.7 | 1.1-3.4 | 1.3     | 1.1-2.2 | 0.9-2.7 | 0.8     | 0.5-1.1 | 0.4-1.6  |
| MCPR                                             | 2.8     | 2.2-4.2  | 1.9-5.2  | 1.7     | 1.3-2.5 | 1.1-3.4 | 1.4     | 0.9-2.2 | 0.8-3.0 | 0.7     | 0.5-1.3 | 0.3-1.8  |

TABLE A19. Projected regional MAM temperature change (°C) under all RCPs for 2080-2099

| MAM<br>2080-2099                                | RCP 8.5 |         |          | RCP 6.0 |         |         | RCP 4.5 |         |         | RCP 2.6 |         |         |
|-------------------------------------------------|---------|---------|----------|---------|---------|---------|---------|---------|---------|---------|---------|---------|
|                                                 | 50      | 17-83   | 5-95     | 50      | 17-83   | 5-95    | 50      | 17-83   | 5-95    | 50      | 17-83   | 5-95    |
| CONUS (1981–2010 normal: 11.4°C)                |         |         |          |         |         |         |         |         |         |         |         |         |
| CMIP5                                           | 4.6     | 3.5–5.4 | 2.9–6.3  | 2.9     | 2.4–3.8 | 1.5–4.4 | 2.5     | 1.7–3.4 | 1.2–3.8 | 1.5     | 0.9–2.3 | 0.6–2.5 |
| SMME                                            | 4.6     | 3.1–6.5 | 2.7–7.2  | 2.8     | 2.1–3.9 | 1.4–4.8 | 2.5     | 1.5–3.7 | 1.2–4.5 | 1.3     | 0.5–2.0 | 0.4–2.5 |
| MCPR                                            | 4.2     | 3.1–6.0 | 2.8–7.8  | 2.9     | 1.9–4.0 | 1.5–5.2 | 2.2     | 1.5–3.4 | 1.2–5.2 | 1.2     | 0.7–1.9 | 0.5–2.6 |
| Northeast (1981–2010 normal: 7.8°C)             |         |         |          |         |         |         |         |         |         |         |         |         |
| CMIP5                                           | 4.6     | 3.8–5.9 | 3.3–7.1  | 2.9     | 2.3–4.3 | 1.9–5.0 | 2.6     | 1.7–3.6 | 1.3–3.9 | 1.5     | 0.7–2.1 | 0.6–2.8 |
| SMME                                            | 4.5     | 3.3–7.4 | 3.2–8.8  | 2.9     | 2.0–4.3 | 1.6–5.4 | 2.5     | 1.5–3.8 | 1.4–4.2 | 1.5     | 0.6–2.0 | 0.5–2.8 |
| MCPR                                            | 4.4     | 3.2–6.5 | 2.8–8.5  | 2.9     | 1.8–4.5 | 1.5–5.5 | 2.4     | 1.6–3.4 | 1.2–5.0 | 1.3     | 0.7–2.1 | 0.2–3.0 |
| Southeast (1981–2010 normal: 16.3°C)            |         |         |          |         |         |         |         |         |         |         |         |         |
| CMIP5                                           | 4.2     | 3.5–4.9 | 2.7–5.4  | 2.6     | 2.2–3.3 | 1.7–3.6 | 2.2     | 1.4–2.8 | 1.1–3.3 | 1.3     | 0.5–1.7 | 0.4–1.8 |
| SMME                                            | 4.1     | 3.2–5.6 | 2.4–7.0  | 2.5     | 2.1–3.4 | 1.6–3.9 | 2.1     | 1.4–2.9 | 1.2–3.5 | 1.3     | 0.4–1.6 | 0.3–1.8 |
| MCPR                                            | 3.8     | 2.9–5.6 | 2.4–7.3  | 2.6     | 1.8–3.6 | 1.4–4.4 | 2.0     | 1.4–3.0 | 1.1–4.4 | 1.1     | 0.5–1.7 | 0.1–2.2 |
| South Central (1981–2010 normal: 17.7°C)        |         |         |          |         |         |         |         |         |         |         |         |         |
| CMIP5                                           | 4.6     | 3.7–5.4 | 3.2–6.0  | 3.0     | 2.4–3.6 | 1.7–4.3 | 2.4     | 1.6–3.2 | 1.1–3.4 | 1.3     | 0.6–1.9 | 0.4–1.9 |
| SMME                                            | 4.5     | 3.3–6.2 | 3.0–7.1  | 2.8     | 2.1–3.8 | 1.6–4.3 | 2.4     | 1.6–3.4 | 1.1–4.3 | 1.3     | 0.4–1.7 | 0.3–1.9 |
| MCPR                                            | 4.1     | 3.2–6.1 | 2.9–7.9  | 2.9     | 2.0–4.0 | 1.6–5.1 | 2.1     | 1.5–3.5 | 1.2–4.6 | 1.1     | 0.6–1.9 | 0.1–2.5 |
| Upper Great Plains (1981–2010 normal: 8.6°C)    |         |         |          |         |         |         |         |         |         |         |         |         |
| CMIP5                                           | 4.6     | 3.4–5.6 | 2.7–6.6  | 3.0     | 2.2–3.8 | 1.4–4.5 | 2.7     | 1.5–3.8 | 1.2–4.2 | 1.6     | 0.7–2.3 | 0.5–2.8 |
| SMME                                            | 4.6     | 2.9–6.2 | 2.5–7.1  | 2.8     | 2.1–4.4 | 1.3–4.9 | 2.7     | 1.4–3.9 | 1.3–4.9 | 1.3     | 0.5–2.2 | 0.4–2.8 |
| MCPR                                            | 4.0     | 2.9–5.9 | 2.5–8.8  | 2.8     | 1.9–4.2 | 1.4–5.2 | 2.4     | 1.5–3.6 | 1.1–5.1 | 1.2     | 0.6–2.2 | 0.4–3.2 |
| Midwest (1981–2010 normal: 8.8°C)               |         |         |          |         |         |         |         |         |         |         |         |         |
| CMIP5                                           | 4.8     | 3.6–5.9 | 3.1–7.2  | 3.0     | 2.4–4.5 | 1.8–5.2 | 2.5     | 1.6–3.6 | 1.2–4.3 | 1.5     | 0.9–2.6 | 0.3–2.9 |
| SMME                                            | 4.7     | 3.4–7.2 | 2.8–8.1  | 2.9     | 2.2–4.5 | 1.6–5.6 | 2.5     | 1.5–4.2 | 1.2–4.9 | 1.3     | 0.4–2.1 | 0.3–2.9 |
| MCPR                                            | 4.3     | 3.1–6.3 | 2.7–9.0  | 3.0     | 1.9–4.4 | 1.5–5.9 | 2.4     | 1.6–3.8 | 1.3–5.1 | 1.3     | 0.6–2.2 | 0.2–3.0 |
| Northwest (1981–2010 normal: 9.0°C)             |         |         |          |         |         |         |         |         |         |         |         |         |
| CMIP5                                           | 3.8     | 3.0–4.9 | 2.4–5.2  | 2.6     | 2.1–3.6 | 1.0–3.9 | 2.3     | 1.1–3.1 | 0.9–3.5 | 1.5     | 0.9–2.2 | 0.6–2.7 |
| SMME                                            | 3.6     | 2.4–5.2 | 1.9–5.8  | 2.4     | 1.8–3.7 | 0.9–4.3 | 2.3     | 1.1–3.1 | 0.9–4.4 | 1.2     | 0.9–2.1 | 0.5–2.9 |
| MCPR                                            | 3.5     | 2.8–5.1 | 2.4–6.0  | 2.4     | 1.7–3.5 | 1.3–4.3 | 2.0     | 1.1–3.2 | 0.8–4.5 | 1.4     | 0.7–1.9 | 0.5–2.8 |
| California (1981–2010 normal: 14.2°C)           |         |         |          |         |         |         |         |         |         |         |         |         |
| CMIP5                                           | 3.7     | 3.1–4.7 | 2.5–5.0  | 2.5     | 2.1–3.1 | 1.1–3.3 | 2.2     | 1.2–2.6 | 0.9–2.7 | 1.3     | 0.7–1.7 | 0.6–2.1 |
| SMME                                            | 3.7     | 2.5–5.2 | 2.2–5.8  | 2.5     | 1.8–3.1 | 1.0–3.8 | 2.2     | 1.2–2.7 | 0.9–3.3 | 1.1     | 0.6–1.7 | 0.3–2.1 |
| MCPR                                            | 3.5     | 2.7–5.2 | 2.3–6.2  | 2.2     | 1.6–3.3 | 1.3–4.4 | 1.8     | 1.2–2.7 | 0.8–4.1 | 1.1     | 0.7–1.7 | 0.3–2.1 |
| Southwest (1981–2010 normal: 13.4°C)            |         |         |          |         |         |         |         |         |         |         |         |         |
| CMIP5                                           | 4.8     | 3.6–5.8 | 3.2–6.6  | 3.1     | 2.5–3.5 | 1.6–4.8 | 2.6     | 1.5–3.2 | 1.2–4.1 | 1.3     | 0.7–2.1 | 0.5–2.5 |
| SMME                                            | 4.8     | 3.5–7.2 | 3.1–8.1  | 3.0     | 2.3–4.0 | 1.5–5.0 | 2.5     | 1.5–3.5 | 1.2–4.5 | 1.2     | 0.5–2.0 | 0.5–2.5 |
| MCPR                                            | 4.4     | 3.4–6.4 | 2.9–8.0  | 2.8     | 2.0–4.2 | 1.7–5.7 | 2.1     | 1.6–3.6 | 1.1–5.2 | 1.1     | 0.6–1.9 | 0.3–2.5 |
| Rocky Mountain States (1981–2010 normal: 7.6°C) |         |         |          |         |         |         |         |         |         |         |         |         |
| CMIP5                                           | 4.6     | 3.5–5.8 | 2.8–6.8  | 3.2     | 2.5–3.9 | 1.1–5.2 | 2.6     | 1.4–3.5 | 1.1–4.6 | 1.6     | 1.1–2.8 | 0.6–3.5 |
| SMME                                            | 4.6     | 2.8–7.2 | 2.2–8.0  | 3.2     | 2.2–4.4 | 1.0–5.6 | 2.6     | 1.4–4.2 | 1.1–5.2 | 1.4     | 0.6–2.5 | 0.3–3.5 |
| MCPR                                            | 4.2     | 3.1–6.1 | 2.7–8.1  | 3.0     | 1.9–4.5 | 1.4–5.8 | 2.4     | 1.4–3.8 | 1.2–5.8 | 1.4     | 0.8–2.2 | 0.6–3.2 |
| Alaska (1981–2010 normal: -1.9°C)               |         |         |          |         |         |         |         |         |         |         |         |         |
| CMIP5                                           | 6.5     | 4.3–9.0 | 2.9–9.4  | 3.9     | 2.9–5.3 | 2.1–6.7 | 3.4     | 1.7–4.8 | 0.8–5.4 | 2.3     | 1.2–3.8 | 0.4–4.1 |
| SMME                                            | 5.6     | 3.6–9.1 | 2.8–10.1 | 3.6     | 2.5–5.7 | 2.0–7.1 | 2.7     | 1.5–5.2 | 0.8–6.4 | 2.6     | 1.0–3.5 | 0.0–4.1 |
| MCPR                                            | 5.9     | 4.3–8.7 | 3.4–12.0 | 3.9     | 2.7–5.5 | 2.0–7.3 | 3.2     | 1.9–4.8 | 1.3–6.1 | 1.7     | 0.8–3.4 | 0.3–4.5 |
| Hawaii (1981–2010 normal: 22.8°C)               |         |         |          |         |         |         |         |         |         |         |         |         |
| CMIP5                                           | 2.9     | 2.5–3.8 | 1.9–4.4  | 1.8     | 1.4–2.8 | 1.0–3.1 | 1.5     | 1.0–1.9 | 0.9–2.3 | 0.9     | 0.6–1.3 | 0.5–1.5 |
| SMME                                            | 2.9     | 2.0–3.9 | 1.6–4.8  | 1.7     | 1.2–2.8 | 1.0–3.3 | 1.3     | 1.0–2.1 | 0.9–2.4 | 0.8     | 0.5–1.2 | 0.5–1.5 |
| MCPR                                            | 2.7     | 2.1–4.2 | 2.0–5.3  | 1.7     | 1.2–2.6 | 1.1–3.4 | 1.4     | 0.9–2.1 | 0.7–2.8 | 0.8     | 0.4–1.4 | 0.2–1.8 |

TABLE A20. Projected regional SON temperature change (°C) under all RCPs for 2080-2099

| SON<br>2080-2099                                | RCP 8.5 |         |          | RCP 6.0 |         |         | RCP 4.5 |         |         | RCP 2.6 |         |         |
|-------------------------------------------------|---------|---------|----------|---------|---------|---------|---------|---------|---------|---------|---------|---------|
|                                                 | 50      | 17-83   | 5-95     | 50      | 17-83   | 5-95    | 50      | 17-83   | 5-95    | 50      | 17-83   | 5-95    |
| CONUS (1981-2010 normal: 12.6°C)                |         |         |          |         |         |         |         |         |         |         |         |         |
| CMIP5                                           | 5.4     | 4.2-6.6 | 3.6-7.0  | 3.5     | 2.8-4.2 | 1.4-4.6 | 2.6     | 1.8-3.6 | 1.4-4.1 | 1.5     | 1.1-2.4 | 0.6-2.6 |
| SMME                                            | 5.3     | 3.6-7.0 | 3.4-8.9  | 3.1     | 2.5-4.4 | 1.3-5.3 | 2.5     | 1.8-4.0 | 1.4-4.7 | 1.4     | 0.5-2.0 | 0.5-3.0 |
| MCPR                                            | 5.0     | 3.8-7.1 | 3.4-8.6  | 3.2     | 2.1-4.5 | 1.9-5.6 | 2.4     | 1.7-3.6 | 1.3-4.6 | 1.3     | 0.8-2.1 | 0.7-2.7 |
| Northeast (1981-2010 normal: 10.2°C)            |         |         |          |         |         |         |         |         |         |         |         |         |
| CMIP5                                           | 5.2     | 4.2-6.6 | 3.7-7.8  | 3.5     | 2.7-4.4 | 1.5-5.0 | 2.6     | 1.7-3.6 | 1.3-4.4 | 1.6     | 0.8-2.3 | 0.5-2.9 |
| SMME                                            | 5.1     | 3.8-7.1 | 2.8-8.8  | 3.0     | 2.5-4.6 | 1.4-5.4 | 2.4     | 1.6-4.1 | 1.3-4.8 | 1.4     | 0.4-2.1 | 0.3-3.1 |
| MCPR                                            | 4.9     | 3.7-7.2 | 3.3-9.2  | 3.3     | 2.3-4.6 | 1.8-5.4 | 2.5     | 1.7-3.9 | 1.3-4.7 | 1.3     | 0.7-2.2 | 0.4-3.0 |
| Southeast (1981-2010 normal: 17.4°C)            |         |         |          |         |         |         |         |         |         |         |         |         |
| CMIP5                                           | 4.8     | 3.8-6.0 | 3.2-7.0  | 2.9     | 2.5-3.8 | 1.4-4.7 | 2.2     | 1.7-3.4 | 1.2-4.0 | 1.3     | 0.8-1.9 | 0.4-2.5 |
| SMME                                            | 4.8     | 3.3-6.4 | 2.9-8.0  | 2.9     | 2.3-4.0 | 1.3-5.0 | 2.2     | 1.6-3.8 | 1.3-4.4 | 1.1     | 0.4-1.9 | 0.4-2.6 |
| MCPR                                            | 4.5     | 3.4-6.7 | 3.0-8.1  | 2.9     | 2.0-4.2 | 1.6-5.0 | 2.3     | 1.6-3.4 | 1.2-4.5 | 1.1     | 0.6-1.6 | 0.3-2.4 |
| South Central (1981-2010 normal: 18.3°C)        |         |         |          |         |         |         |         |         |         |         |         |         |
| CMIP5                                           | 5.3     | 4.1-6.0 | 3.4-6.5  | 3.2     | 2.8-3.9 | 1.3-4.8 | 2.6     | 1.7-3.3 | 1.3-4.2 | 1.4     | 1.0-2.3 | 0.5-2.4 |
| SMME                                            | 5.3     | 3.7-6.5 | 3.4-8.2  | 3.2     | 2.6-4.1 | 1.2-4.9 | 2.6     | 1.9-3.7 | 1.3-4.7 | 1.3     | 0.1-2.0 | 0.1-3.0 |
| MCPR                                            | 4.9     | 3.8-7.1 | 3.3-9.4  | 3.1     | 2.1-4.5 | 1.7-5.5 | 2.3     | 1.7-3.8 | 1.3-4.9 | 1.3     | 0.8-1.9 | 0.3-2.6 |
| Upper Great Plains (1981-2010 normal: 9.6°C)    |         |         |          |         |         |         |         |         |         |         |         |         |
| CMIP5                                           | 6.0     | 4.2-7.0 | 3.8-7.5  | 3.8     | 3.0-4.5 | 1.3-4.7 | 3.0     | 1.7-3.8 | 1.4-4.7 | 1.8     | 1.1-2.6 | 0.6-3.0 |
| SMME                                            | 6.0     | 4.0-7.5 | 3.5-9.2  | 3.5     | 2.4-4.6 | 1.2-5.7 | 2.6     | 1.7-4.2 | 1.5-5.5 | 1.5     | 0.4-2.2 | 0.4-3.1 |
| MCPR                                            | 5.3     | 4.0-7.6 | 3.7-9.8  | 3.4     | 2.2-4.7 | 1.8-6.1 | 2.6     | 1.8-3.9 | 1.3-5.4 | 1.5     | 0.9-2.2 | 0.6-3.1 |
| Midwest (1981-2010 normal: 10.3°C)              |         |         |          |         |         |         |         |         |         |         |         |         |
| Stab:tas CMIP5                                  | 5.6     | 4.4-7.1 | 3.8-7.7  | 3.6     | 3.0-4.7 | 1.4-5.2 | 2.9     | 1.8-4.0 | 1.4-4.7 | 1.7     | 1.0-2.7 | 0.5-3.3 |
| SMME                                            | 5.6     | 4.0-7.8 | 3.5-9.4  | 3.3     | 2.5-4.7 | 1.3-6.0 | 2.7     | 1.6-4.7 | 1.6-5.5 | 1.6     | 0.4-2.2 | 0.4-3.4 |
| MCPR                                            | 5.3     | 4.0-7.5 | 3.6-9.3  | 3.4     | 2.2-4.8 | 1.9-5.9 | 2.7     | 1.8-3.9 | 1.3-5.3 | 1.5     | 0.9-2.4 | 0.5-3.3 |
| Northwest (1981-2010 normal: 9.7°C)             |         |         |          |         |         |         |         |         |         |         |         |         |
| CMIP5                                           | 4.8     | 3.5-6.1 | 2.8-6.4  | 3.3     | 2.0-3.8 | 1.5-4.3 | 2.4     | 1.4-3.4 | 0.7-3.9 | 1.3     | 1.1-2.3 | 0.8-2.5 |
| SMME                                            | 4.5     | 2.8-6.4 | 2.1-7.2  | 3.3     | 1.5-4.0 | 1.3-4.6 | 2.3     | 1.1-3.6 | 1.0-4.3 | 1.2     | 1.0-1.9 | 0.6-2.5 |
| MCPR                                            | 4.6     | 3.1-6.3 | 2.6-7.8  | 2.8     | 1.8-4.1 | 1.5-5.3 | 2.2     | 1.4-3.3 | 0.9-4.3 | 1.3     | 0.7-2.1 | 0.4-2.6 |
| California (1981-2010 normal: 16.3°C)           |         |         |          |         |         |         |         |         |         |         |         |         |
| CMIP5                                           | 5.1     | 3.9-6.2 | 2.9-6.7  | 3.3     | 2.2-4.1 | 1.4-4.3 | 2.3     | 1.7-3.3 | 1.3-4.0 | 1.5     | 0.9-2.3 | 0.8-2.6 |
| SMME                                            | 4.8     | 3.5-6.8 | 2.9-8.2  | 3.0     | 1.8-4.1 | 1.2-4.8 | 2.3     | 1.5-3.6 | 1.4-4.1 | 1.3     | 0.9-1.7 | 0.4-2.6 |
| MCPR                                            | 4.7     | 3.4-6.9 | 2.9-8.2  | 2.8     | 2.1-4.0 | 1.8-5.2 | 2.3     | 1.6-3.3 | 1.1-4.6 | 1.2     | 0.7-2.1 | 0.5-2.5 |
| Southwest (1981-2010 normal: 14.6°C)            |         |         |          |         |         |         |         |         |         |         |         |         |
| CMIP5                                           | 5.5     | 4.4-6.7 | 4.1-7.2  | 3.3     | 2.8-4.3 | 1.3-4.6 | 2.8     | 1.8-3.7 | 1.5-4.0 | 1.5     | 1.0-2.3 | 0.5-2.6 |
| SMME                                            | 5.1     | 4.1-7.0 | 3.6-8.8  | 3.2     | 2.4-4.3 | 1.2-5.4 | 2.5     | 1.7-3.8 | 1.6-4.8 | 1.3     | 0.8-2.2 | 0.5-2.9 |
| MCPR                                            | 5.1     | 4.0-7.5 | 3.4-9.6  | 3.2     | 2.3-4.7 | 1.9-5.7 | 2.6     | 1.7-3.9 | 1.2-5.0 | 1.4     | 0.8-2.1 | 0.7-2.8 |
| Rocky Mountain States (1981-2010 normal: 8.4°C) |         |         |          |         |         |         |         |         |         |         |         |         |
| CMIP5                                           | 5.7     | 4.1-6.7 | 3.3-7.2  | 3.5     | 2.5-4.2 | 1.4-4.5 | 2.7     | 1.7-3.8 | 1.3-4.1 | 1.4     | 1.1-2.4 | 0.8-2.6 |
| SMME                                            | 5.2     | 3.6-7.3 | 3.2-8.6  | 3.5     | 2.1-4.4 | 1.3-5.2 | 2.6     | 1.6-4.0 | 1.4-4.8 | 1.4     | 0.8-1.9 | 0.5-2.7 |
| MCPR                                            | 5.0     | 3.8-7.2 | 3.3-9.1  | 3.2     | 2.3-4.5 | 1.8-5.7 | 2.5     | 1.6-3.8 | 1.2-4.6 | 1.4     | 0.8-2.2 | 0.6-2.8 |
| Alaska (1981-2010 normal: -2.6°C)               |         |         |          |         |         |         |         |         |         |         |         |         |
| CMIP5                                           | 6.3     | 4.8-7.3 | 3.4-7.8  | 4.0     | 2.9-4.7 | 1.7-5.4 | 3.3     | 2.2-4.2 | 1.4-5.1 | 2.2     | 1.3-2.8 | 0.4-2.9 |
| SMME                                            | 6.2     | 4.5-7.4 | 3.1-9.1  | 3.9     | 2.6-4.8 | 1.7-5.8 | 3.1     | 2.2-4.4 | 1.4-5.6 | 2.1     | 1.3-2.8 | 0.4-2.9 |
| MCPR                                            | 6.1     | 4.1-8.1 | 3.4-11.2 | 4.0     | 2.5-5.7 | 2.1-6.6 | 3.1     | 2.3-4.4 | 1.3-7.4 | 1.8     | 1.0-2.7 | 0.5-4.5 |
| Hawaii (1981-2010 normal: 24.5°C)               |         |         |          |         |         |         |         |         |         |         |         |         |
| CMIP5                                           | 3.1     | 2.5-4.6 | 2.2-5.4  | 2.1     | 1.4-3.1 | 1.2-3.8 | 1.6     | 1.1-2.4 | 0.7-3.2 | 1.0     | 0.6-1.6 | 0.5-2.2 |
| SMME                                            | 3.0     | 2.2-4.9 | 1.8-5.9  | 1.7     | 1.2-3.1 | 1.2-4.0 | 1.5     | 1.1-2.6 | 0.8-3.3 | 0.8     | 0.5-1.5 | 0.4-2.2 |
| MCPR                                            | 3.0     | 2.4-4.5 | 2.0-6.1  | 1.9     | 1.4-2.8 | 1.2-3.7 | 1.6     | 0.9-2.2 | 0.6-3.5 | 0.8     | 0.5-1.5 | 0.3-2.2 |

TABLE A21. Projected number of days with maximum daily temperature greater than 35°C (population-weighted using county population) under all RCPs for 2040-2059

| 2040-2059                                           | RCP 8.5 |             |             | RCP 6.0 |             |             | RCP 4.5 |             |             | RCP 2.6 |             |             |
|-----------------------------------------------------|---------|-------------|-------------|---------|-------------|-------------|---------|-------------|-------------|---------|-------------|-------------|
|                                                     | 50      | 17-83       | 5-95        | 50      | 17-83       | 5-95        | 50      | 17-83       | 5-95        | 50      | 17-83       | 5-95        |
| CONUS (1981-2010 normal: 14.9 days)                 |         |             |             |         |             |             |         |             |             |         |             |             |
| CMIP5                                               | 38.1    | 32.4-47.2   | 26.4-51.1   | 28.7    | 26.5-34.9   | 21.0-36.9   | 31.8    | 24.7-39.8   | 21.7-43.6   | 26.7    | 23.2-33.5   | 22.9-35.6   |
| SMME                                                | 38.1    | 26.7-49.8   | 25.3-54.8   | 28.5    | 25.6-34.0   | 18.5-36.0   | 31.2    | 24.7-40.5   | 21.7-45.8   | 25.8    | 23.2-31.9   | 19.7-37.2   |
| MCPR                                                | 34.6    | 29.9-44.4   | 28.0-50.5   | 28.1    | 24.7-33.1   | 23.4-36.7   | 29.8    | 25.8-37.9   | 22.8-44.0   | 26.0    | 22.6-30.7   | 20.1-35.5   |
| Northeast (1981-2010 normal: 2.6 days)              |         |             |             |         |             |             |         |             |             |         |             |             |
| CMIP5                                               | 13.4    | 9.8-17.6    | 6.6-22.1    | 7.2     | 5.4-11.0    | 4.3-13.4    | 9.0     | 6.0-13.0    | 4.4-16.5    | 7.0     | 4.7-9.5     | 4.0-9.8     |
| SMME                                                | 11.3    | 7.3-18.3    | 4.3-26.8    | 6.1     | 4.6-9.1     | 4.1-12.7    | 9.0     | 5.9-14.8    | 4.4-18.8    | 6.8     | 5.3-9.3     | 3.8-11.0    |
| MCPR                                                | 11.9    | 8.3-17.4    | 7.2-24.2    | 7.2     | 5.4-10.1    | 4.1-12.4    | 8.0     | 6.2-11.8    | 5.2-16.6    | 6.3     | 4.8-9.7     | 3.8-11.6    |
| Southeast (1981-2010 normal: 8.2 days)              |         |             |             |         |             |             |         |             |             |         |             |             |
| CMIP5                                               | 42.1    | 32.1-57.8   | 24.5-63.1   | 28.1    | 21.8-39.1   | 17.9-41.0   | 31.3    | 22.1-42.7   | 19.6-50.4   | 23.5    | 19.6-36.3   | 17.5-41.1   |
| SMME                                                | 39.8    | 24.7-60.6   | 23.2-68.2   | 28.1    | 21.5-38.9   | 15.3-40.5   | 31.3    | 23.6-42.7   | 19.6-52.7   | 21.9    | 19.5-33.9   | 16.9-41.1   |
| MCPR                                                | 37.7    | 28.2-50.9   | 26.0-62.4   | 26.9    | 21.5-35.2   | 18.8-42.3   | 29.6    | 23.7-41.0   | 18.8-50.6   | 22.8    | 17.6-31.6   | 15.8-37.1   |
| South Central (1981-2010 normal: 35.7 days)         |         |             |             |         |             |             |         |             |             |         |             |             |
| CMIP5                                               | 81.5    | 68.7-91.0   | 60.1-100.6  | 73.2    | 64.7-78.4   | 49.9-86.0   | 73.9    | 59.4-87.7   | 52.7-90.6   | 65.8    | 57.5-72.5   | 49.4-80.7   |
| SMME                                                | 81.5    | 63.7-98.4   | 53.7-105.7  | 71.7    | 64.0-79.3   | 41.9-85.3   | 74.7    | 59.4-88.9   | 52.7-97.6   | 65.8    | 56.7-70.4   | 49.4-80.7   |
| MCPR                                                | 76.8    | 67.8-93.2   | 62.4-104.3  | 68.9    | 62.0-78.3   | 56.7-87.4   | 69.4    | 60.4-82.5   | 54.2-96.0   | 62.8    | 51.0-74.0   | 43.6-83.8   |
| Upper Great Plains (1981-2010 normal: 12.5 days)    |         |             |             |         |             |             |         |             |             |         |             |             |
| CMIP5                                               | 38.9    | 28.0-47.2   | 22.6-51.2   | 29.8    | 25.1-32.6   | 19.1-37.6   | 30.8    | 23.4-39.0   | 19.4-45.3   | 26.1    | 22.0-32.7   | 20.1-35.9   |
| SMME                                                | 37.9    | 25.7-47.5   | 21.1-54.3   | 28.3    | 23.3-31.9   | 18.0-32.9   | 30.7    | 23.7-43.4   | 19.6-48.4   | 25.8    | 22.0-31.7   | 18.4-35.9   |
| MCPR                                                | 34.7    | 27.7-44.3   | 24.0-49.6   | 27.2    | 22.4-33.2   | 18.5-38.3   | 28.9    | 23.4-37.8   | 19.6-45.6   | 24.6    | 19.7-31.9   | 16.4-39.7   |
| Midwest (1981-2010 normal: 2.7 days)                |         |             |             |         |             |             |         |             |             |         |             |             |
| CMIP5                                               | 19.0    | 11.7-25.7   | 8.4-38.1    | 11.1    | 9.3-13.9    | 6.1-16.7    | 12.1    | 7.2-23.3    | 6.3-25.5    | 9.6     | 7.6-15.2    | 5.3-18.2    |
| SMME                                                | 19.0    | 9.2-28.6    | 7.3-33.5    | 10.3    | 7.4-13.7    | 5.5-15.9    | 11.5    | 7.2-24.8    | 6.3-30.6    | 9.2     | 7.6-12.5    | 5.3-18.2    |
| MCPR                                                | 15.5    | 11.3-23.6   | 9.5-27.8    | 10.2    | 7.5-14.0    | 6.0-17.2    | 11.2    | 7.8-17.8    | 6.5-24.2    | 8.8     | 6.4-13.6    | 5.1-17.9    |
| Northwest (1981-2010 normal: 3.5 days)              |         |             |             |         |             |             |         |             |             |         |             |             |
| CMIP5                                               | 12.5    | 9.5-15.0    | 7.2-17.3    | 8.1     | 6.9-9.7     | 5.8-11.8    | 9.4     | 6.9-12.1    | 5.8-14.9    | 8.0     | 6.6-11.7    | 5.8-13.5    |
| SMME                                                | 12.0    | 9.5-16.0    | 6.5-18.7    | 8.0     | 6.5-9.4     | 4.9-11.0    | 9.4     | 7.0-13.7    | 6.1-15.1    | 7.7     | 6.6-10.4    | 4.7-14.8    |
| MCPR                                                | 10.9    | 8.5-14.7    | 7.5-17.9    | 7.6     | 5.9-10.0    | 5.1-12.0    | 8.5     | 6.9-11.3    | 6.1-14.5    | 7.9     | 6.2-10.5    | 5.5-11.8    |
| California (1981-2010 normal: 31.6 days)            |         |             |             |         |             |             |         |             |             |         |             |             |
| CMIP5                                               | 48.6    | 43.4-52.8   | 40.9-54.9   | 40.5    | 39.0-43.5   | 34.3-50.7   | 43.1    | 38.7-47.2   | 36.2-54.0   | 40.0    | 36.7-44.9   | 35.9-49.9   |
| SMME                                                | 48.4    | 41.0-54.5   | 39.7-60.3   | 40.3    | 38.4-43.2   | 30.9-48.0   | 43.7    | 38.7-47.9   | 36.2-56.9   | 39.6    | 36.7-43.4   | 35.6-49.9   |
| MCPR                                                | 46.0    | 41.4-52.5   | 38.2-58.6   | 40.6    | 37.1-44.8   | 35.1-49.4   | 41.9    | 38.1-48.3   | 35.4-53.6   | 39.3    | 36.1-43.9   | 34.3-47.3   |
| Southwest (1981-2010 normal: 92.0 days)             |         |             |             |         |             |             |         |             |             |         |             |             |
| CMIP5                                               | 125.9   | 115.5-132.6 | 111.4-138.2 | 114.7   | 113.8-118.8 | 102.8-128.7 | 118.4   | 109.9-122.7 | 105.2-131.0 | 112.9   | 107.3-118.7 | 103.8-122.1 |
| SMME                                                | 125.9   | 114.9-138.2 | 109.2-145.5 | 114.7   | 111.0-118.8 | 98.0-120.9  | 118.7   | 109.9-125.8 | 107.2-133.9 | 111.8   | 107.3-117.7 | 100.8-125.0 |
| MCPR                                                | 120.8   | 113.0-131.5 | 109.7-139.5 | 112.8   | 107.2-120.3 | 103.4-126.6 | 115.8   | 108.5-124.6 | 104.9-133.5 | 110.4   | 104.9-116.6 | 98.8-123.3  |
| Rocky Mountain States (1981-2010 normal: 23.0 days) |         |             |             |         |             |             |         |             |             |         |             |             |
| CMIP5                                               | 46.9    | 40.8-53.2   | 36.0-59.6   | 38.5    | 36.1-41.7   | 29.6-49.1   | 40.7    | 35.2-44.6   | 32.3-51.9   | 35.5    | 32.0-41.3   | 31.3-44.5   |
| SMME                                                | 46.9    | 40.0-53.8   | 33.2-63.4   | 37.7    | 33.5-40.9   | 26.5-43.0   | 41.2    | 35.6-47.4   | 32.3-59.3   | 35.3    | 32.0-39.5   | 29.2-44.5   |
| MCPR                                                | 43.5    | 38.1-52.5   | 35.2-56.8   | 36.9    | 32.8-42.0   | 30.8-46.0   | 38.8    | 35.2-46.4   | 32.5-51.5   | 35.1    | 31.1-39.9   | 28.2-46.3   |
| Alaska (1981-2010 normal: 0.0 days)                 |         |             |             |         |             |             |         |             |             |         |             |             |
| CMIP5                                               | 0.1     | 0.0-0.3     | 0.0-0.7     | 0.0     | 0.0-0.1     | 0.0-0.2     | 0.0     | 0.0-0.1     | 0.0-0.5     | 0.0     | 0.0-0.2     | 0.0-0.4     |
| SMME                                                | 0.0     | 0.0-0.4     | 0.0-0.7     | 0.0     | 0.0-0.1     | 0.0-0.2     | 0.0     | 0.0-0.1     | 0.0-0.4     | 0.0     | 0.0-0.1     | 0.0-0.4     |
| MCPR                                                | 0.1     | 0.0-0.2     | 0.0-0.3     | 0.0     | 0.0-0.1     | 0.0-0.2     | 0.0     | 0.0-0.1     | 0.0-0.2     | 0.0     | 0.0-0.1     | 0.0-0.2     |
| Hawaii (1981-2010 normal: 0.0 days)                 |         |             |             |         |             |             |         |             |             |         |             |             |
| CMIP5                                               | 0.3     | 0.1-2.2     | 0.0-9.0     | 0.0     | 0.0-0.2     | 0.0-0.8     | 0.1     | 0.0-0.4     | 0.0-1.6     | 0.0     | 0.0-0.2     | 0.0-0.5     |
| SMME                                                | 0.3     | 0.0-2.0     | 0.0-6.8     | 0.0     | 0.0-0.2     | 0.0-0.5     | 0.0     | 0.0-0.2     | 0.0-1.3     | 0.0     | 0.0-0.1     | 0.0-0.5     |
| MCPR                                                | 0.3     | 0.1-1.3     | 0.0-4.7     | 0.1     | 0.0-0.2     | 0.0-0.4     | 0.1     | 0.0-0.4     | 0.0-1.4     | 0.1     | 0.0-0.2     | 0.0-0.8     |

TABLE A22. Projected number of days with minimum daily temperature less than 0°C (population-weighted using county population) under all RCPs for 2040-2059. Note that ranges are presented as cool to warm.

| 2040-2059                                            | RCP 8.5 |             |             | RCP 6.0 |             |             | RCP 4.5 |             |             | RCP 2.6 |             |             |
|------------------------------------------------------|---------|-------------|-------------|---------|-------------|-------------|---------|-------------|-------------|---------|-------------|-------------|
|                                                      | 50      | 83-17       | 95-5        | 50      | 83-17       | 95-5        | 50      | 83-17       | 95-5        | 50      | 83-17       | 95-5        |
| CONUS (1981-2010 normal: 74.1 days)                  |         |             |             |         |             |             |         |             |             |         |             |             |
| CMIP5                                                | 54.2    | 59.6-50.6   | 65.7-46.0   | 62.5    | 66.1-60.2   | 68.1-52.2   | 60.0    | 64.0-56.4   | 66.6-50.5   | 62.8    | 67.1-58.5   | 68.0-56.3   |
| SMME                                                 | 54.2    | 62.1-49.3   | 66.5-41.3   | 64.8    | 67.4-59.8   | 69.4-52.7   | 60.2    | 63.9-51.0   | 66.6-48.1   | 63.8    | 68.5-58.7   | 70.7-52.2   |
| MCPR                                                 | 57.0    | 61.5-51.1   | 65.2-43.3   | 64.0    | 66.8-59.8   | 68.9-53.6   | 61.4    | 64.2-55.8   | 66.5-50.7   | 64.2    | 68.7-58.1   | 71.6-54.6   |
| Northeast (1981-2010 normal: 102.9 days)             |         |             |             |         |             |             |         |             |             |         |             |             |
| CMIP5                                                | 74.3    | 84.7-70.8   | 90.7-63.2   | 88.6    | 93.1-82.7   | 94.8-69.7   | 82.7    | 88.7-78.3   | 94.0-68.5   | 87.1    | 94.2-80.1   | 95.5-75.5   |
| SMME                                                 | 76.1    | 86.7-65.9   | 92.3-53.2   | 89.2    | 93.7-82.9   | 96.9-69.7   | 82.7    | 88.7-73.0   | 93.8-65.1   | 89.9    | 95.9-81.4   | 99.7-70.1   |
| MCPR                                                 | 79.0    | 85.0-69.4   | 90.0-57.5   | 88.7    | 93.3-80.8   | 96.3-73.3   | 84.1    | 90.0-77.2   | 93.4-66.3   | 89.4    | 97.5-79.3   | 103.5-73.6  |
| Southeast (1981-2010 normal: 47.3 days)              |         |             |             |         |             |             |         |             |             |         |             |             |
| CMIP5                                                | 33.0    | 39.5-30.4   | 42.3-29.3   | 40.5    | 42.9-37.6   | 44.1-34.9   | 37.3    | 40.9-34.3   | 43.5-31.3   | 38.9    | 43.4-36.8   | 44.3-34.8   |
| SMME                                                 | 33.0    | 39.7-30.0   | 43.3-27.4   | 41.1    | 43.8-38.0   | 44.8-36.9   | 37.3    | 40.6-33.5   | 41.7-31.3   | 41.2    | 43.4-37.1   | 46.3-34.5   |
| MCPR                                                 | 35.7    | 39.3-30.4   | 41.4-24.4   | 40.4    | 43.5-36.9   | 45.4-33.7   | 37.8    | 41.4-33.3   | 44.2-28.9   | 40.1    | 44.2-36.0   | 48.6-32.2   |
| South Central (1981-2010 normal: 30.3 days)          |         |             |             |         |             |             |         |             |             |         |             |             |
| CMIP5                                                | 19.7    | 24.0-17.7   | 27.6-16.8   | 25.4    | 28.3-23.6   | 30.1-21.4   | 23.9    | 26.1-22.2   | 27.3-17.4   | 25.7    | 27.0-22.9   | 28.3-22.2   |
| SMME                                                 | 20.6    | 25.0-17.2   | 28.2-16.0   | 26.3    | 29.3-23.6   | 33.4-21.4   | 23.7    | 25.9-21.3   | 27.3-15.2   | 25.9    | 27.0-22.9   | 31.5-21.0   |
| MCPR                                                 | 21.7    | 25.5-18.7   | 29.0-14.6   | 26.7    | 28.9-23.9   | 30.7-21.5   | 24.7    | 27.5-20.9   | 28.6-19.4   | 27.0    | 29.5-23.1   | 32.1-20.7   |
| Upper Great Plains (1981-2010 normal: 130.6 days)    |         |             |             |         |             |             |         |             |             |         |             |             |
| CMIP5                                                | 108.9   | 116.8-98.2  | 120.9-94.2  | 116.8   | 123.0-112.2 | 125.7-106.4 | 115.1   | 120.6-107.7 | 122.9-98.6  | 117.6   | 123.9-111.4 | 124.1-109.8 |
| SMME                                                 | 109.4   | 119.1-97.4  | 121.5-93.4  | 119.2   | 123.8-110.7 | 126.5-106.8 | 115.1   | 120.3-102.6 | 122.0-91.9  | 121.0   | 122.8-111.1 | 124.7-106.9 |
| MCPR                                                 | 110.0   | 117.9-101.1 | 122.5-85.0  | 118.9   | 122.9-112.8 | 125.6-107.5 | 115.5   | 120.1-107.7 | 123.9-101.3 | 119.4   | 123.5-112.1 | 128.2-106.6 |
| Midwest (1981-2010 normal: 122.4 days)               |         |             |             |         |             |             |         |             |             |         |             |             |
| CMIP5                                                | 93.8    | 102.0-86.5  | 107.8-78.1  | 106.6   | 112.0-100.9 | 113.4-89.4  | 102.1   | 106.7-94.3  | 111.8-86.0  | 105.8   | 112.6-98.8  | 114.3-95.7  |
| SMME                                                 | 96.0    | 106.1-85.6  | 109.4-70.8  | 109.4   | 113.4-99.9  | 115.3-90.2  | 102.8   | 106.7-86.7  | 111.3-81.4  | 108.3   | 114.3-99.6  | 114.9-90.2  |
| MCPR                                                 | 97.9    | 104.3-89.3  | 109.9-74.5  | 107.7   | 112.7-99.8  | 116.5-90.9  | 103.4   | 108.4-93.8  | 111.6-87.6  | 107.5   | 113.9-98.7  | 118.0-94.5  |
| Northwest (1981-2010 normal: 63.3 days)              |         |             |             |         |             |             |         |             |             |         |             |             |
| CMIP5                                                | 37.1    | 44.7-27.7   | 49.8-24.5   | 42.2    | 48.1-39.6   | 57.2-29.9   | 40.6    | 49.0-35.4   | 52.2-31.5   | 44.6    | 50.5-35.7   | 53.2-34.4   |
| SMME                                                 | 37.1    | 46.9-27.4   | 52.2-22.2   | 46.4    | 56.7-38.2   | 57.9-29.9   | 40.7    | 51.2-33.1   | 51.7-26.6   | 46.2    | 54.5-40.4   | 57.3-33.1   |
| MCPR                                                 | 39.8    | 45.9-32.2   | 50.7-27.0   | 46.9    | 53.3-38.6   | 56.2-34.5   | 44.6    | 52.0-35.1   | 57.9-29.0   | 47.0    | 54.5-37.9   | 61.9-31.9   |
| California (1981-2010 normal: 15.8 days)             |         |             |             |         |             |             |         |             |             |         |             |             |
| CMIP5                                                | 8.9     | 10.9-7.0    | 12.3-6.4    | 10.7    | 13.2-8.7    | 14.5-7.8    | 10.5    | 13.5-8.8    | 14.4-8.4    | 11.4    | 14.0-9.8    | 14.3-9.5    |
| SMME                                                 | 9.2     | 12.3-7.1    | 15.4-6.3    | 11.6    | 13.9-8.7    | 15.4-8.2    | 10.6    | 13.9-8.5    | 14.4-6.5    | 12.8    | 14.8-10.1   | 15.6-8.7    |
| MCPR                                                 | 9.2     | 11.9-7.4    | 13.8-5.9    | 11.3    | 12.8-9.6    | 14.1-8.6    | 10.9    | 12.9-9.0    | 14.4-7.6    | 12.3    | 14.4-10.3   | 15.8-8.3    |
| Southwest (1981-2010 normal: 47.4 days)              |         |             |             |         |             |             |         |             |             |         |             |             |
| CMIP5                                                | 34.4    | 37.3-31.3   | 40.2-29.1   | 39.3    | 40.8-36.2   | 43.2-34.6   | 37.7    | 41.9-34.6   | 43.5-32.5   | 40.5    | 42.7-36.5   | 43.3-35.9   |
| SMME                                                 | 34.6    | 39.2-30.7   | 41.6-27.7   | 39.8    | 41.7-37.4   | 46.4-34.7   | 37.8    | 42.0-33.8   | 43.5-32.3   | 41.3    | 42.7-36.5   | 45.0-34.6   |
| MCPR                                                 | 35.7    | 39.3-31.3   | 41.6-27.7   | 40.0    | 42.5-37.1   | 43.8-35.2   | 39.0    | 41.2-34.9   | 42.5-32.8   | 41.1    | 43.8-38.0   | 45.0-33.9   |
| Rocky Mountain States (1981-2010 normal: 133.9 days) |         |             |             |         |             |             |         |             |             |         |             |             |
| CMIP5                                                | 102.6   | 109.3-90.2  | 116.3-85.9  | 113.7   | 117.9-99.8  | 122.2-96.0  | 110.0   | 119.4-102.5 | 121.9-94.5  | 112.9   | 119.3-106.0 | 122.5-98.9  |
| SMME                                                 | 102.6   | 116.3-86.6  | 117.4-80.8  | 114.7   | 119.6-99.8  | 127.8-96.0  | 110.0   | 119.5-96.1  | 121.9-90.1  | 115.3   | 122.7-106.2 | 125.5-96.4  |
| MCPR                                                 | 105.8   | 113.7-93.4  | 116.7-82.7  | 112.8   | 119.5-105.7 | 122.1-101.6 | 111.8   | 118.1-101.8 | 122.1-97.0  | 115.6   | 121.6-108.4 | 123.5-99.8  |
| Alaska (1981-2010 normal: 187.7 days)                |         |             |             |         |             |             |         |             |             |         |             |             |
| CMIP5                                                | 150.0   | 161.2-140.8 | 165.8-135.8 | 163.9   | 167.3-157.3 | 178.6-149.0 | 157.6   | 166.3-147.2 | 171.7-144.8 | 160.4   | 171.5-151.9 | 179.3-151.1 |
| SMME                                                 | 150.0   | 161.2-140.7 | 166.1-135.6 | 164.2   | 170.9-157.3 | 178.6-149.0 | 158.1   | 171.1-146.7 | 173.1-144.2 | 164.2   | 171.5-155.3 | 179.5-151.1 |
| MCPR                                                 | 155.0   | 164.1-141.0 | 169.7-127.3 | 165.0   | 174.9-157.5 | 180.0-152.2 | 160.9   | 171.3-148.6 | 180.3-137.6 | 166.7   | 176.3-153.9 | 181.4-148.1 |
| Hawaii (1981-2010 normal: 0.0 days)                  |         |             |             |         |             |             |         |             |             |         |             |             |
| CMIP5                                                | 0.0     | 0.0-0.0     | 0.0-0.0     | 0.0     | 0.0-0.0     | 0.0-0.0     | 0.0     | 0.0-0.0     | 0.0-0.0     | 0.0     | 0.0-0.0     | 0.0-0.0     |
| SMME                                                 | 0.0     | 0.0-0.0     | 0.0-0.0     | 0.0     | 0.0-0.0     | 0.0-0.0     | 0.0     | 0.0-0.0     | 0.0-0.0     | 0.0     | 0.0-0.0     | 0.0-0.0     |
| MCPR                                                 | 0.0     | 0.0-0.0     | 0.0-0.0     | 0.0     | 0.0-0.0     | 0.0-0.0     | 0.0     | 0.0-0.0     | 0.0-0.0     | 0.0     | 0.0-0.0     | 0.0-0.0     |

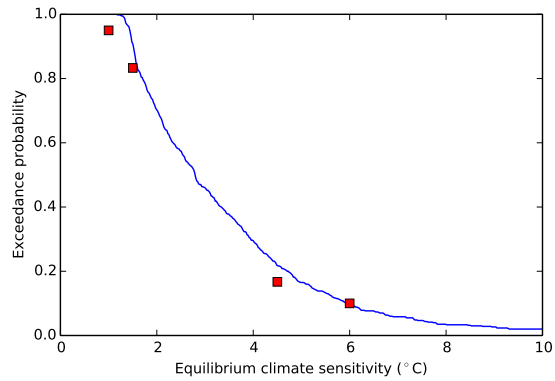

FIG. A1. Survival function of climate sensitivities from MAGICC. Red squares indicate the statements made by AR5.

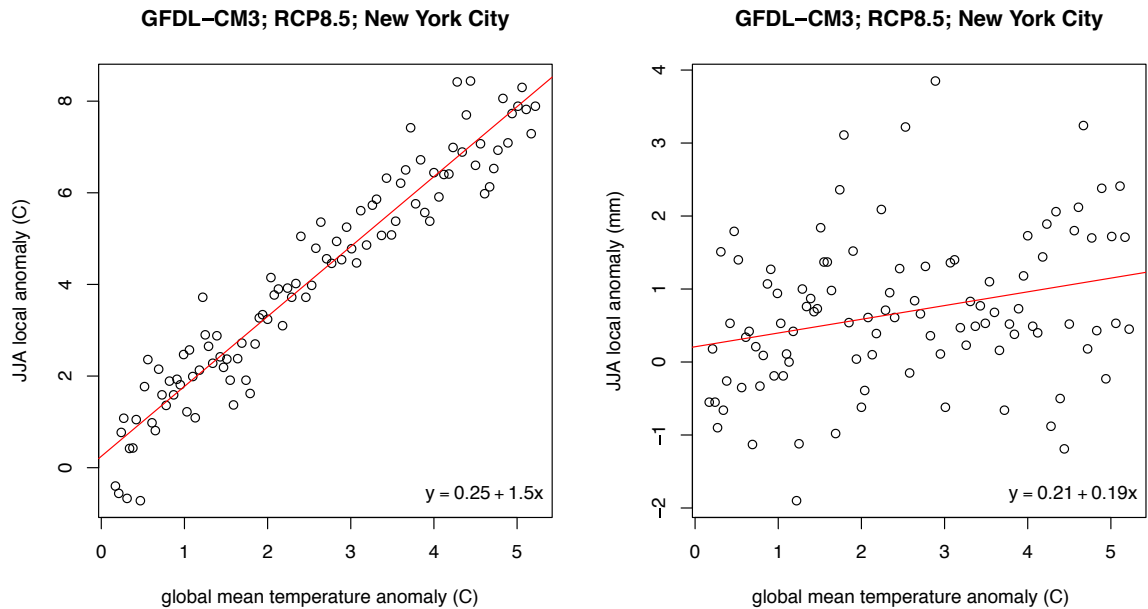

FIG. A2. Left: Local June-July-August temperature anomaly from the GFDL-CM3 grid cell containing New York City, versus global mean temperature anomaly (RCP 8.5). Right: as for Left, but for daily precipitation rate (mm/day). Best-fit regression lines are shown in red.

TABLE A23. Projected regional JJA precipitation change (%) under all RCPs for 2080-2099

| JJA<br>2080-2099                                 | RCP 8.5 |            |             | RCP 6.0 |            |            | RCP 4.5 |            |             | RCP 2.6 |            |            |
|--------------------------------------------------|---------|------------|-------------|---------|------------|------------|---------|------------|-------------|---------|------------|------------|
|                                                  | 50      | 17-83      | 5-95        | 50      | 17-83      | 5-95       | 50      | 17-83      | 5-95        | 50      | 17-83      | 5-95       |
| CONUS (1981-2010 normal: 212.5mm)                |         |            |             |         |            |            |         |            |             |         |            |            |
| CMIP5                                            | -0.3    | -13.4-5.4  | -22.1-9.9   | -1.3    | -6.9-3.2   | -16.0-19.1 | 0.6     | -4.9-6.6   | -12.3-14.4  | 2.6     | -3.5-10.0  | -4.4-11.6  |
| SMME                                             | -0.3    | -8.3-3.3   | -17.2-9.9   | -0.4    | -2.9-1.4   | -9.2-17.1  | -0.1    | -3.4-4.6   | -8.3-8.3    | 2.4     | -0.1-7.7   | -4.4-11.6  |
| MCPR                                             | 0.2     | -12.1-7.8  | -21.1-12.4  | -2.5    | -8.0-4.3   | -13.3-16.6 | 1.9     | -4.1-8.1   | -10.8-13.0  | 1.8     | -3.4-6.4   | -12.3-8.6  |
| Northeast (1981-2010 normal: 309.5mm)            |         |            |             |         |            |            |         |            |             |         |            |            |
| CMIP5                                            | 2.3     | -4.7-18.7  | -6.8-26.2   | 2.5     | -1.7-14.4  | -6.5-22.2  | 4.8     | -1.8-13.0  | -5.8-23.2   | 6.3     | -0.5-11.2  | -2.4-15.7  |
| SMME                                             | 0.3     | -2.1-12.3  | -5.8-26.2   | 0.7     | -1.7-14.4  | -2.5-18.1  | 3.0     | -1.0-10.4  | -5.8-14.4   | 1.5     | -0.5-8.6   | -2.4-15.7  |
| MCPR                                             | 5.9     | -2.7-20.1  | -11.0-27.6  | 5.1     | -2.1-16.0  | -8.3-22.2  | 6.8     | -0.1-12.6  | -8.1-19.3   | 5.1     | -1.5-10.8  | -5.8-14.7  |
| Southeast (1981-2010 normal: 374.9mm)            |         |            |             |         |            |            |         |            |             |         |            |            |
| CMIP5                                            | 1.0     | -15.1-12.8 | -20.5-20.2  | 2.5     | -5.0-11.3  | -13.4-41.4 | 4.8     | -6.7-13.3  | -9.1-17.0   | 2.7     | -2.2-11.7  | -4.5-12.6  |
| SMME                                             | 0.3     | -11.8-12.0 | -17.2-16.1  | 2.2     | -0.5-9.0   | -10.3-23.1 | 1.7     | -5.6-9.5   | -7.2-15.5   | 0.8     | -0.1-10.4  | -4.5-12.6  |
| MCPR                                             | 4.1     | -7.5-18.8  | -23.6-28.3  | 3.6     | -5.7-15.8  | -13.2-34.0 | 4.9     | -0.1-15.6  | -8.9-22.2   | 4.7     | -2.7-10.6  | -9.5-15.8  |
| South Central (1981-2010 normal: 247.8mm)        |         |            |             |         |            |            |         |            |             |         |            |            |
| CMIP5                                            | -5.9    | -21.1-4.2  | -26.6-17.0  | -6.5    | -14.9-5.5  | -16.6-20.3 | -1.5    | -14.0-11.8 | -18.6-16.9  | -0.1    | -7.6-11.5  | -9.6-12.3  |
| SMME                                             | -0.4    | -17.6-1.0  | -22.9-7.3   | -0.8    | -14.9-5.2  | -16.5-12.2 | -0.9    | -7.5-10.4  | -18.6-13.4  | 0.1     | -7.3-11.5  | -9.6-12.3  |
| MCPR                                             | -7.8    | -21.8-5.5  | -31.0-13.9  | -4.5    | -18.1-5.3  | -22.8-17.1 | -1.2    | -16.0-13.6 | -32.3-20.7  | 0.4     | -13.3-10.9 | -20.1-16.4 |
| Upper Great Plains (1981-2010 normal: 239.2mm)   |         |            |             |         |            |            |         |            |             |         |            |            |
| CMIP5                                            | -12.1   | -23.7-0.4  | -33.5-12.0  | -6.0    | -15.8-2.2  | -20.7-18.7 | -5.1    | -15.8-4.6  | -18.9-16.3  | -0.0    | -6.0-8.1   | -12.2-10.2 |
| SMME                                             | -3.8    | -18.2-0.8  | -33.5-12.0  | -1.6    | -15.8-0.3  | -19.7-7.2  | -1.1    | -10.2-3.0  | -18.8-7.6   | 0.0     | -3.9-6.6   | -12.2-10.2 |
| MCPR                                             | -10.4   | -25.1-4.7  | -37.0-16.5  | -7.7    | -18.3-2.4  | -22.3-7.9  | -2.8    | -15.1-8.5  | -23.0-15.6  | -1.7    | -11.2-6.9  | -19.1-13.7 |
| Midwest (1981-2010 normal: 304.2mm)              |         |            |             |         |            |            |         |            |             |         |            |            |
| CMIP5                                            | -3.9    | -16.8-7.6  | -29.8-12.8  | -1.6    | -12.5-3.5  | -13.6-16.2 | 0.7     | -9.4-7.0   | -14.2-13.4  | 4.4     | -3.5-9.2   | -6.0-9.9   |
| SMME                                             | -0.2    | -10.3-5.9  | -21.4-11.8  | -0.5    | -11.9-2.5  | -13.4-14.6 | 0.2     | -6.3-5.2   | -13.8-8.4   | 1.6     | -1.2-9.0   | -6.0-9.9   |
| MCPR                                             | -2.3    | -14.9-7.5  | -21.9-14.0  | -5.3    | -13.8-4.5  | -19.2-14.2 | 0.6     | -7.2-7.5   | -17.3-13.5  | -0.8    | -6.1-7.5   | -16.8-12.0 |
| Northwest (1981-2010 normal: 72.6mm)             |         |            |             |         |            |            |         |            |             |         |            |            |
| CMIP5                                            | -19.2   | -35.4-2.0  | -51.0-27.1  | -9.5    | -20.0-1.0  | -41.1-21.9 | -5.6    | -19.2-10.4 | -37.4-24.9  | 7.7     | -11.8-16.2 | -16.9-29.7 |
| SMME                                             | -5.9    | -32.3-0.1  | -50.0-15.9  | -5.2    | -16.8-0.9  | -29.9-15.4 | -2.9    | -19.2-8.3  | -37.4-22.5  | 3.6     | -6.2-14.9  | -16.9-29.7 |
| MCPR                                             | -14.3   | -45.8-10.0 | -58.0-30.9  | -5.8    | -26.6-16.2 | -48.3-27.8 | -4.9    | -28.1-13.6 | -40.8-37.5  | -0.4    | -21.8-23.9 | -43.5-38.7 |
| California (1981-2010 normal: 16.9mm)            |         |            |             |         |            |            |         |            |             |         |            |            |
| CMIP5                                            | 5.2     | -38.0-89.7 | -53.7-198.6 | -7.2    | -25.5-30.1 | -31.9-87.5 | 1.4     | -27.3-40.3 | -37.5-71.2  | 6.0     | -9.2-51.1  | -20.5-70.5 |
| SMME                                             | -0.6    | -27.2-40.4 | -39.2-198.6 | 0.2     | -19.8-30.1 | -29.8-87.5 | 0.0     | -16.5-25.1 | -37.5-70.3  | 0.1     | -3.1-39.4  | -20.5-70.5 |
| MCPR                                             | 14.8    | -35.3-80.3 | -58.3-158.3 | 1.2     | -19.5-42.2 | -43.3-72.5 | 1.6     | -33.1-37.7 | -52.6-100.4 | 7.2     | -21.2-37.4 | -44.6-62.3 |
| Southwest (1981-2010 normal: 120.2mm)            |         |            |             |         |            |            |         |            |             |         |            |            |
| CMIP5                                            | 3.8     | -18.4-23.7 | -39.8-34.2  | 0.8     | -14.4-12.4 | -23.4-28.4 | 4.4     | -12.0-14.7 | -22.0-23.2  | -0.2    | -4.5-10.8  | -21.1-20.8 |
| SMME                                             | 1.3     | -9.3-13.7  | -26.8-30.3  | 0.8     | -14.4-6.9  | -18.9-15.9 | 1.1     | -4.9-13.9  | -17.2-19.9  | -0.4    | -8.6-8.5   | -21.1-20.8 |
| MCPR                                             | 2.8     | -18.4-23.3 | -45.4-36.2  | -5.1    | -21.5-13.9 | -28.2-25.8 | -0.1    | -19.7-15.7 | -30.5-31.1  | -3.1    | -19.6-14.6 | -32.4-24.0 |
| Rocky Mountain States (1981-2010 normal: 92.4mm) |         |            |             |         |            |            |         |            |             |         |            |            |
| CMIP5                                            | -4.0    | -19.8-15.7 | -35.9-20.9  | -1.9    | -14.4-10.3 | -32.9-14.9 | -2.5    | -10.5-12.0 | -19.8-17.1  | 4.3     | -1.8-15.1  | -12.8-20.4 |
| SMME                                             | -0.6    | -16.4-6.1  | -29.4-17.4  | 0.3     | -10.6-10.3 | -16.0-14.8 | -1.7    | -9.2-4.4   | -19.8-17.1  | 0.3     | -1.8-10.5  | -12.8-20.4 |
| MCPR                                             | -1.3    | -18.9-17.9 | -37.1-29.1  | -2.2    | -17.0-13.2 | -29.4-21.3 | -1.2    | -12.9-14.8 | -23.5-33.7  | 1.2     | -10.7-15.2 | -30.3-21.9 |
| Alaska (1981-2010 normal: 184.7mm)               |         |            |             |         |            |            |         |            |             |         |            |            |
| CMIP5                                            | 28.9    | 18.2-40.6  | 12.2-64.0   | 16.2    | 13.8-26.5  | 7.1-57.4   | 15.3    | 10.3-26.2  | -4.4-31.2   | 13.9    | 5.8-17.8   | 3.3-27.4   |
| SMME                                             | 22.1    | 1.9-38.0   | 0.5-57.0    | 14.9    | 1.3-25.1   | 0.1-29.4   | 14.1    | 1.1-21.2   | 0.4-30.2    | 8.4     | 0.8-15.4   | 0.3-27.4   |
| MCPR                                             | 25.2    | 17.3-44.3  | 5.2-76.2    | 15.6    | 9.8-25.1   | 7.0-42.1   | 14.4    | 7.5-27.2   | 2.3-35.6    | 11.2    | 3.7-19.6   | -2.1-25.4  |
| Hawaii (1981-2010 normal: 472.8mm)               |         |            |             |         |            |            |         |            |             |         |            |            |
| CMIP5                                            | -3.6    | -15.2-22.3 | -37.6-49.0  | -0.1    | -9.9-8.4   | -32.0-49.3 | -0.4    | -13.1-17.7 | -23.7-26.8  | 5.8     | -7.1-14.5  | -14.1-25.5 |
| SMME                                             | -0.5    | -12.8-17.4 | -37.6-45.5  | -0.4    | -9.9-4.2   | -32.0-14.6 | 0.1     | -8.7-9.6   | -20.8-23.6  | 4.8     | -0.2-12.9  | -14.1-25.5 |
| MCPR                                             | 0.7     | -17.2-22.5 | -35.9-41.2  | 0.5     | -11.4-9.1  | -25.5-15.6 | -3.0    | -13.6-13.8 | -23.6-22.9  | 4.1     | -7.7-16.7  | -16.6-24.0 |

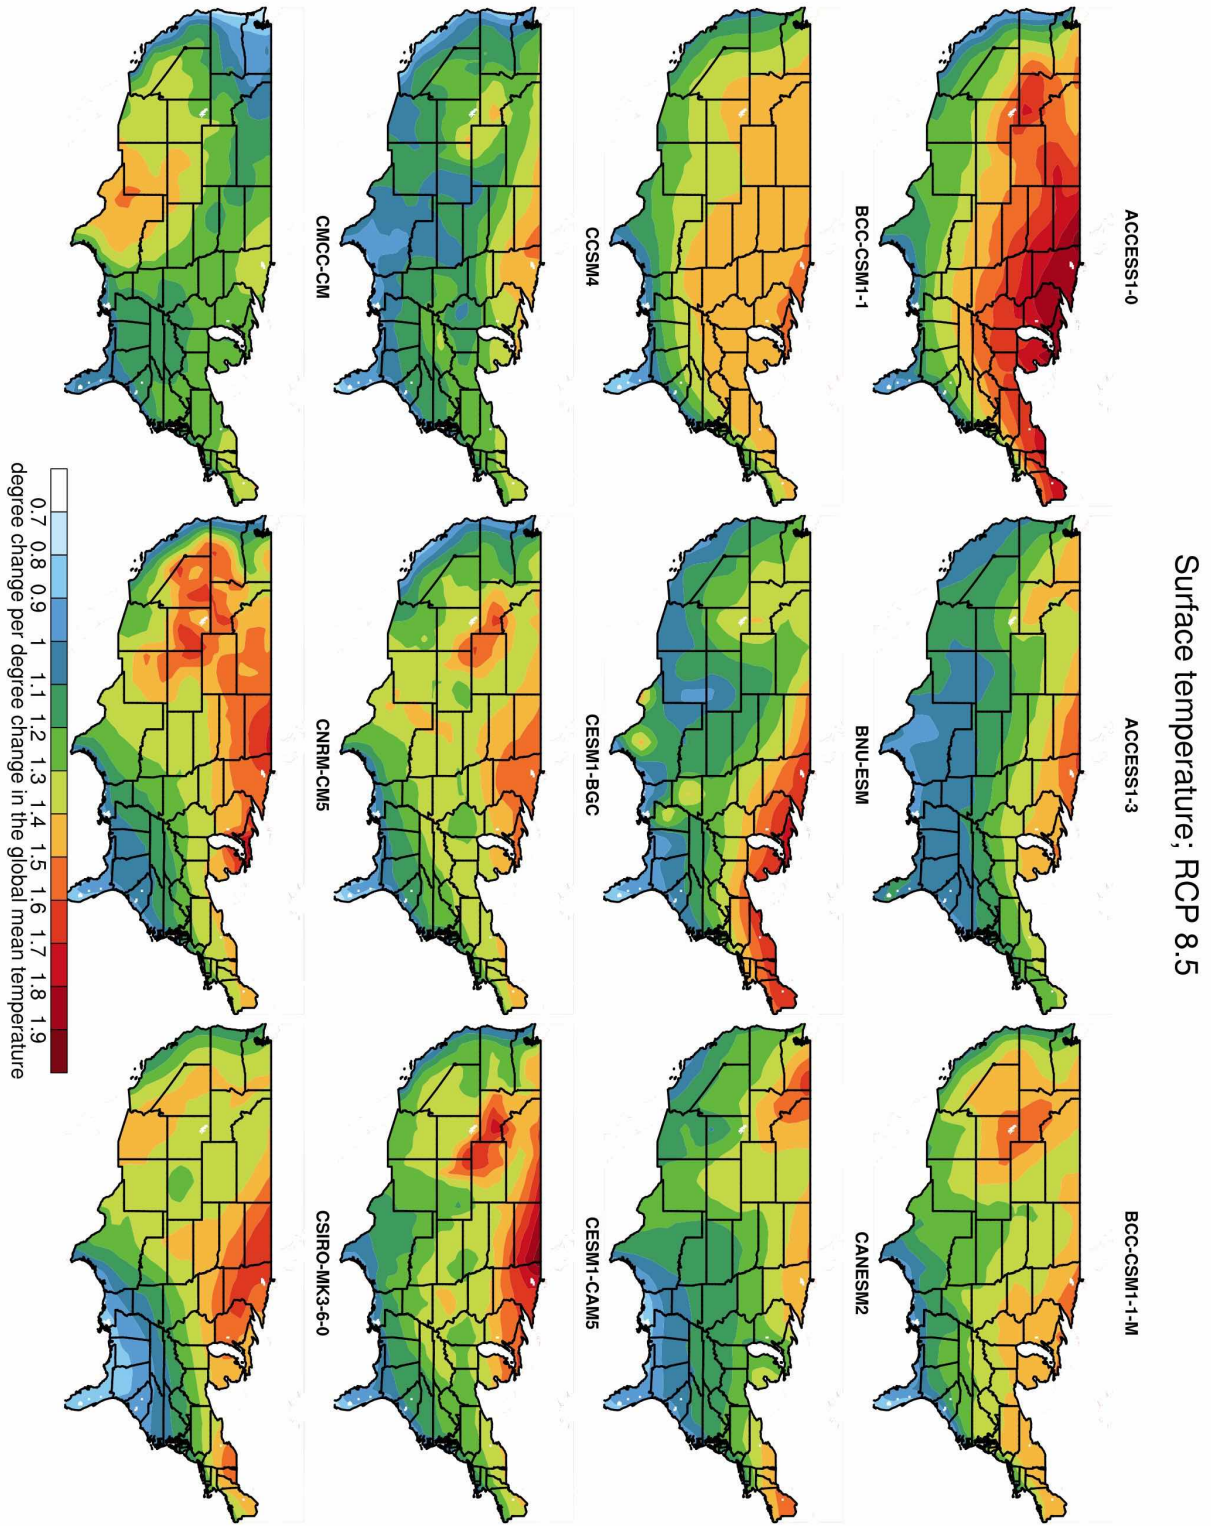

FIG. A3. Annual surface temperature patterns for each CMIP5 model for RCP 8.5.

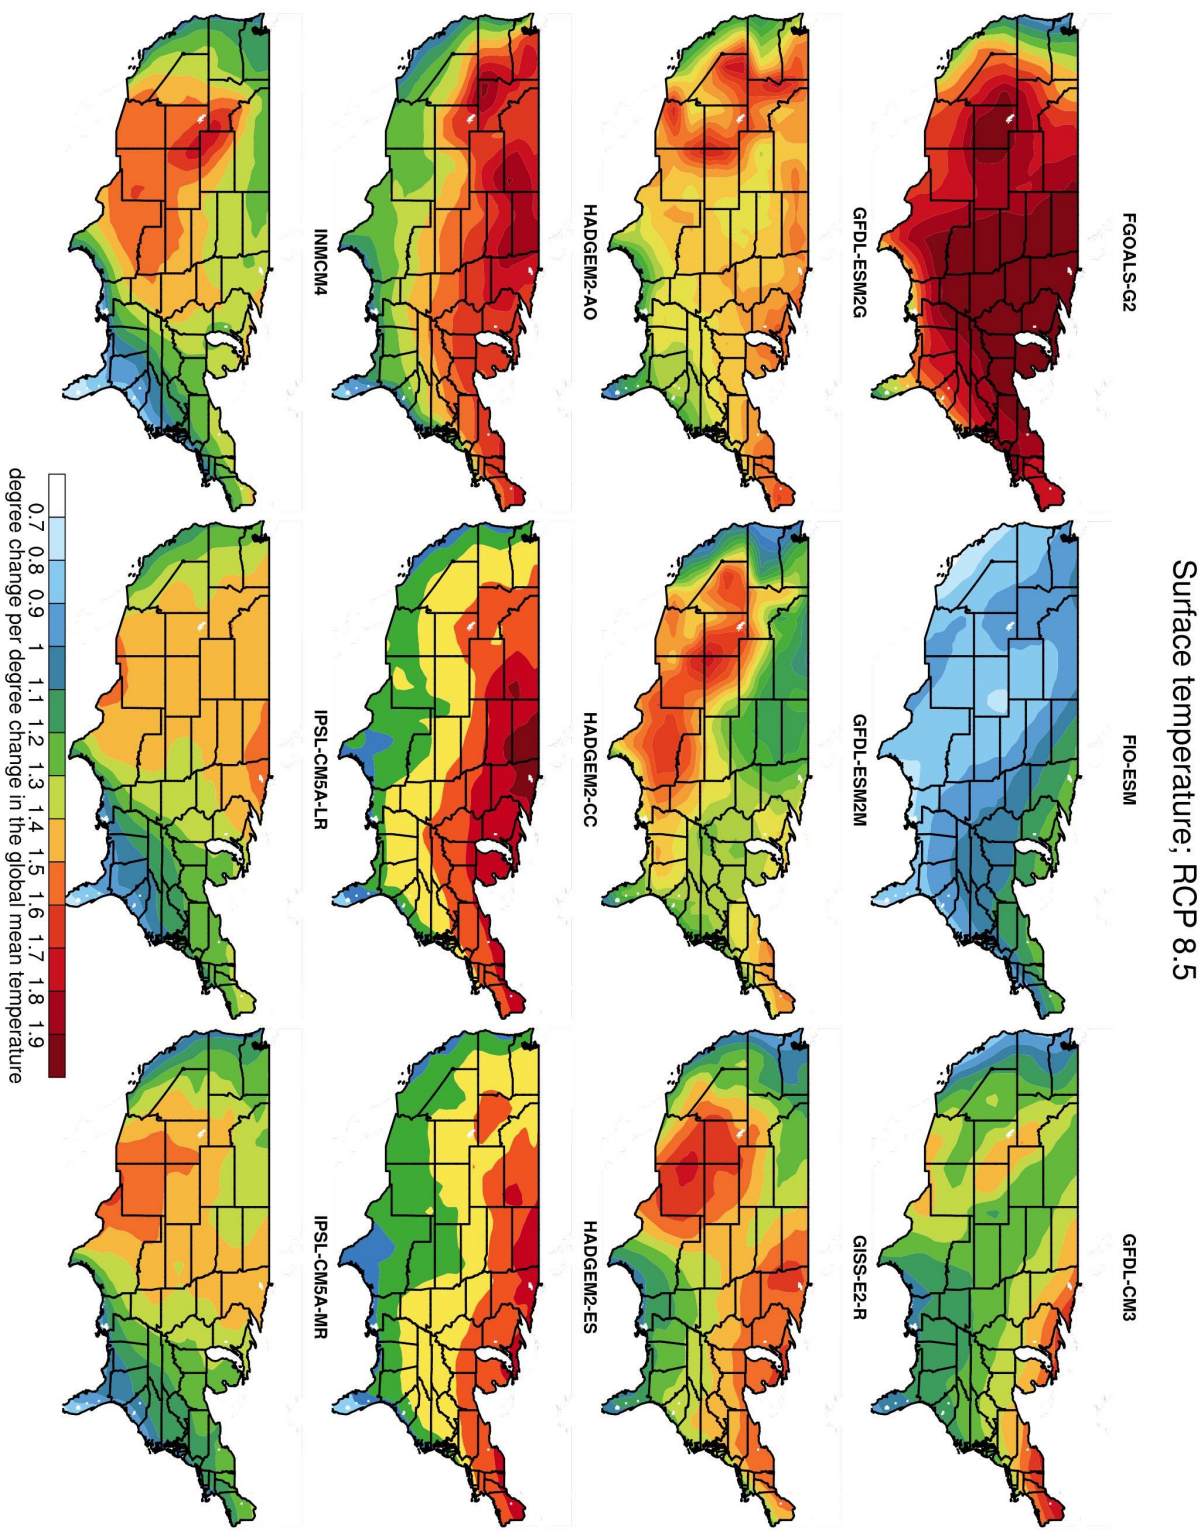

FIG. A3. (con't)

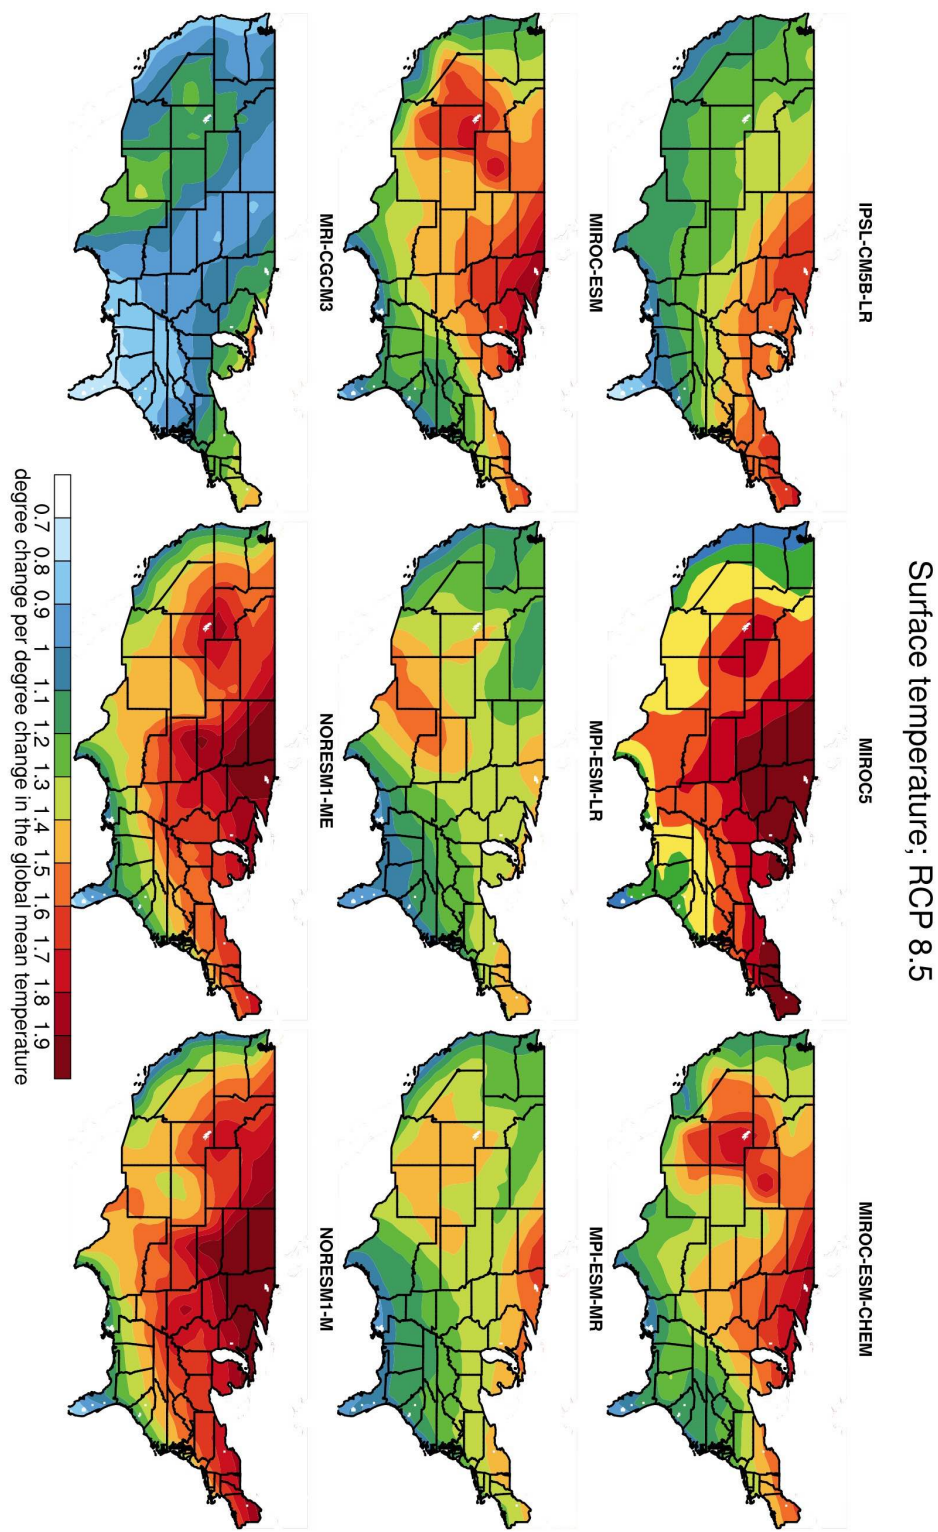

FIG. A3. (con't)

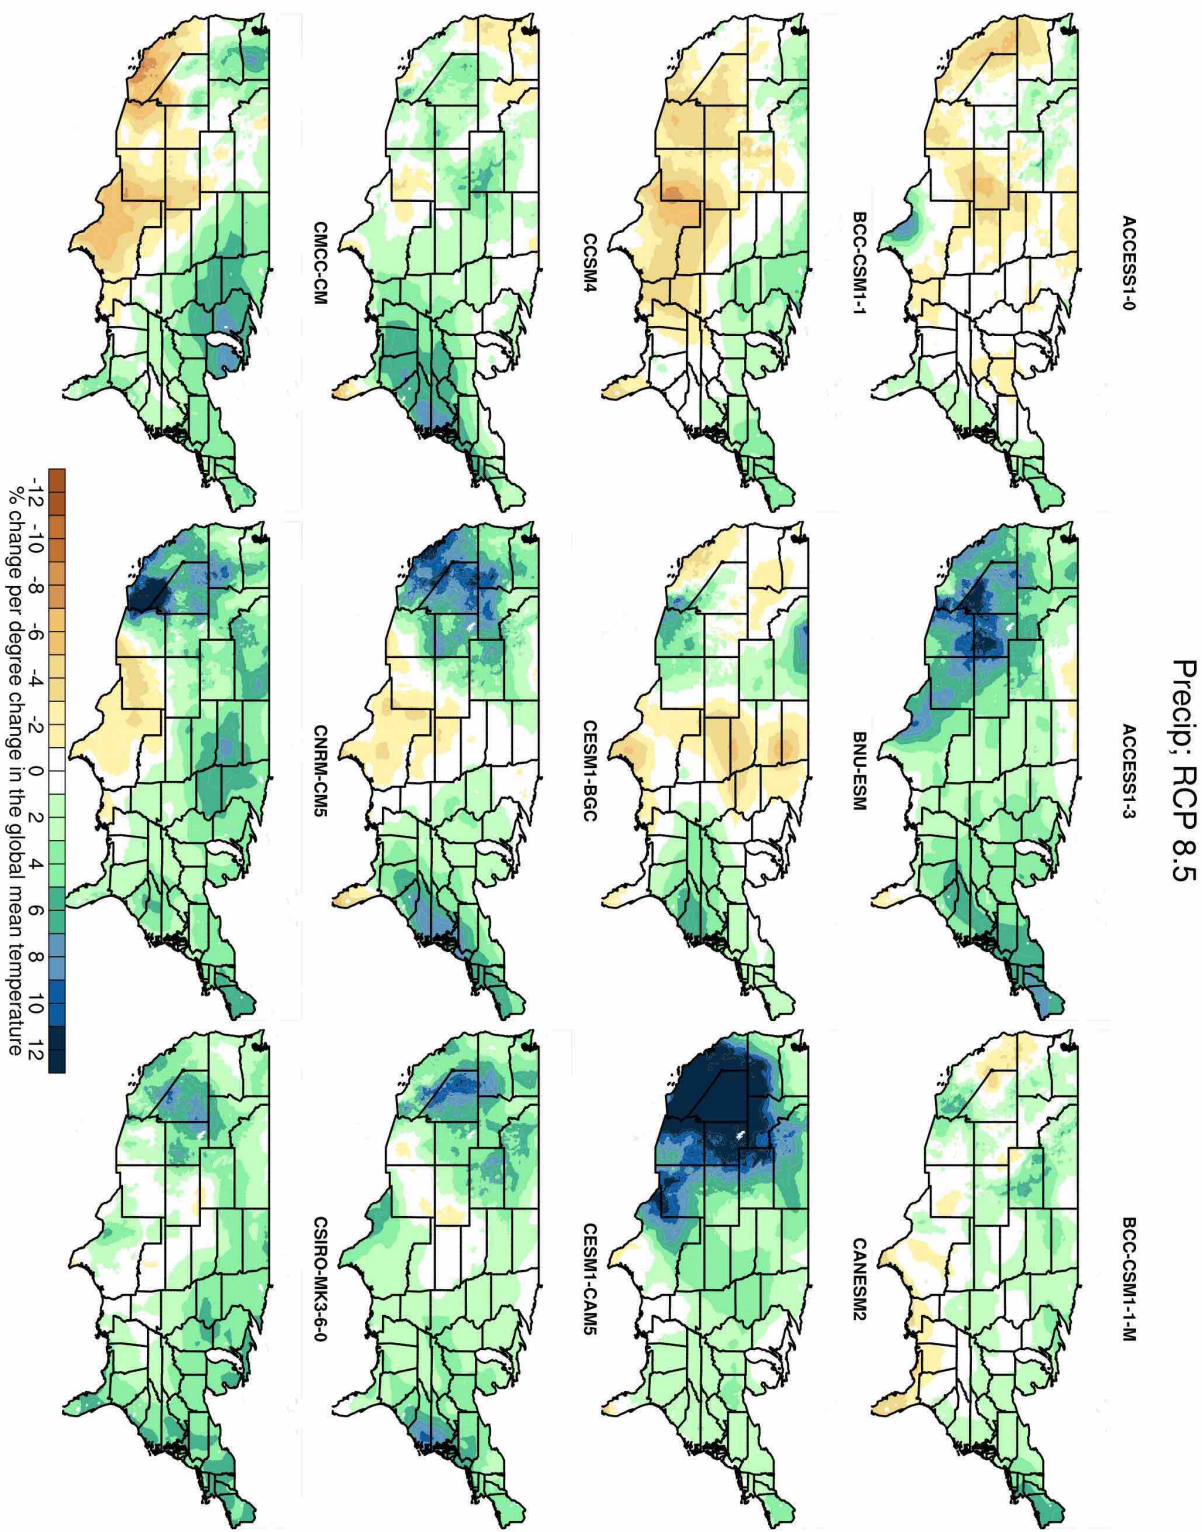

FIG. A4. Annual precipitation patterns for each CMIP5 model for RCP 8.5.

# Precip; RCP 8.5

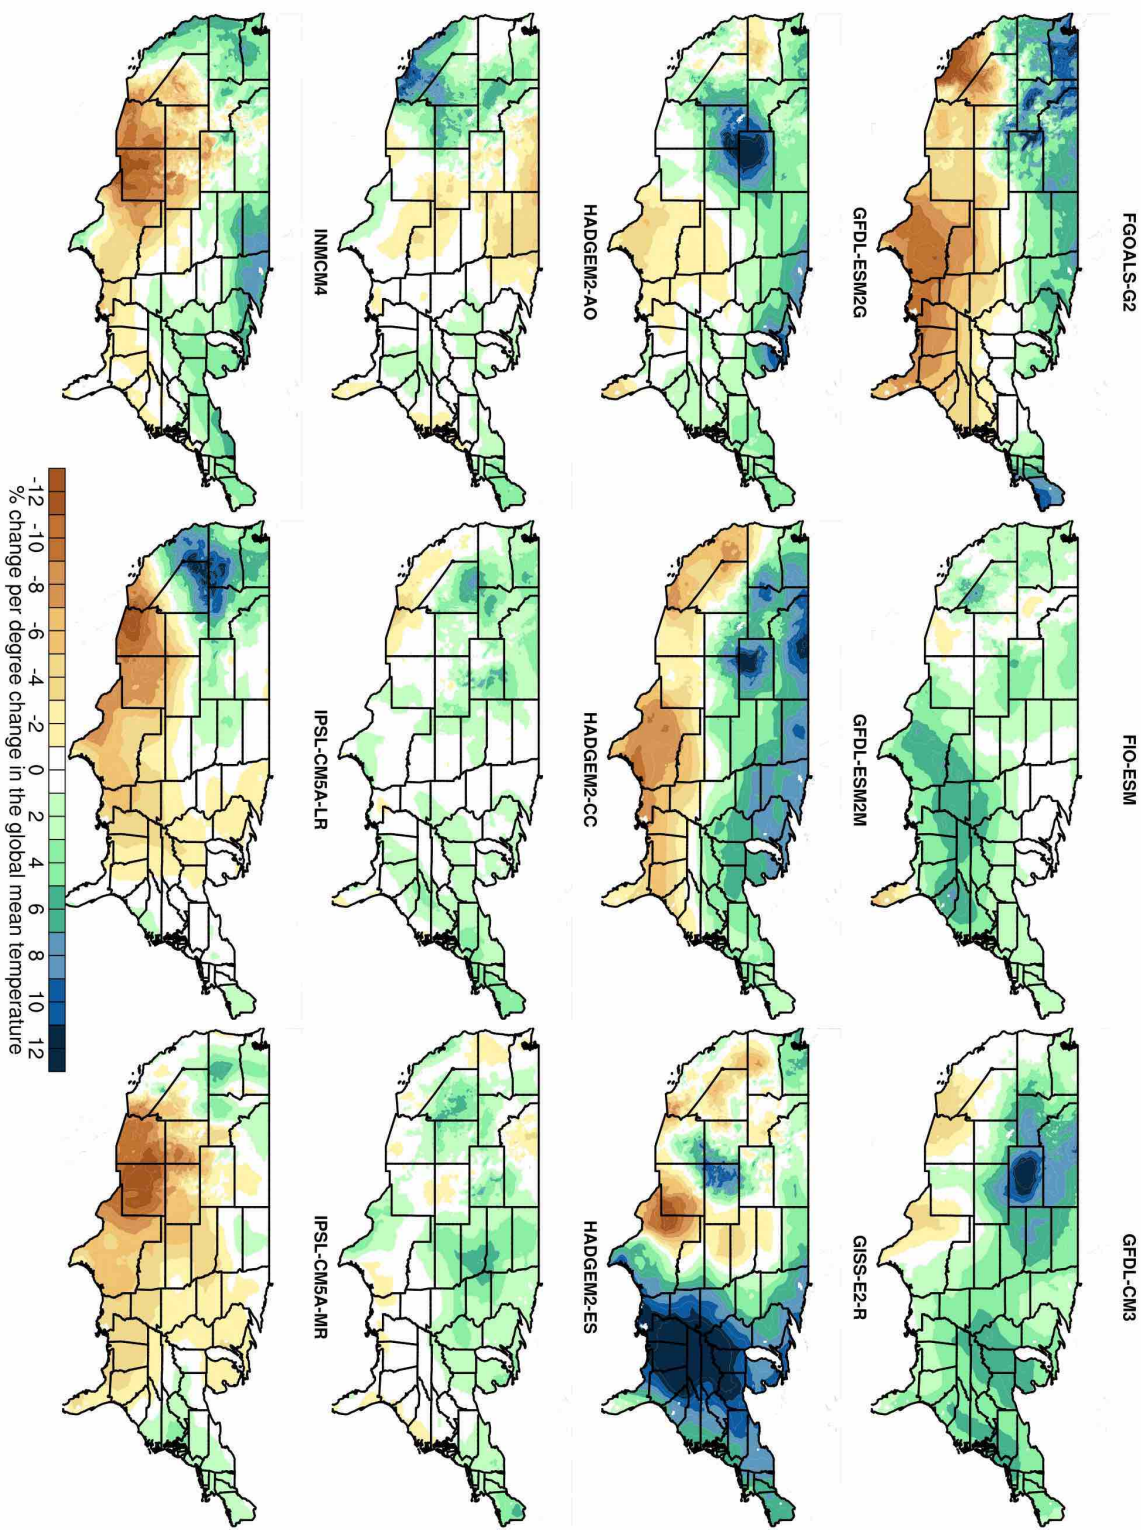

FIG. A4. (con't)

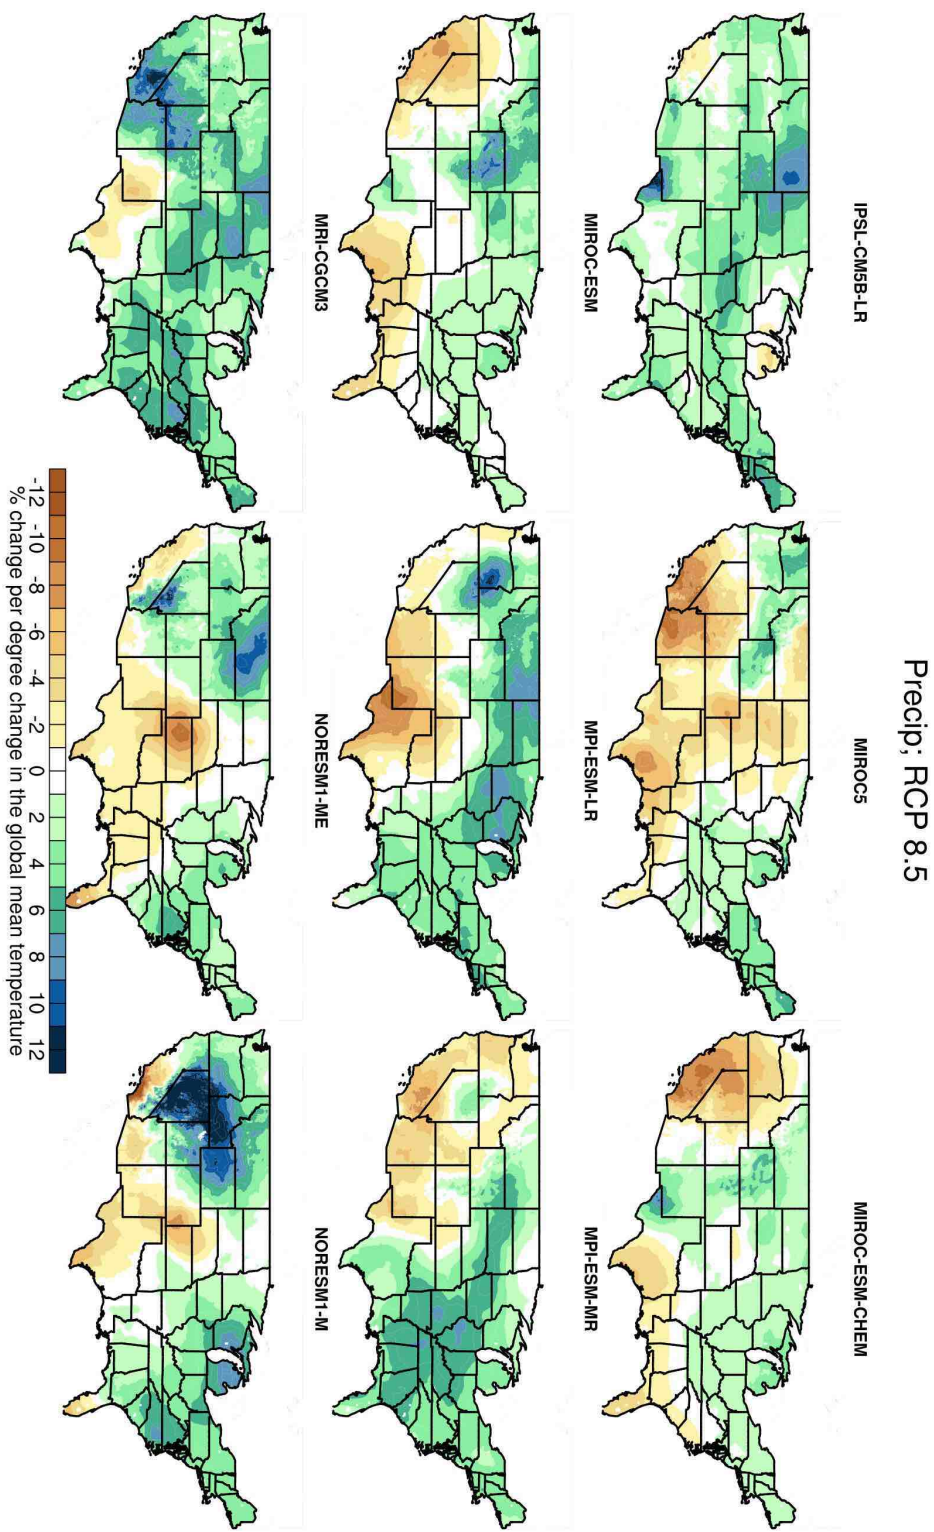

FIG. A4. (con't)

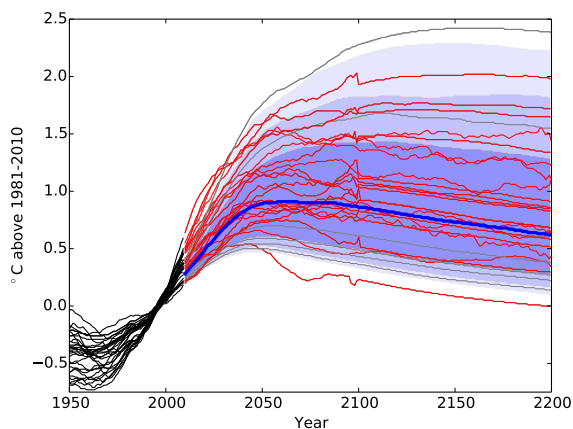

FIG. A5. As for Fig. 2, but for RCP 2.6.

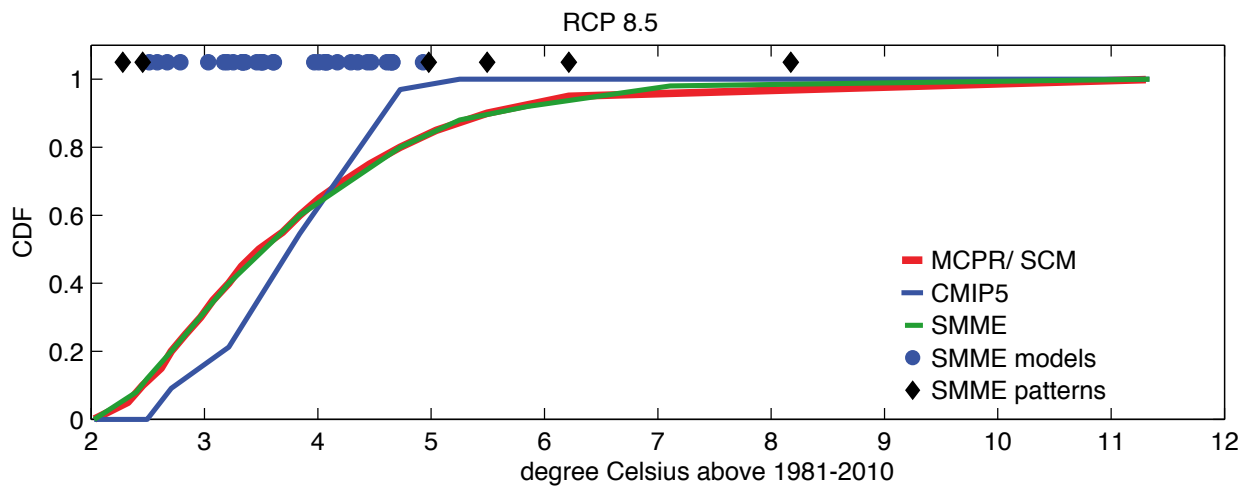

FIG. A6. The cumulative distribution function of 2080–2099 global mean temperature anomalies (relative to the 1981–2010 normal) for RCP 8.5. Blue curve = CMIP5 model output CDF; red curve = MCPR/SCM projection; green curve = SMME projection. Blue dots/black diamonds indicate the models/surrogates weighted in the SMME projection.

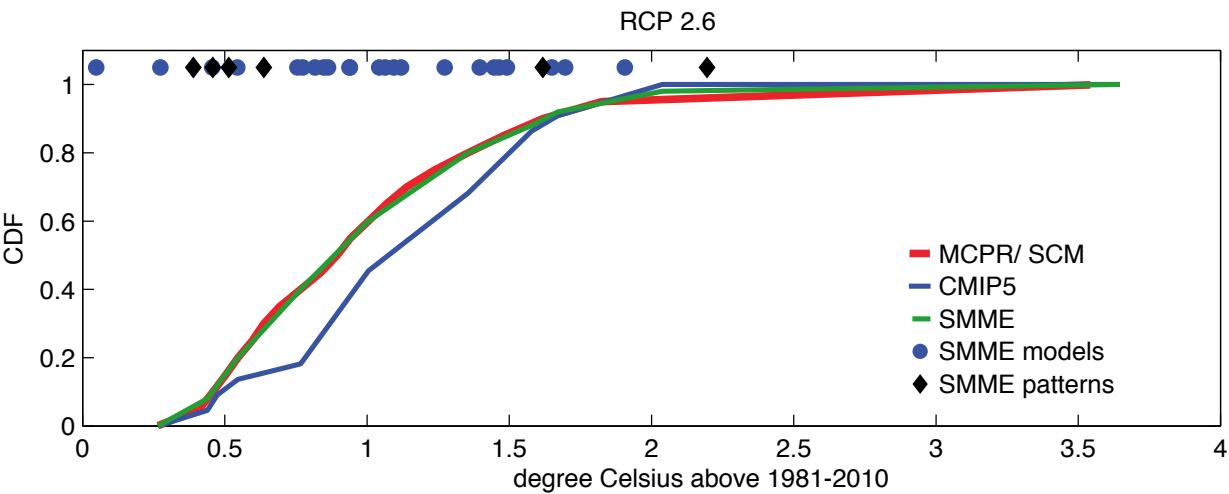

FIG. A7. As for Fig. A6, but for RCP 2.6.

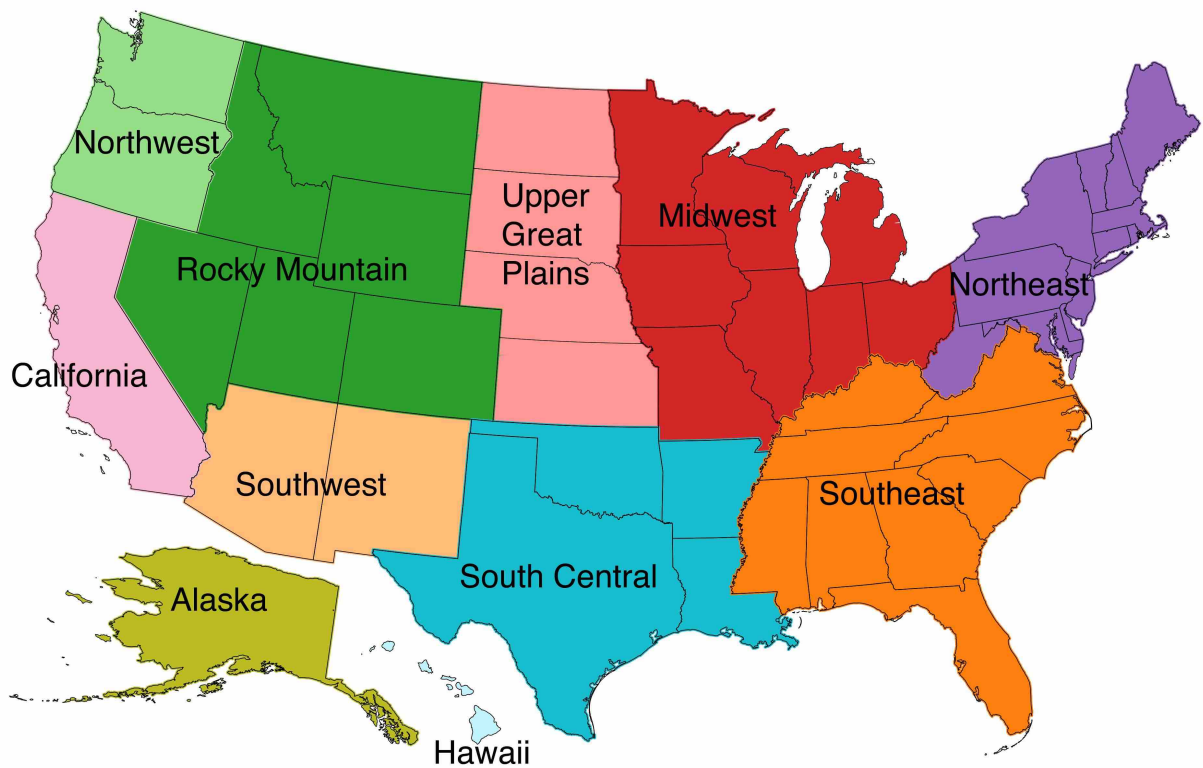

FIG. A8. State clusters for regional climate results aggregation.

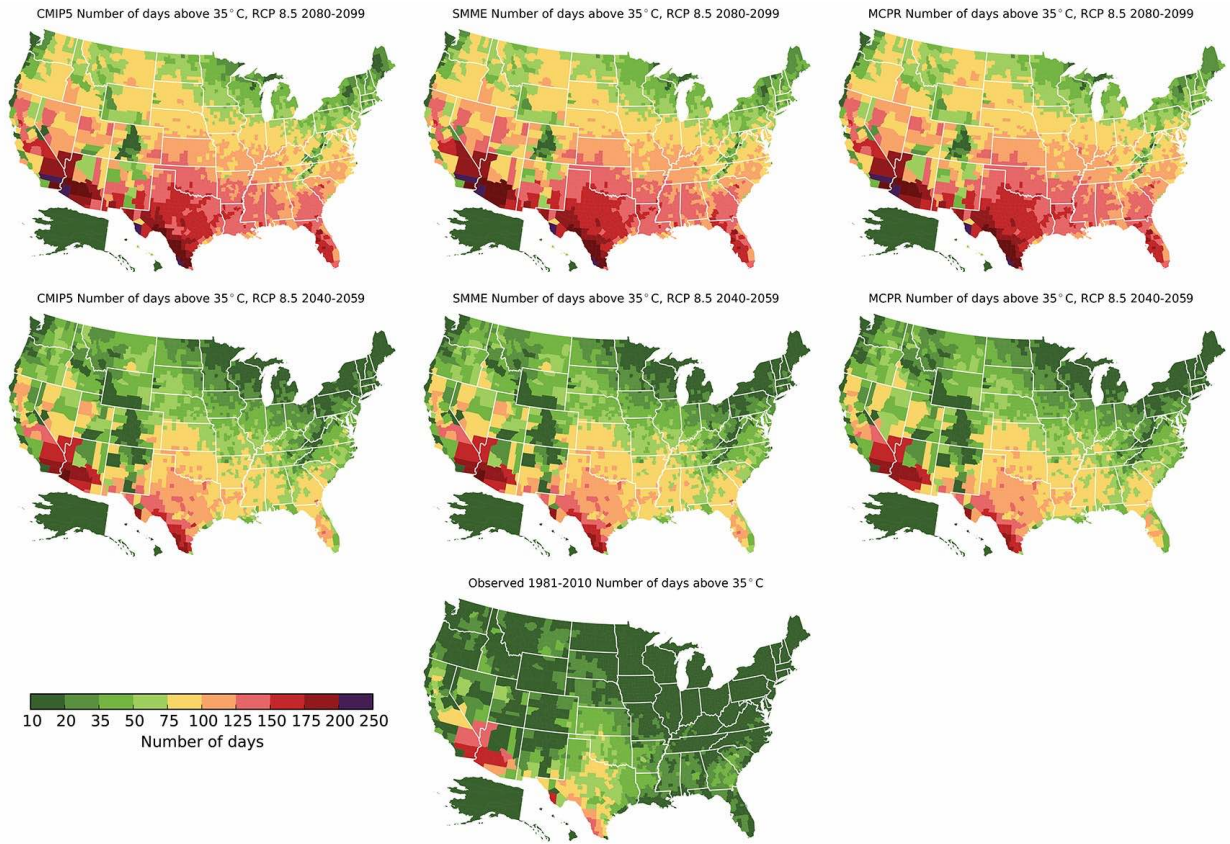

FIG. A9. Expected number of days (i.e., averaged across years and states of the world) with maximum temperature above 35°C under RCP 8.5 for 2040–2059 and 2080–2099. Bottom row is the 1981–2010 normal.

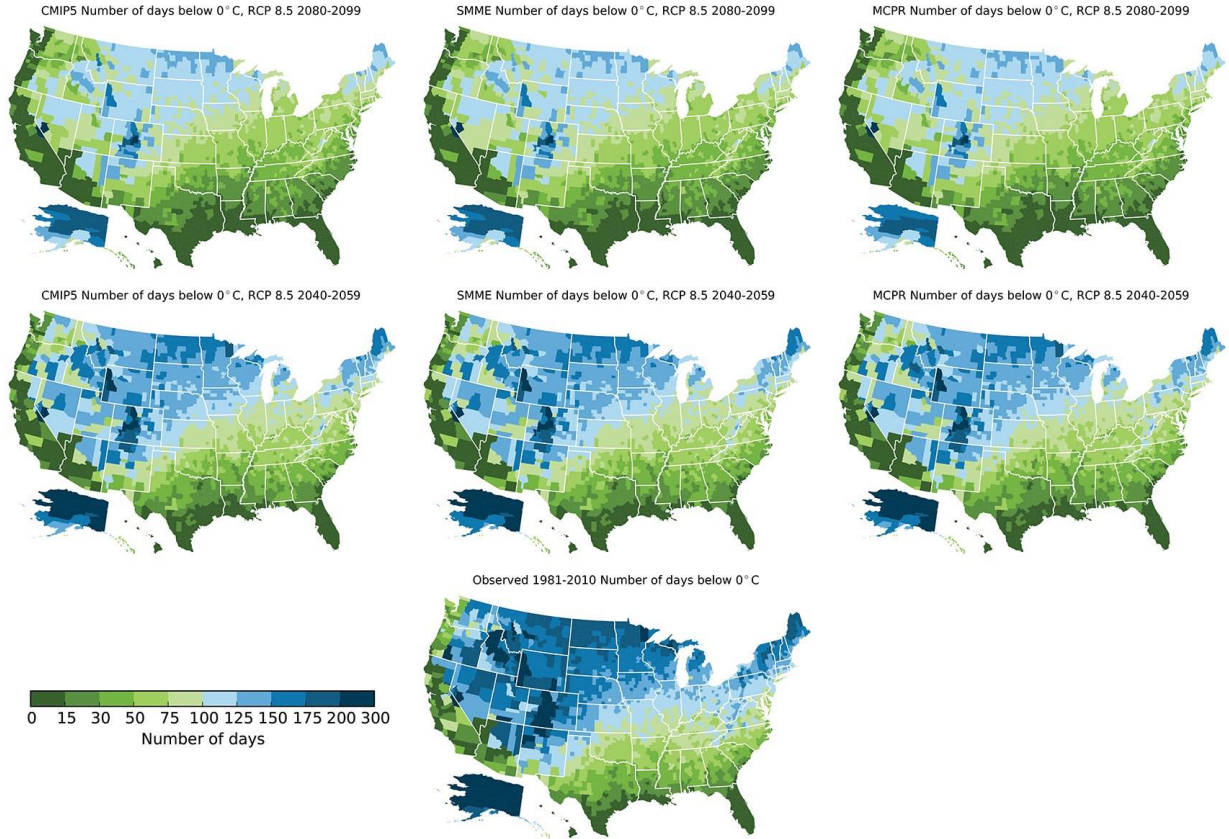

FIG. A10. Expected number of days (i.e., averaged across years and states of the world) with minimum temperature below 0°C under RCP 8.5 for 2040–2059 and 2080–2099. Bottom row is the 1981–2010 normal.

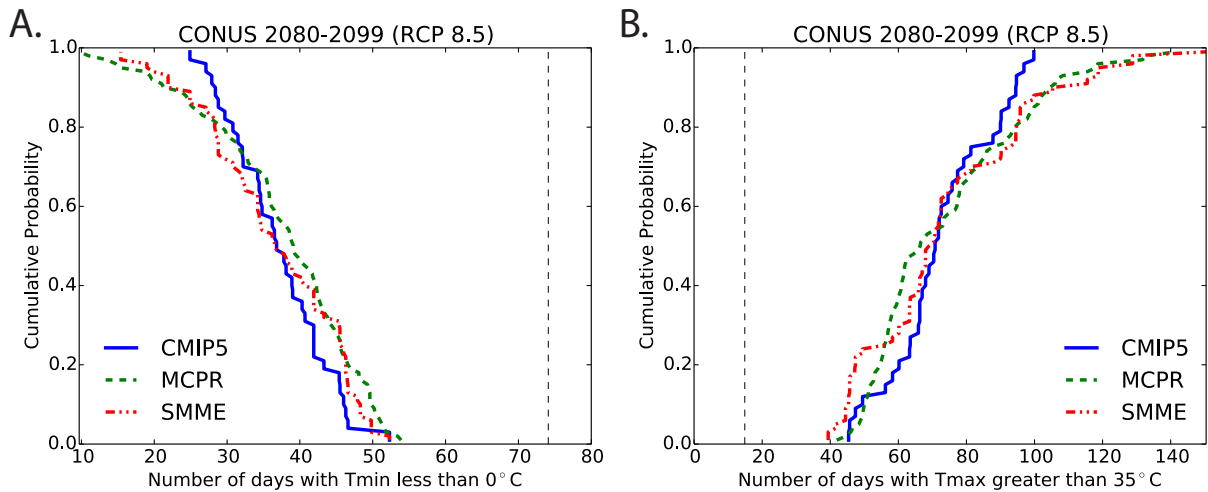

FIG. A11. (A) Survival function of number of days with minimum temperature below 0°C (population-weighted using county population) and (B) cumulative probability of number of days with maximum temperature above 35°C (population-weighted using county population) under RCP 8.5 for 2080–2099 for the contiguous U.S. Vertical dashed lines indicate the 1981–2010 normal.

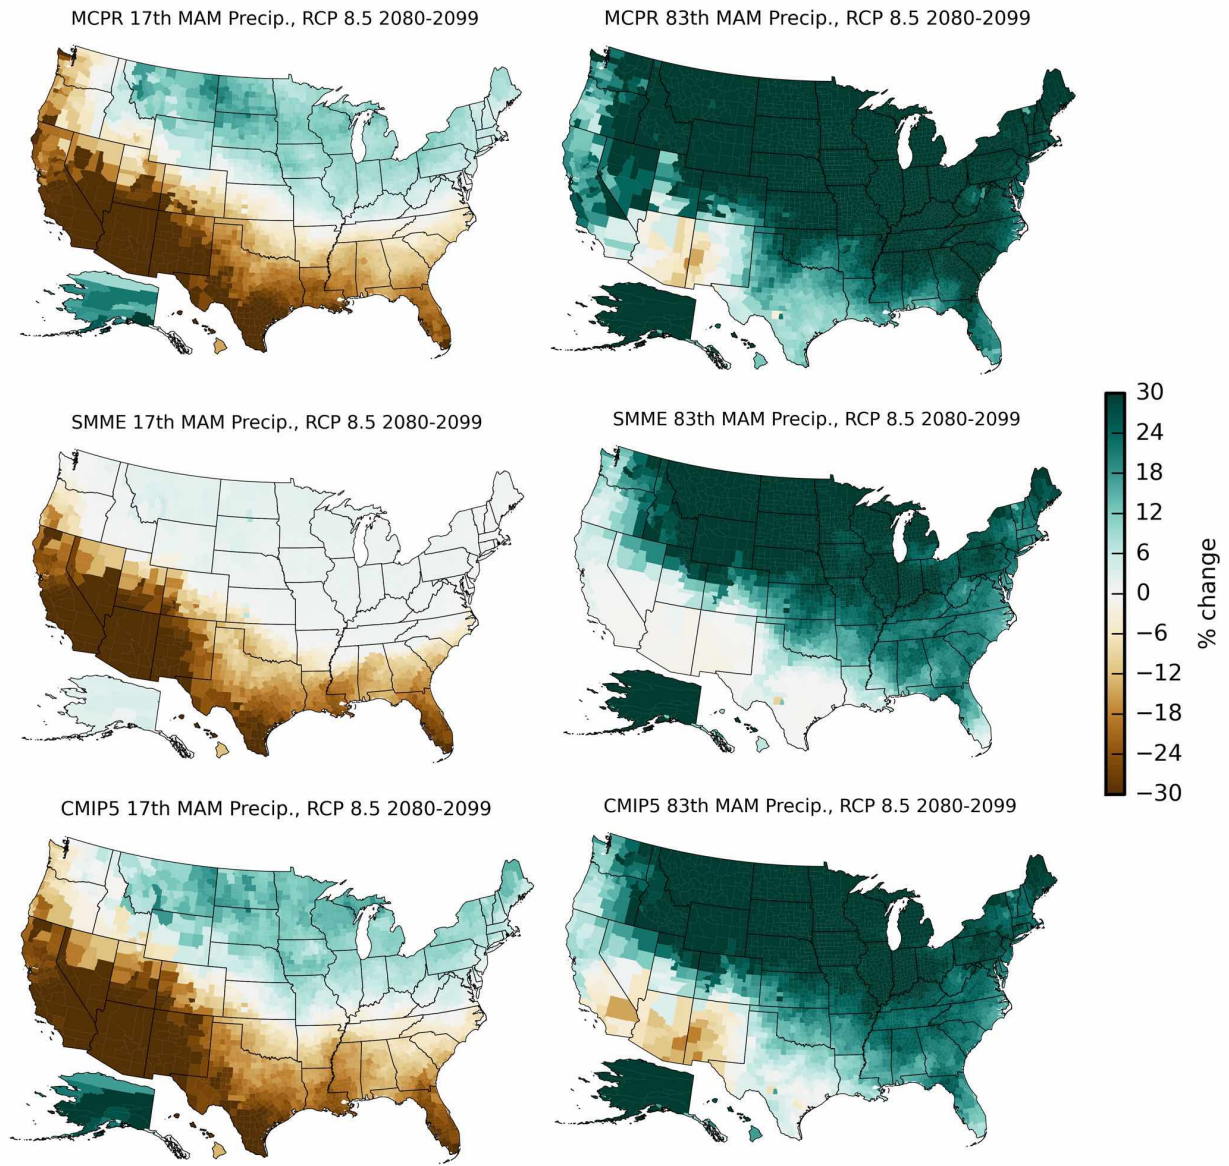

FIG. A12. Percentage change (left column: 17th percentile; right column: 83rd percentile) in average spring precipitation from MCPR (top row), SMME (middle row), and CMIP5 (bottom row) under RCP 8.5.

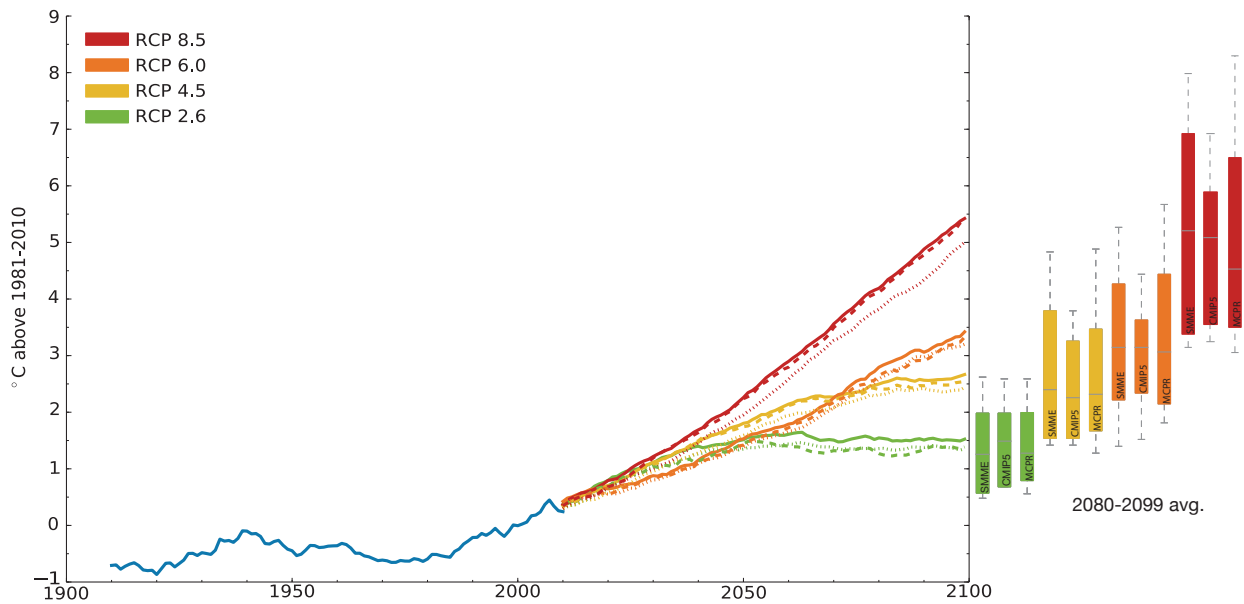

FIG. A13. (Left) Projected median CONUS average annual temperature anomaly (10-yr running average, relative to 1981–2010) from the unweighted CMIP5 ensemble (solid), SMME (dashed), and MCPR (dotted). Blue: historical observations from the National U.S. Historical Climatology Network (USHCN); red: RCP 8.5; orange: RCP 6.0; yellow: RCP 4.5; green: RCP 2.6. (Right) 2080–2099 CONUS temperature anomaly, relative to 1981–2010. red: RCP 8.5; orange: RCP 6.0; yellow: RCP 4.5; green: RCP 2.6. Whiskers are 5th/95th, boxes are 17th/50th/83rd.
